# Supplementary material for: Technical Design Report for the LUXE Experiment
Source: arXiv:2308.00515 source file (2023-08-02)
Supplement: Supplementary file 1 [file appendix_PerSystemOrganisation.tex]

\section{Laser \& Diagnostics}
The related costs, manpower and timelines are discussed in detail. The timeline for laser sub-project are largely independent of the \euxfel shutdown schedule. Preparatory work can be conducted at available lasers (Jena or Tel Aviv) and once the clean-room is ready for installation in the clean room. 

The laser installation schedule intercepts with the \euxfel schedule only for the installation of the IP chamber (which is part of the electron beamline in the \euxfel tunnel XS1) and the laser beamline components in XS1. The latter does not require a long shutdown for installation (discussed in Chapter 12) while the IP chamber interior components are modular and can be pre-aligned and installed at short notice. 

There are two distinct scenarios with regards to the installation of the laser. The first is the locating the laser in level -2 above the \euxfel tunnel (considered in the CDR). This could still  be a viable option, but for reasons detailed in Chapter 12 the currently preferred option is a clean room constructed at ground level. This option is visible in the timelines. We note that changing the location does not have a major impact on the laser installation schedule.

The activities regarding the construction of the laser and beamline are distributed across four collaborating institutes: Deutsches Elektronen Synchrotron (DESY), Friederich-Schiller University Jena and Helmholtz Institute  Jena, The Queen's University of Belfast and Tel Aviv University of Israel. Jena will co-ordinate the implementation of the laser system.

\subsection{Human and financial resources}

Below we detail the resources required for the implementation of the preferred option of integrating a new 350 TW laser system into LUXE.
The activities can be split into 5 major areas of investment:

\begin{itemize}
    \item Laser
    \item Laser automation
    \item Diagnostics
    \item Laser Beamline
    \item Tunnel Diagnostics
    
\end{itemize}

Resources for the vacuum components and beamlines directly associated with the laser (compressor, diagnostics chamber) are included in the laser budget while vacuum pumps for the electron beamline and the integration of the laser diagnostics into the DAQ system are considered within the context of the Technical Coordination and DAQ TDR chapters respectively .

\subsubsection{Financial Resources} 
The net investment cost as per quotations and estimates is listed below and summarised in Table \ref{tab:cost}. We note that these costs are currently subject to inflationary pressures.

\begin{itemize}
    \item \textbf{Laser system }\\
This cost is based on a quotation from Thales  as shown in table \ref{tab:cost}. The estimate comprises oscillator, amplifier and compressor+ chamber. A staged implementation would split the capital costs over the course of the project with with phase-0 delaying the cost of the  \euro1700k amplifier to a later stage in the project. Common components of phase-0 with phase-1 such as beamline and compressor will be built to be compatible with both implementation stages.

A detailed breakdown is shown in Table~\ref{tab:New_laser_system_cost} and Table~\ref{tab:Jeti40_laser_system_cost} in the appendix.

\item \textbf{Laser automation: \euro250k}\\
Automation of key alignment procedures in the laser will allow the stable operation for extended periods without manual intervention. 

\begin{table}[]
    \centering
    \caption{Cost estimates for the laser project (in k\euro). }
    %\begin{tabular}{l|r|l}
    \begin{tabular}{|p{4cm}|p{2cm}|p{6cm}|}
         \hline
         350 TW Laser Amplifier System  & 3685 & quote  \\\hline
         Oscillator  & 160 & quote  \\\hline
         Timing  & 80 & quote  \\\hline
         Compressor  & 250 & quote  \\\hline
         Automation & 250 & based on JETI200 components\\\hline
         Laser  diagnostics & 310 & quote + based on JETI200\\\hline
         Beamline & 400 & quote +  based on experience\\\hline
         Vacuum chamber & 95 & quote + based on experience \\\hline
         Tunnel diagnostics & 115 & quote +  based on experience\\\hline

        \textbf{Total sum} & \textbf{5345} & Total expenditure
         \\\hline
    \end{tabular}
    \label{tab:cost}
\end{table}

\item \textbf{Laser diagnostics: \euro310k }\\
The costings for laser area diagnostics includes the purchase of all the laser characterisation devices, optics, cameras, mounts, vacuum chamber for the diagnostics and required vacuum pump. Detailed cost breakdown by item  is given in Appendix in  Table~\ref{tab:laser_area_diag_cost}. 
 
\item \textbf{Transport beamline cost: \euro400k}\\
The cost of the laser transport line includes cost of mirror mounts, mirrors and other items required for steering the optics and monitoring.  A detailed cost breakdown is given in the appendix in  Table~\ref{tab:laser_beamline_cost}.

\item \textbf{IP chamber: \euro95k}\\
The IP chamber cost includes the actual IP chamber and the optical table beneath the IP chamber. As the IP chamber is integrated in the LUXE particle beam line cost relating to vacuum pumps, gate valves and control system are included in infrastructure section.

\item \textbf{Tunnel diagnostics:\euro115}\\
The tunnel diagnostics consist of an imaging system for the IP and the optomechnical components for the diagnostics and timing diagnostic. 
\end{itemize}

A detailed budget breakdown can be found in the appendix.

\subsubsection{Human Resources} 

During the life time of the project 2 physicists and 0.5 technicians are required on a permanent basis for the operation of the laser and diagnostics. During the early phase of the project they are responsible for planning, purchasing and development. In particular the tunnel and laser diagnostics can be fully implemented and tested with final installation as soon as the infrastructure at Osdorfer Born is ready.
 They will coordinate with the laser manufacturer during manufacture  and supervise the acceptance procedures and installation.

Additional effort is required during installation to implement laser safety interlock system and integrate it into Osdorfer Born. Support for installation and commissioning of services (electrical/water) and vacuum systems by the respective  technical groups at DESY/XFEL.

\textbf{Additional  personnel for installation}\\
 The disassembly at the factory and installation of the laser will be performed by the laser company. During the installation the LUXE laser team will be present full time and learn the operation of the system.
 
 Additional technical staff is required for the installation of the laser beamline and services. This is estimated at 1.5 FTE (3  technicians for 6 months)

%\begin{table}[]
    %\centering
   % \caption{Cost estimates for personnel required during phase 0 and 1.}
    %\begin{tabular}{l|r|l}
  %  \begin{tabular}{|p{4cm}|p{2cm}|p{2cm}|p{1.5cm}|p{2cm}|}
       % \hline
        %Components  & FTE Phase 0 & FTE Phase 1 & Cost (kEur) \\\hline
        % Lasers & 4 & 5  & 720  \\\hline
         
         %Transport Beamline & 3 & - & 240 \\\hline
         
         %Tunnel and laser Diagnostics & 6 & 1 & 440 \\\hline
        % Vacuum chambers & 1 & 1 & - \\\hline
        %\textbf{Total sum} &  &  & 
         %\\\hline
   % \end{tabular}
 %   \label{tab:cost_personnel}
%\end{table}

\subsection{Schedule and milestones}

The schedule for the laser system installation at the LUXE site is shown in the Fig. ~\ref{fig:schedule}. The main constraints on laser readiness are the availability of a laser cleanroom and the delivery of a new laser system (under the preferred scenario). The timelines for these two major constraints are well matched and will take about 2\textonehalf years.

 The preferred  option operationally is to install the complete 350 TW laser system. Installation of a phase-0,  40 TW laser system will result in additional downtime of the order of 6 weeks at a later point and will not allow the full range of parameters at the earliest stage.  
 
 Beamline installation can be performed at any stage. Vacuum components are relatively short lead-time items. Infrastructure work (holes in the walls/floors) is relatively quickly executed and can be fitted into short shut-downs. The beamline can be fully pre-aligned using low power lasers.
 
 Work on diagnostics (both tunnel and laser) can proceed off-line at available facilities and be stored ready for installation once the clean-room/tunnel are available for installation.
 
 The milestones for the installation are as follows:
 
 \begin{itemize}
  \setlength\itemsep{0pt}
     \item {\normalfont \bfseries~M1}	Tender ready
     \item {\normalfont \bfseries~M2}	Laser contract placed
     \item {\normalfont \bfseries~M3} Factory Acceptance Test complete
     \item {\normalfont \bfseries~M4} Laser installation complete
     \item {\normalfont \bfseries~M5} Synchronisation complete
     \item {\normalfont \bfseries~M6} Diagnostics concept finalised
     \item {\normalfont \bfseries~M7} Diagnostics installed
     \item {\normalfont \bfseries~M8}	Beamline defined 
     \item {\normalfont \bfseries~M9}	Target beamline complete
     \item {\normalfont \bfseries~M10} Automation concept complete
     \item {\normalfont \bfseries~M11} Stable operation for data runs
 \end{itemize}

\begin{figure}[htbp]
    \centering
    \includegraphics[width=01.0\textwidth]{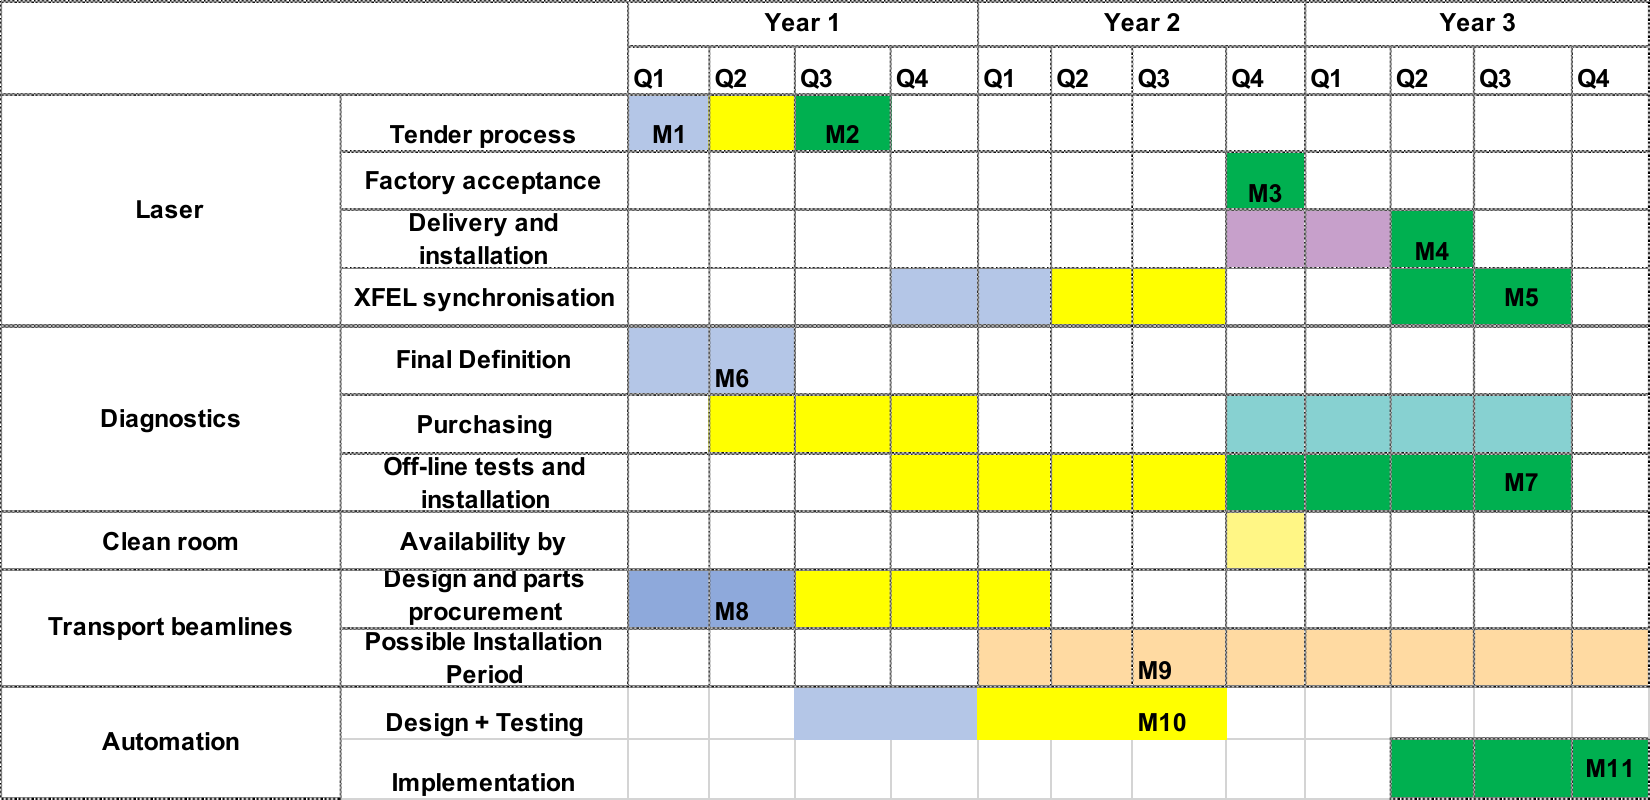}
    \caption{Schedule for the laser installation at the LUXE site.}
    \label{fig:schedule}
\end{figure}

\subsection{Risk management}
The main risks are discussed and their impact is quantified in terms of cost and schedule with respective probabilities and mitigation strategies:

There are two dimensions, the impact and the probability. We separate the impact on the cost and the schedule and use the following terms for impact risks:
\begin{itemize}
    \item Insignificant: Risk is easily mitigated by day to day process. 
    \item Minor: Delays up to 10\% of schedule. Cost increase up to 10\% of budget. 
    \item Moderate: Delays up to 30\% of schedule. Cost increase up to 30\% of budget. 
    \item Major: Delays up to 50\% of schedule. Cost increase up to 50\% of budget. 
    \item Catastrophic: project abandoned
\end{itemize}

For the budget, the denominator used is the budget of that area, i.e. if it is in the phase-0 laser area it is relative to the total phase-0 laser costs. In any case for the cost also the absolute numbers are given, so we can easily renormalize if the total cost changes.

For the schedule, the fraction is taken relative to 24 months, assuming a start in January 2022 and a readiness of January 2024. 

The probability of a risk to be realized is quantified as, rare: ($<3$\%), unlikely (3-10\%), moderate (10-50\%), likely (50-90\%) or certain ($>90\%$). 

Table˜\ref{tab:risks} shows a template for a summary of the risks.
\begin{table}[]
    \centering
    \caption{Risk description, potential impact on cost and schedule, probability to occur and strategy on how to mitigate the risk.}
\begin{tabular}{p{0.2\linewidth}|p{0.1\linewidth}|p{0.13\linewidth}|p{0.13\linewidth}|p{0.3\linewidth}}
         Description & Cost & Schedule & Probability & Strategy\\\hline
         & & & & \\\hline
         Mechanical Jitter Causes Overlap Problems & Medium 30 \% & Moderate (6~Months) & Medium (w/o tests) & Beamline Design and tests prior to installation   \\\hline
         Maintenance downtime & 10\% of laser cost pa & Lost beam weeks & High
& Schedule maintenance,
System monitoring Preemptive maintenance/ new laser rather JETI 40 \\\hline

Radiation degradation of tunnel diagnostics &
Low (replacement)  & Loss of beamtime & High & Choose components with known rad hardness, shield, spares readily available \\\hline

Laser automation not to plan & Moderate 20\%  & Medium Continuous loss of time & Medium & Start design now, Apply  proven automation strategy \\\hline

Low Damage threshold optics - shoot with lower energy & 30 \% & 10 \% & Low & test optics before installation \\\hline

Insufficient Diagnostic precision - lower data precision & Medium 30\%  & Low 10 \% & Low & test optics before installation \\\hline

Synchronisation jitter too high - intensity fluctuations in the data & Low & Medium & Low (based on HIBEF experience) & Active drift stabilisation may be required or changed IP geometry \\
\hline
\hline
\end{tabular}
\label{tab:risks}
\end{table}

\subsection{Responsibilities}
%Discuss which institute takes responsibility for what aspect.
The responsible institutions are Jena, DESY and Tel Aviv. Leadership and responsibility of the overall project is with Jena, and also of the Laser and Diagnostic sub-project. Infrastructure related planning is delegated to DESY and the vacuum chamber design is delegated to Tel Aviv.

\subsection{Laser Safety Considerations}
The LUXE laser system described  is a class 4 laser system capable of generating ionising radiation in focus.  Here we describe the main safety considerations with specific attention given to the set-up at LUXE. The detailed safety requirements are well understood and have been implemented previously at \euxfel and DESY for very similar systems. For example, the multi-100 TW Ti:Sa ReLaX laser system at the HED beamline of \euxfel is directly comparable Ti:Sa in all safety relevant aspects and the implementation of the safety system will mirror those at ReLaX closely.

\subsubsection{Laser operation modes} 
The laser will always be operated at minimum power and intensity required to ensure safety at all times. The following energy/power settings will be available and will be interlocked to appropriate operator modes.

\begin{itemize}
\item Ultra-low Intensity (nanosecond) \\
In this mode the laser uses the self-seeded regenerative amplifier (regen) described in the previous sections (i.e. the seed is blocked by an interlocked shutter). The  pulse duration is determined by the regen roundtrip time (12.5 ns in the case of JETI). This reduces the laser intensity for a given pulse energy E by 
\begin {equation}
 I_{ULI}(E)=I_{fs}(E) \frac{\tau_{Regen}}{\tau_L} <3\times10^{-6}  I_{fs}(E)\,\,.
\end {equation}
For full regen output ($<0.5$ mJ at the IP focus) the peak intensity will be   below $10^{11}$ Wcm$^{-2}$ - far below the level at which ionisation becomes relevant.
\item Low Intensity (nanosecond) \\
The same operating mode allows a maximum energy in excess of 10 mJ with  (exact values depending on Regen roundtrip time of laser) while staying below the ionising threshold for all beam sizes including the IP focus and enables the beam to be safely and easily aligned.
\item Low Intensity (femtosecond)  \\
The laser will be attenuated to intensities below ionisation threshold in the the IP focus. Depending on transport efficiency in the system this corresponds to $\mu$J level pulses.
\end{itemize}

Higher energy modes at full compression will be available with interlocked enclosures to ensure safe working. Intensities  at which ionising radiation can be present will require area interlocks to prevent access.

The interlock system will be zoned to allow operational modes to be set with lasers present only in certain restricted areas.

{\normalfont \bfseries Mode 1}: Laser-only operation\\
An interlocked shutter system will be installed prior to the beamline transporting the laser to the IP to allow the laser to be operated independently from the beamline/IP chamber for set-up purposes.
The laser shutter will be in a beam dump enclosure and be made of high damage threshold material (e.g. Alumina ceramic) to allow the laser to be operated at up to full power with the energy being dumped/diffused in the shutter/beamdump assembly.

This mode will have different interlock settings  on intensity depending on whether the laser beam can be accessed by the operator or if the compressed beam is fully enclosed.\\

{\normalfont \bfseries Mode 2}: Interaction Point (IP) Mode \\
In IP mode the laser will be allowed to propagate to the IP chamber. The availability of the energy modes will depend on the interlock status (IP area without personnel, IP area with vacuum system closed (no access to high intensity), IP area and chamber accessible).

%We need to also ensure that a safe level of laser energy is reached in the IP chamber. All q-switches of the pump lasers of the amplifiers will be interlocked. Meaning that during the alignment in the interaction area, the main amplification can not take place. The front end energy (about $500 \mu$ J ) will be only available. Such level of energy is required to align for example during the set up of optics inside the IP camber. The focused intensity at the IP will be 2.1016 W/cm2 for a tight focus diameter of $3\mu$ m (FWHM). However, the intensity outside the area of 3mm2 will be already below 10w/cm2 due to the fast diverging beam (beam diameter at 2cm from IP= 0.66cm). 

%{\normalfont \bfserieshigh power alignment} \\

The focus of the laser must be characterised both with the IP diagnostic and with the diagnostic system. Meaningful measurement requires the laser to operate under full power conditions.  To ensure that the energy in the pulse does not exceed the one in the alignment case, an interlockable $10^{-6}$ attenuator  will be inserted in the path of the laser beam after the last stage of the amplification and before the compressor. This attenuator consists of high quality ($<\lambda/20$) uncoated mirrors mounted in a so called dog-leg geometry. The insertion of this attenuator will be done using a motorised translation stage. This stage can be interlocked with the laser to ensure that attenuator is at in position when the beam is fully amplified.  A pointing monitor in laser bay with switchable attenuation will ensure that the laser is propagating down an identical path both with and without the attenuator present.\\

{\normalfont \bfseries High power mode} \\

For operation at full power (data acquisition and full power live diagnostic laser only).  The IP area will be searched and fully locked, so that no one can access it while the laser is operating at full power and/or the electron beam is present. In this mode the  full energy laser pulse can be delivered at the IP and, after initial attenuation in the IP chamber, propagate to the diagnostic suite in the laser clean room.  Interactions of the GeV beam with the laser pulse can take place.

\subsubsection{Safety protocols}
%do we need to describe all the details of safety interlocks, emergency switches, entry to the laser room etc?\\
In other labs at DESY \cite{laser28m} and in EuXFEL-HIBEF (which host $> 300$ TW class IV lasers) \cite{hibef} the safety procedures for the alignment and focus check is as discussed above. This is so called``Justierung mode-alignment mode". The main safety interlock is at the attenuator which does not allow high energy in the pulse when the laser is in alignment mode. During the ``Sperrbereich-mode" (shooting mode), the interaction area is fully locked and the attenuator moves out of the beam path allowing full energy in the pulse. Other standard procedures are the announcement of the laser beam being sent to the IP area and when the interaction area is being locked for the high power interaction mode.

\subsection{Budget Summary}
The costs listed in the previous section are given with more granularity.  Table   ~\ref{tab:New_laser_system_cost} breaks down the individual laser components and upgrade cost from a phase-0 to phase-1 system. Here phase-0 is conceived to have common components at phase-1 specification, with the upgrade consisting of additional amplification and pump lasers. The costs arising in the other areas of this TDR are shown in tables  ~\ref{tab:laser_area_diag_cost}  for the laser area diagnostics,  ~\ref{tab:laser_beamline_cost} for the transport beamline and ~\ref{tab:TA_diagnsotics_cost} for the target area diagnostics. The costing for the hardware part is presented in Infrastructure note \cite{LUXETDR-Infra}. Finally we show for comparison the phase-0 option with the JETI 40 laser in table ~\ref{tab:Jeti40_laser_system_cost}. The investment savings over the project lifetime are clearly limited and very small compared to the total cost of LUXE. On the downside there is the high risk of additional unscheduled maintenance downtime with the possibility that some of the pump lasers might need full replacement during the running period of LUXE. 

\begin{table}[]
   \centering
   \caption{Detailed cost estimates for the new laser system only.}
    %\begin{tabular}{l|r|l}
    \begin{tabular}{|p{4.5cm}|p{1.5cm}|p{4.5cm}|}
       \hline
         & Cost (kEur) & Comment\\\hline
        Laser system phase-0  & 1650 & quote from manufacturer\\ \hline
       Compressor and chamber & 250 & {laser manufacturer quote}\\\hline
         
        Timing system (with EuXFEL master clock)  & 80 & estimates based on input\\\hline
         
         Automation cost & 250 & {estimates based on  quotes and experience}\\\hline
        Oscillator & 160 & {based on  quotes}\\\hline
        Attenuation, shot and  energy control & 195 & {laser manufacturer quote}\\\hline
        Adaptive Optic & 140 & {based on  quotes}\\\hline
       
       \textbf{Phase-0} & \textbf{2725} & \\\hline \hline
       Upgrade to 350 TW & 1700 & {laser manufacturer quote}\\\hline
        
       \textbf{Phase-1}  & \textbf{4425} & \\\hline
        350 TW Laser system for Phase 1  & 3050 & quote from Thales\\\hline
        \textbf{Total sum for phase 0 and 1} & \textbf{3825} & 
        \\\hline
    \end{tabular}
    \label{tab:New_laser_system_cost}
\end{table}

\begin{table}[]
   \centering
    \caption{Laser area diagnostics costing.}
    %\begin{tabular}{l|r|l}
    \begin{tabular}{|p{4.5cm}|p{1.5cm}|p{4.5cm}|}
       \hline
       Laser area diagnostics  & Cost (kEur) & Comment\\\hline
        Wizzler & 35 & estimates based on quote \\\hline
        Sequoia & 30 & quote \\\hline
        Insight  & 60 & estimates based on quote\\\hline
        Spot CCD microscope & 7 & quote \\\hline
        Vacuum chamber for the diagnostics & 45 & estimates based on quote\\\hline
         Pump & 13 & {estimates based on  quote}\\\hline
         Optical tables & 15 & quote \\\hline
         Adaptive optics & 25 & estimates based on quote\\\hline
         Small optics and mounts & 25 & {estimates based on  quote}\\\hline
Nonlinear 2D detectors & 25 & estimates based on quote\\\hline
        Off axis parabola & 30 & {estimates based on  quote}\\\hline
        \textbf{Total sum} & \textbf{310} & 
         \\\hline
    \end{tabular}
   \label{tab:laser_area_diag_cost}
\end{table}

\begin{table}[]
    \centering
    \caption{Laser beamline costs. Tubing, pumps and gate valves are costed in the Infrastructure note TDR.}
    %\begin{tabular}{l|r|l}
    \begin{tabular}{|p{4.5cm}|p{1.5cm}|p{4.5cm}|}
       \hline
       Laser Beamline  & Cost (kEur) & Comment\\\hline
         Mirror mounts & 110 & estimates based on quote \\\hline
         Optics & 200 & quote \\\hline
         Crosses  & 40 & estimates based on input\\\hline
        Mounting breadboards & 50 & quote \\\hline
        \textbf{Total sum} & \textbf{400} & 
         \\\hline
    \end{tabular}
    \label{tab:laser_beamline_cost}
\end{table}

\begin{table}[]
  \centering
   \caption{Detailed cost estimates for the vacuum chambers.}
   \begin{tabular}{|p{4.5cm}|p{1.5cm}|p{4.5cm}|}
       \hline
       Vacuum chambers  & Cost (kEur) & Comment\\\hline
        IP chamber & 40 & estimates based on quote \\\hline
        ICS and gamma chamber & 15 & quote \\\hline
        
       \textbf{Total sum} & \textbf{55} & 
        \\\hline
   \end{tabular}
   \label{tab:vacuum_chamber_cost}
\end{table}

\begin{table}[]
    \centering
    \caption{Tunnel diagnostic costs.}
    %\begin{tabular}{l|r|l}
    \begin{tabular}{|p{4.5cm}|p{1.5cm}|p{4.5cm}|}
        \hline
        Target area diagnostics  & Cost (kEur) & Comment\\\hline
         Microscope & 8 & estimates based on quote \\\hline
         EO Timing tool & 4 & previous quotes \\\hline
         Beam dump  & 3 & estimates based on input\\\hline
         axis parabolas & 30 & quote \\\hline
        Linear stages & 50 & estimates based on quote\\\hline
        Mounts for parabolas & 20 & {estimates based on  experience}\\\hline
       \textbf{Total sum} & \textbf{115} & 
        \\\hline
    \end{tabular}
    \label{tab:TA_diagnsotics_cost}
\end{table}

\begin{table}[]
    \centering
    \caption{Cost estimates for the JETI 40 option to phase-0 and phase-1.}
   % \begin{tabular}{l|r|l}
   \begin{tabular}{|p{4.5cm}|p{1.5cm}|p{4.5cm}|}
        \hline
        Jeti 40 Laser system Phase 0  & Cost (kEur) & Comment\\\hline
         Optical Tables & 30 & estimates based on quote \\\hline
         Oscillator with synchro lock & 160 & quote \\\hline
         Timing system (with EuXFEL master clock)  & 80 & estimates based on input\\\hline
         Jeti 40 laser & 0 & in-kind contribution \\\hline
         Transport of Jeti 40 to XS1 & 5 & estimates based on experience\\\hline
        New pump laser & 250 & {estimates based on  quotes}\\\hline
        Automation cost & 250 & {estimates based on  quotes and experience}\\\hline
         spare pump laser for front end & 40 & estimates based on  quotes\\\hline
         Additional Staff costs & 160 & estimate\\\hline
       & &  \\\hline
       \textbf{Total phase-0} & \textbf{975} & \\\hline
       Full size adaptive optics & 140 & based on quote\\\hline
        Full size compressor & 250 & laser manufacturer quote\\\hline
        Attenuation, shot and energy control  & 195 & laser manufacturer quote \\\hline
        Energy upgrade & 1700 & laser manufacturer quote \\\hline
        Additional maintenance costs & 300 & estimates\\\hline
        & & \\\hline
        \textbf{Total phase-1} & \textbf{3560} & \\\hline
        
        \textbf{cost to upgrade to 350 TW} & \textbf{3050?} & \textbf{estimates based on  quotes}\\\hline
        350 TW Laser system for Phase 1  & 3050 & quote from Thales\\\hline
        \textbf{Total sum for phase 0 and 1} & \textbf{3825} & 
        \\\hline
   \end{tabular}
    \label{tab:Jeti40_laser_system_cost}
\end{table}

\section{Pixel Tracker}
% Includes organisation of work at institutions, discussion of main technical milestones (e.g. internal or external reviews, test beam campaigns etc.) and interfaces to common services.
% Also discusses which institution contributes how.
The related 
%costs, 
manpower and timelines are discussed in detail.

For the installation timeline of the tracker alone, we consider the following three baseline scenarios:
\begin{enumerate}
    \item during the 2024 shutdown,
    \item during 2025 summer shutdown (2 weeks),
    \item during 2025 winter shutdown (4-6 weeks).
\end{enumerate}
The priority will be to finish the installation in scenario 1.
If it is missed due to technical or financial reasons, then the other scenarios may come into play.

In that respect, the ``bare-bones'' tracker scenario is particularly important to outline, as this is the most likely case fit for scenario This case is therefore detailed independently.

\subsection{Manpower}
\label{sec:manpower}
The manpower requirements follow a two-step logic: (i) design (including simulation), installation and commissioning in ``period A'', and (ii) operation, maintenance and analysis during ``period B''.

In period A, generally one postdoctoral research fellow (PD), one PhD student, one technician, one mechanics engineer/designer and one electronics engineer are required (besides the WIS PI and staff-scientist).
The technicians and engineers of this team are based on WIS personnel of the faculty of physics ``core facilities'' (PCF) department.
This technical team is highly experienced and can be hired on a day-by-day basis.
This arrangement allows maximum flexibility with respect to the schedule compared to the alternative, which essentially involves hiring of equivalent manpower.

Before installation at the experiment, this team is not needed at 100\% FTE, except for the PD.
The design and simulation, including the mechanics is already underway with one PD at 100\% FTE and one mechanics engineer at $\sim 5-10\%$ FTE.

As initial modules (one stave, FELIX, ...) will arrive at WIS, an involvement of an electronics engineer at $\sim 5-10\%$ FTE and a technician at $\sim 5-10\%$ FTE is foreseen (PCF personnel).
This equipment is expected before the end of 2021 independent of LUXE's timeline or budgeting and based on private WIS budget.
This will allow to gain experience with the end-point detector elements and to progress on many fronts (mechanics, cooling, FELIX, readout, software, etc.) even before the bulk budget will arrive.

Once the quantities of detector modules purchased for LUXE will start to arrive at WIS, the work will gain speed with increased involvement of the PCF personnel.
A PhD student is required to be recruited early enough before that point in order to participate effectively in the construction.
Particularly, the reception, testing and assembly of the tracker modules will be done at this step.
The assembled equipment will be shipped to DESY, tested on-surface and installed in the experimental hall by the personnel described above.

As discussed in Section~\ref{sec:install}, the installation itself in period A, a team of at least 5-6 FTEs will be needed.
The team will consist of one WIS PI, one WIS scientist (or a postdoc), one postdoc/student, 1-2 WIS technicians and potentially one WIS electronics expert.
The installation will take at least 2-4 straight weeks, with $\sim$one week on surface and $\sim 2-3$ weeks in the experiment hall.
During that time the team will be fully dedicated to the installation.
With this team in mind, the installation can fit the timeframe of any of the three scenarios outlined at the beginning of this Section.
It would be particularly comfortable in the first scenario, but it can also be fitted in the second or third (shorter) scenarios, given the extra time that will be used to make as much progress as possible at WIS and on-surface at DESY.

In period B, at least one PD and one PhD student are required.
This is expected over a period of three years at least.
It is assumed that minimum technical intervention will be needed at this step.
Hence, the technical team is not needed for extended periods, while in special cases where short technical interventions are needed, these could be covered based on the same WIS technical personnel.
The tasks to be covered in period B by student(s) and postdoc(s) will include software development, data-quality monitoring, on-call expert shifts, etc.
%The PD and PhD components in period B are not included in Table~\ref{tab:cost}.

\subsection{Risk management}
\label{sec:risks}
The main risks are discussed and their impact is quantified in terms of cost and schedule with respective probabilities and  mitigation strategies:
\begin{itemize}
    \item Insignificant: Risk is mitigated by day to day process,
    \item Minor: delays up to 10\% of the schedule and the cost increases by up to 10\% of the budget,
    \item Moderate: delays up to 30\% of the schedule and the cost increases by up to 30\% of the budget,
    \item Major: delays up to 50\% of the schedule and the cost increases by up to 50\% of the budget,
    \item Catastrophic: project abandoned,
\end{itemize}
where the fractions for the budget are taken relative to the overall tracker-project budget alone.
The fractions for the schedule are taken relative to 24 months, assuming a start in January 2022 and readiness on January 2024.
The probability of a risk to be realized is quantified as: rare ($<3$\%), unlikely (3-10\%), moderate (10-50\%), likely (50-90\%) or certain ($>90\%$).

This analysis is done for the \underline{full tracker} scenario.
Similar tough reduced conclusions may be also applied to the ``bare-bones'' tracker scenario.

Table~\ref{tab:risks} shows a summary of the risks analysis.
\begin{table}[!h]
\centering
\begin{tabular}{p{0.22\linewidth}|p{0.05\linewidth}|p{0.1\linewidth}|p{0.12\linewidth}|p{0.37\linewidth}}
Description & Cost & Schedule & Prob. & Mitigation strategy\\
\toprule
%%%%%%%%%%%%%%%%%%%%%%%%%
Problems in the detector design (mostly sensors, readout and DAQ) & 30\% & 30\% & Moderate & Testing of initial modules will start in 2022 with a milestone set for full chain test around Aug 2022 with three months of contingency before modules must be ordered.\\\hline
%%%%%%%%%%%%%%%%%%%%%%%%%
Budget not identified by Oct 2022 & 50\% & 50\% & Likely &Push installation to winter 2025.\\\hline
%%%%%%%%%%%%%%%%%%%%%%%%%
Stave production is delayed & 10\% & 10\% & Unlikely & Contingency of 2 months is taken on top of the most conservative estimate from ALICE. Can also compensate later by descoping testing and assembly steps at WIS.\\\hline
%%%%%%%%%%%%%%%%%%%%%%%%%
CAEN, RU and/or PU production is delayed & 20\% & 10\% & Unlikely & Contingency of 2 months is taken. Can also compensate later by descoping testing and assembly steps at WIS.\\\hline
%%%%%%%%%%%%%%%%%%%%%%%%%
WIS integration is delayed & 10\% & 10\% & Moderate & Contingency is allocated. Reception tests can be descoped to the bare minimum while prioritising connectivity tests and assembly procedures only.\\\hline
%%%%%%%%%%%%%%%%%%%%%%%%%
Leak-less cooling concept underestimated & 20\% & 10\% & Moderate & Contingency is allocated. Start design early in 2022 with WIS experts and in consultation with ALICE engineers. If too expensive and/or complicated work with normal flow (no under-pressure) and take the risk of small (vertical) leaks.\\\hline
%%%%%%%%%%%%%%%%%%%%%%%%%
Radiation in the position of the power system and/or readout backend is too high (from simulation) & 20\% & 30\% & Moderate & Scrutinise design based on detailed dose simulation with proper shielding. If necessary, upgrade the power supply system to the hostile-compatible version (with higher cost and complexity) and increase the shielding.\\
\bottomrule
\end{tabular}
\caption{Risk description, potential impact on cost and schedule, probability to occur and strategy on how to mitigate the risk. The different risks are tied to the steps outlined in Fig.~\ref{fig:schedule}.}
\label{tab:risks}
\end{table}

\subsection{Responsibilities}
\label{sec:responsibilities}
When writing up this document, the responsible institution is only WIS.
The PI of the WIS group devotes $>50\%$ of the time to the LUXE project and particularly to the development of the tracker. 
The facilities and equipment at the WIS lab are also adapted to this purpose.
On top of that, the availability of the faculty's PCF department technical personnel on demand is invaluable.
The mechanical design of different elements in LUXE (not only the tracker) is already benefiting from the expertise of the PCF instrument design team.
Moreover, the expertise of the PCF electronics and DAQ team will be particularly important for the FELIX adaptations (FELIX was developed by WIS experts and is still being worked on for ATLAS phase-1 and phase-2 upgrade campaigns).

\section{Electromagnetic Calorimeter}

\subsection{Human and financial resources}
%Estimate of human and financial resources required. For the financial resources the sources (e.g. company quotes, experience from previous work...) and uncertainties should be provided. For the human resources it should be clarified what type of people are needed.

ECAL-E and ECAL-P will be built in a joint effort of the AGH-University of Technology (AGH-UST) Cracow, Instituto de Fisica Corpuscular (IFIC),
the Kyushu University (KU), the Laboratoire de Physique des 2 Infinis Irène Joliot-Curie, (IJC) Paris, the 
Laboratoire Leprince-Ringuet (LLR) Paris, the
Institute of Space Science (ISS) Bucharest, the Tel Aviv University (TAU) and the University of Warsaw (UW). These institutes will provide the human and financial resources needed for the design, production, test, commissioning and operation of ECAL-P.
The group of AGH-UST comprises 5 experienced researchers, specialised in ASIC design, 1 technician and several students.
At IFIC, one experienced researcher and one Ph.D. student will perform the gluing.
From the Kyushu University one researcher specialised on sensors will join. The 
Laboratoire -Ringuet Paris will contribute with mechanics, sensor assembly and electronics of ECAL-E with 2 researchers.
From the ISS group, 3 physicists experienced in software and data handling are included. 
The TAU group comprises 3 experienced physicists, 1 part-time technician (full time technician will be hired in the near future), one postdoc, and several graduate students.  The University of Warsaw participates with 2 experienced researchers, one student (postdoc candidate) and engineering support to design and build the mechanical frame of ECAL-P. 

The cost estimates for the production of ECAL-E and ECAL-P are given in Tables~\ref{tab:cost_ECAL-E} and ~\ref{tab:cost_ECAL-P}.
\begin{table}[h]
    \centering
    \caption{Cost estimates for the various components of ECAL-E. The comment in parentheses gives the source of the price. The meaning of the quality factor is given in the appendix.}
        \begin{tabular}{|l|r|l|c|l|}
         \hline
        Component  & Cost         & responsible lab               & Quality     & Status\\
                   &  (kEur)      & (origin of estimates)        & factor      &        \\
         \hline
         Mechanics &    10        &  IJC (previous projects)  &   1         & design\\
         Sensors   &    120       &  KU, LLR, IFIC, IJC       &   1         & Prototyping\\
                   &              &  (offer by the vendor)        &             &            \\
         FE ASICs  &    165      &    IJC, LLR                    &       2    & design ready  \\
                   &              &    (recent submissions)        &            &        \\
         PCBs      &    30        &    LLR, IJC                    &    1       &   \\
                   &              &    (previous production)       &            & \\
         DAQ       &    10        &   IJC                          &      1     & \\
         Power supplies &  20     &   IJC (current offers)         &    1  & \\
         Tooling and gluing   & 25 &  IFIC , IJC                   &     1       & \\
         Tungsten   &    30       &   LLR (offer by the vendor)   &     1       & \\ 
         Auxiliary  &    20       & IJC, LLR (experience from              &     1        & \\
         components &             & previous projects)            &              & \\ 
         \hline
         Total sum  &  430  &   & &
         \\  \hline
    \end{tabular}
    \label{tab:cost_ECAL-E}
\end{table}
\begin{table}[h]
    \centering
    \caption{Cost estimates for the various components of ECAL-P. The comment in parentheses gives the source of the price. The meaning of the quality factor is given in the appendix.}
        \begin{tabular}{|l|r|l|c|l|}
         \hline
        Component  & Cost         & responsible lab               & Quality     & Status\\
                   &  (kEur)      & (origin of estimates)        & factor      &        \\
         \hline
         Mechanics &    40        &  UW (previous projects)        &   1         & design\\
         Sensors   &   100        &  TAU                           &   1         & Prototyping\\
                   &              &  (offer by the vendor)         &             &            \\
         FE ASICs  &    165       &   AGH-UST                      &       2    & Redesign  \\
                   &              &    (recent submissions)        &            &        \\
         PCBs      &    22        &    AGH-UST, TAU                &    1       &   \\
                   &              &    (previous production)       &            & \\
         DAQ       &    27        &   TAU (FCAL experience)        &      1     & \\
         Power supplies &  20     &   AGH-UST, TAU (current offers)&    1       & \\
         Tooling and gluing & 30  &   IFIC, TAU                    &     1       & \\
         Tungsten   &    30       &   TAU (offer by the vendor)    &     1       & \\ 
         Auxiliary  &  30         &   AGH-UST, TAU (experience from              &     1        & \\
         components &             & previous projects)            &              & \\ 
         \hline
         Total sum  &  464  &   & &
         \\  \hline
    \end{tabular}
    \label{tab:cost_ECAL-P}
\end{table}
 The major cost drivers are the sensors and the FE ASICs. TAU will cover the sensor costs for ECAL-P; received support from the PAZY Foundation (Israel Atomic Energy Commission) and will apply for support from the Israel Science Foundation. For the sensor costs of ECAL-E, the labs in the table above will make a joint application to their funding agencies.  
 Compared to the CDR, the estimated price of FE ASICs has increased by about 25\% mainly due to expected increased production costs. 
 To cover the costs of the FE ASICs of ECAL-P the AGH-UST group has successfully applied for a grant from the Polish National Science Centre.
 
 To cover the costs for the mechanics, the UW will apply for support from the national funding agency. Costs for tungsten plates of precise thickness and flatness will be shared between LLR and TAU. The DAQ will be partly funded from the AGH-UST application. IJC and LLR will apply for additional funding. PCBs, power supplies, tooling and auxiliary components will be shared between AGH-UST,  TAU and IJC. IFIC will apply for funding to cover the costs for contact gluing, including the necessary tools. 
 
 In addition, TAU together with the DESY and Freiburg University groups and other participants from Israel and Germany recently applied to the German-Israeli Project Cooperation (DIP) in the 2022 call. If successful, some funds will be dedicated to the shortfalls in the ECAL-P funding, if necessary.
 
 The ECAL-E collaborators in LUXE are also involved in the CALICE SiW calorimeter prototype effort. At the moment it can be assumed that the funding in the next two to three years will be continued at the current level in the frame of the base funding for CALICE and Linear Collider activities. The person-power situation is such that there are at the moment around ten senior researchers and engineers, one postdoc, four PhD students and one master student, and the expectation is that the same level of manpower will remain available for the next two or three years. A positive development towards a Higgs factory as well as the creation of the French-German lab DMLAB, may lead to an improvement of the situation.  
 Currently available is the CALICE prototype ECAL, covering a fiducial area of $18\times 18 \units {cm^2}$, fully equipped with sensors, FE electronics and DAQ. The installation of this ECAL in LUXE would need only a small amount of additional funding. For a full coverage of ECAL-E, a second and a third stack of the same size has to be added, for which additional 430 kEuro are needed.

\subsection{Schedule and milestones}
%Describe here the schedule and the milestones. Normally we will try to be ready for installation by January 2024. There will be risks to that which we can treat as risks and the mitigation is to install later. 

The schedules for the construction of ECAL-E and ECAL-P are shown in Fig.~\ref{fig:ECAL_E_timeline}
and Fig.~\ref{fig:ECAL_P_timeline}.

\begin{figure}[htbp]
 \begin{center}
% \hspace*{-1.5cm}
  \includegraphics[width=\textwidth]{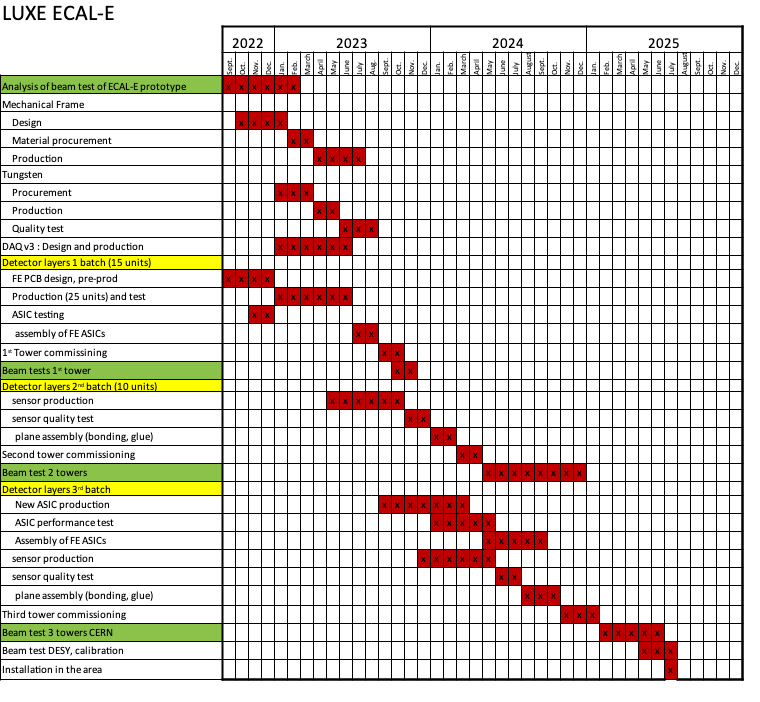}
 % \vspace*{-10.5cm}
    \caption{The time schedule for the construction, test and commissioning of 
    the ECAL-E.} 
    \label{fig:ECAL_E_timeline}
    \end{center}
\end{figure}
\begin{figure}[htbp]
 \begin{center}
 \hspace*{-1.5cm}
  \includegraphics[width=\textwidth]{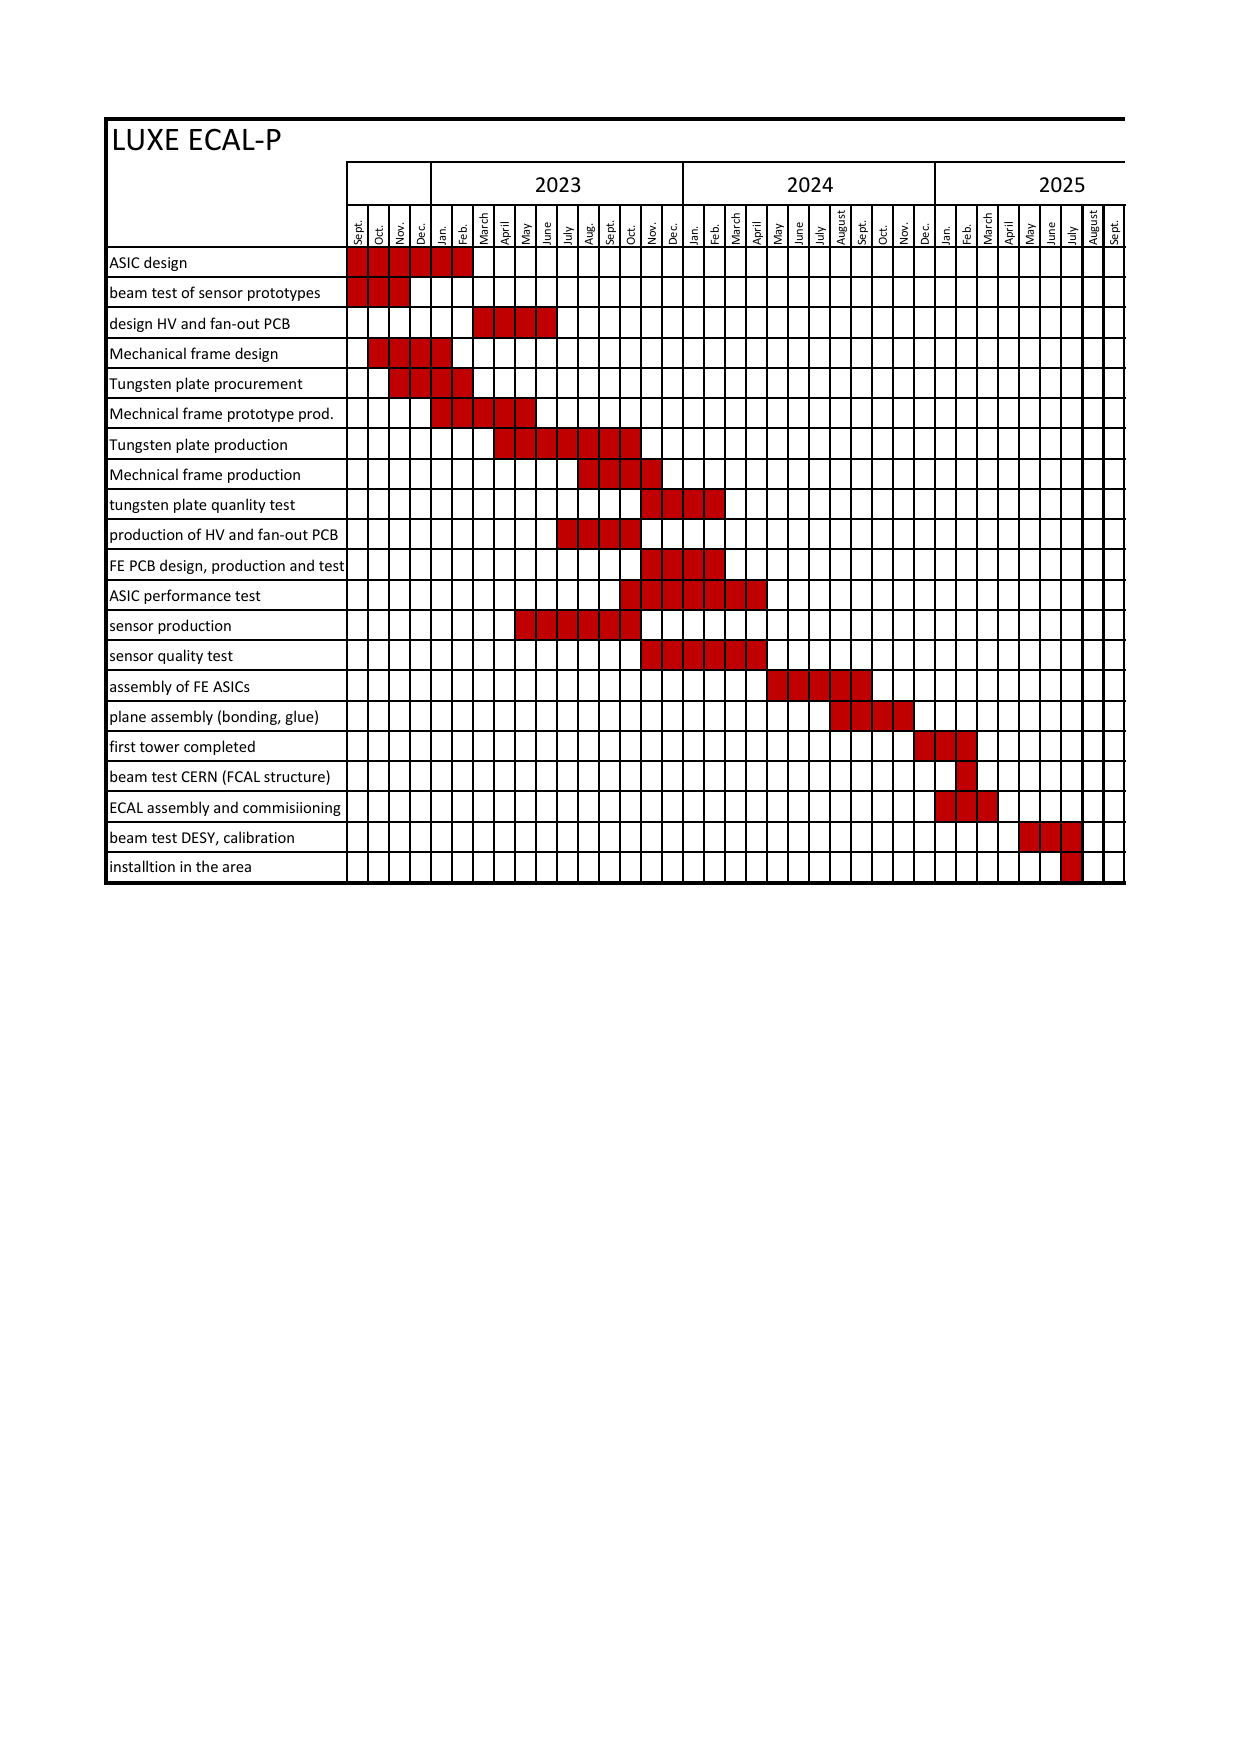}
  \vspace*{-10.5cm}
    \caption{The time schedule for the construction, test and commissioning of the ECAL-P.} 
    \label{fig:ECAL_P_timeline}
    \end{center}
\end{figure}

%
% The major milestones ahead are the following:
%\begin{enumerate}
%    \item{Tungsten plate quality check - July 2022.}
%    \item  {Sensor performance measurements in test-beam in November 2021 and September 2022, followed by technology choice in February 2023.}
%    \item { Completion of the ASIC production in June 2023.}
%   \item { Completion of the sensor production in October 2023.}
%    \item { Completion of the sensor plane instrumentation in March 2024.}
%    \item { Completion of ECAL-P assembly in April 2024.}
%   \item { Beam-tests of fully assembled ECAL-P at DESY in May 2024.}
%    \item { Readiness for commissioning by July 2024.}
%\end{enumerate}

\subsection{Risk management}

Two major elements may impact the time-line and the costs of ECAL-P construction. One pertains to the sensors, the other to the readout delivery. 

 The impact on the costs and the timeline of the ECAL-P is negligible as the sensors prices are based on current offers by Hamamatsu. The funding is not yet fully guaranteed for TAU. The labs of ECAL-E are still in the stage of the preparation of applications for funding for the sensors of the second and third tower. A better assessment will be known by December 2022. The expectation is that if the LUXE project goes ahead, shortfalls in funding if any, will be covered potentially by request of extra support from TAU research funds if not from DIP. 

 For the ASIC production, time delays of the order of 6 months may be expected. Another factor is an increase in pricing which may be of the order of 25\% (included in the price estimate). As a mitigating action, for ECAL-P the existing FLAME boards will be used for testing purposes. According to the present schedule, that would give an extra 9 months for completing the production and testing of the FLAXE readout boards. For the ASICs of the second and third tower of ECAL-E funding applications will be prepared.
 
 Since March 2022, the ECAL-P team developed a strategy to mitigate the effects of the present political crisis, since deliveries from Russian collaborators are unlikely. New partner (UW, IFIC) took over the responsibility for the mechanics
 and sensor plane assembly. In IFIC a funding application is pending, and UW applies for funding.  
ECAL-E can in case of major delays in ASIC production only partially assembled.
In the worst case scenario, where the lack of funding would prevent the delivery of ECAL-P on time for the \phaseone data taking, the ECAL-E with at least one tower will be used on the positron side, leaving the electron side uninstrumented for the \glaser runs. .

An attempt to summarise the risks is presented in Table~\ref{tab:risks}.

%Table~\ref{tab:risks} shows a template for a summary of the risks.
\begin{table}[h]
    \centering
    \caption{Risk description, potential impact on cost and schedule, probability to occur and strategy on how to mitigate the risk.}
\begin{tabular}{|p{0.2\linewidth}|p{0.1\linewidth}|p{0.1\linewidth}|p{0.1\linewidth}|p{0.3\linewidth}|}
        \hline
         Description & Cost & Schedule & Prob. & Strategy\\\hline
 FEB chip production      & $\pm 10\%$ & 25\% to 35\% & 30\% & Adapt existing FLAME readout\\
         \hline
         \end{tabular}
         \label{tab:risks}
\end{table}

\subsection{Responsibilities}
Each institute or university will be responsible for a component of ECAL-E and ECAL-P, as shown in Table  
~\ref{tab:responsibilities}.
\begin{table}[h]
    \centering
    \caption{The participating institutes and their main responsibilities in the ECAL-E and ECAL-P construction.}
    \begin{tabular}{|l|l|}
    \hline
        Institute/University  & contribution to ECAL-E \\ \hline
         IFIC    &  contacts of sensors pads with readout traces using conductive glue, sensors  \\
         IJC    &  sensors, readout, DAQ, PCB \\
         KU     &  sensors, contact to Hamamatsu  \\      
         LLR    &  sensors, PCB, assembly, tools, precise tungsten plates  \\
       \hline
       \hline
        Institute/University  & contribution to ECAL-P \\ \hline
         AGH-UST    &  FE-ASICs development and production, DAQ \\
         IFIC    &  contacts of sensors pads with readout traces using conductive glue, sensors  \\
         ISS    &  slow control, software, computing infrastructure \\
         TAU    &  sensors, assembly of detector planes, DAQ \\
         UW     &  design and prototyping of the mechanical frame\\
       \hline
    \end{tabular}
    \label{tab:responsibilities}
\end{table}
A prototype of ECAL-E (CALICE Prototype) has been operated in test-beams at DESY and CERN. The Data analysis is ongoing, and results on the performance are expected within a few months. With relatively small modifications this prototype will be the first tower of ECAL-E. The additional towers will need
further system tests.
To study the performance of sensors and ECAL-P towers, and finally a full system test and calibration, measurements will be done in the test-beam. These campaigns will be organised and funded as a joint effort.

The installation and commissioning of ECAL-E and ECAL-P will again be done in a joint effort, as described in the resource loaded schedule for ECAL-P as example, in appendix A.

\section{Scintillator Screens \& Camera System}
\subsection{Human and Financial Resources}
In Table \ref{tab:scint_costing} is a costing of the screen and camera system(s). Not taken into account is the engineering work required for installation or construction of optical tables - as these are at least shared with the \cer device. These costs are taken to be accounted for within the technical infrastructure estimate (see chapter~\ref{chapt12}). Mounts specific to the screen and cameras, essentially the frame to hold the screen and the mounts for cameras/lenses, \textit{are} costed.  

\begin{table}[h]
\caption{Estimates for costs relating to the scintillation screen. The screen and camera and accessories are increased in number for back-ups and are costed here (2 back-ups for each camera position). The equipment costs are for each instance, and so the cost is also given doubled to include implementation in both regions. Percentage values for labour represents the expected fraction of full-time work expected multiplied by the total cost of the position for this detector at LUXE. }
\label{tab:scint_costing}
\begin{center}
\begin{tabular}{ lclc }
  \hline\hline
  Item 							& Unit price (\EUR{}) 		& Quantity 		& Total price (\EUR{})	\\
  \hline
  Equipment needed\\ for each site: \\
  \hline
  GadOx screen			& 1000			& 2			& 2000 \\
  4K camera     		& 1400			& 3			& 4200 \\
  2K camera             & 400           & 6         & 2400 \\
  $f$=50\,mm lens      	& 250			& 4		    & 1000 \\
  $f$=75\,mm lens       & 600           & 2         & 1200 \\
  Optical Filter                & 725           & 6         & 4350 \\
  Neutral Density Filter & 50 & 2 & 100 \\
  Scintillator Frame    & 1000          & 2         & 2000 \\
  Camera Mounts \& Shielding & 2000     & 2         & 4000 \\
  \hline
  Total equipment, one site				&  					&  				& 21250 \\
  \hline
 \multicolumn{4}{l}{Equipment sharable between both sites/exclusive to one site:} \\
  \hline
  Additional Computing/cabling & 1000 & 1 & 1000 \\
  Calibration Lamp & 1000 & 1 & 1000 \\
  Optical Target(s) & 500 & 1 & 500 \\
  Ceiling Mount Apparatus & 5000 & 1 & 5000 \\
  \hline
   Total equipment both sites	&  					&  				& 49900 \\
  \hline
  25\% PostDoc (3 years)				& 						&					& 75000	\\
  PhD student (3 years)			& 						&					& 75000	\\
  25\% PhD student (5 years) 	& 						&					& 31250	\\
  \hline
  Total non-equipment		& 						&					& 181250 \\
  %\hline
  %Total					&  					&  				& 207400 \\
\hline\hline
\end{tabular}
\end{center}
\end{table}

\subsection{Schedule and Milestones}

Unlike the custom-built detectors common to high-energy physics, these ``off-the-shelf" components leave  comparatively few formal milestones to complete in the construction of the detector. These are listed below: 

\begin{itemize}
    \item Convergence upon a design for the scintillation screen and camera system (2021, completed). 
    \item Prototype testing and quality control (2022/2023, underway). 
    \item Collection and assembly of all commercially sourced components (2022/2023).
    %\JH{irradiation tests??}
    \item Measurement of a light--charge calibration curve with a high-population electron bunch user beam facility (late 2022/2023).
    \item Integration with Cherenkov detector and DAQ and control system (2023).
    \item Pre-installation preparations (2023/2024).
    \item Final Installation in the \euxfel chamber (2024)
\end{itemize}

This schedule ensures a detector ready for installation 2024. In the case of delays of the rest of the experimental setup, deeper analyses of the system, in particular with regard to the detector's resistance to radiation, can be performed before installation. The current state of the system includes a prototype with at least 2 of each component (camera, lens, filter, screen) and developing data acquisition software. The software for reconstruction is well underway and used in the performance chapter on results from a \geant simulation. 

%Describe here the schedule and the milestones. Normally we will try to be ready for installation by January 2024. There will be risks to that which we can treat as risks and the mitigation is to install later. 

%The level of detail of milestones should be quite high but maybe we should put it partially into an appendix. 

\subsection{Risk Management}

%Plain text that discusses the main risk factors, how/if they impact cost and/or schedule, their probability and how they are mitigated.

%There are two dimensions, the impact and the probability. We separate the impact on the cost and the schedule and use the following terms for impact risks:
%\begin{itemize}
%    \item Insignificant: Risk is easily mitigated by day to day process. 
%    \item Minor: Delays up to 10\% of schedule. Cost increase up to 10\% of budget. 
%    \item Moderate: Delays up to 30\% of schedule. Cost increase up to 30\% of budget. 
%    \item Major: Delays up to 50\% of schedule. Cost increase up to 50\% of budget. 
%    \item Catastrophic: project abandoned
%\end{itemize}
%For the budget, the denominator used is the budget of that area, i.e. if it is in the phase-0 \laser area it is relative to the total phase-0 \laser costs. In any case for the cost also the absolute numbers are given, so we can easily renormalize if the total cost changes.

%For the schedule, the fraction is taken relative to 24 months, assuming a start in January 2022 and a readiness of January 2024. 

%The probability of a risk to be realized is quantified as, rare: ($<3$\%), unlikely (3-10\%), moderate (10-50\%), likely (50-90\%) or certain ($>90\%$). 

Table \ref{tab:risks} shows a summary of the risks.
\begin{table}[]
    \centering
    \caption{Risk description, potential impact on cost and schedule, probability to occur and strategy on how to mitigate the risk. }
\begin{tabular}{p{0.2\linewidth}|p{0.1\linewidth}|p{0.1\linewidth}|p{0.1\linewidth}|p{0.35\linewidth}}
         Description & Cost & Schedule & Prob. & Mitigation Strategy\\\hline
         Radiation Damage to Screen & Minor & Minor & 3--10\% & Replace Screen/Rely on \cer measurements \\ \hline
         Permanent Radiation Damage to Cameras & Minor & Low & 10--20\% & Replace Screen/Rely on \cer measurements/increase shielding \\ \hline 
         Excessive unforeseen background & Moderate & Moderate & 3--10\% & Rely on \cer measurements/Increase shielding  \\
         \hline
         \end{tabular}
         \label{tab:risks}
\end{table}

\subsection{Responsibilities}
University College London takes responsibility for development, testing, measurement-taking and maintenance. Further engineering aspects with respect to installation and the creation of mechanical mounts and supports is handled by DESY engineers and technicians, whether employed already or will be in the future for LUXE.

\section{Cherenkov Detector}

\subsection{Human and financial resources}

The human and financial resources are estimated assuming a schedule relative to the point in time $T_0$, where funding for the LUXE experiment is released, with three years until the experiment is ready for data-taking. No explicit assumptions are made about the time of a long \euxfel shutdown.\\

Tables \ref{tab:cost_IBM} and \ref{tab:cost_EDS} list the cost of electrical and mechanical components of the IBM and EDS \cer detector systems respectively. The total cost of the two systems combined amounts to about $150\,\text{kEUR}$. Most of the hardware cost is expected to be spent during the second year after $T_0$, when equipment and components are ordered and delivered.\\

The person-power needed to complete the design, construction and software/readout design integrated over three years from $T_0$ is the following:

\begin{itemize}
    \item 3 FTE-years Post-doc (1 Postdoc FTE/yr) (detector design, readout software, testbeam campaign, supervision of students)
    \item 4 FTE-years PhD students ($2\times2/3$FTE /yr) (detector design, readout software, testbeam campaign)
    \item 0.6 FTE-years electrical/mechanical engineer (mainly required in year 1 for mechanical design, PCB design, )
    \item 0.3 FTE-years technician (mainly required for year 2 for detector assembly)
\end{itemize}
 
\begin{table}[h!]
    \centering
    \caption{Cost estimates for the IBM \cer system with 2 layers of 50 straw channels.}
    \begin{tabular}{|c|c|c|c|}
        \hline
        \textbf{Component}  & \textbf{Unit Cost (kEur)} & \textbf{Units req.} & \textbf{Total Cost (kEur)}\\\hline
         SiPMs & 0.06 & 50 & 3 \\\hline
         APDs & 0.26 & 50 & 13 \\\hline
         Readout electronics & 6.5 (32 channels) & 2 & 13 \\\hline 
         Straws & 0.005 & 100 & 0.5  \\\hline 
         PD PCB & 5 & 2 & 20 \\\hline 
         LED calibration board, fibers & 0.5 & 2 & 1  \\\hline
         cables, filters, small items & 5 & 1 & 5 \\\hline
         Slow-control and PC & 5 & 1 & 5 \\\hline
         Aluminium box & 0.2 & 1 & 0.2  \\\hline
         Gas system & 4 & 1 & 4 \\\hline\hline
         \textbf{Total} & & & 54.2 \\\hline
    \end{tabular}
    \label{tab:cost_IBM}
\end{table}

\begin{table}[h!]
    \centering
    \caption{Cost estimate for the EDS \cer system with 2 layers of 100 straw channels.}
    \begin{tabular}{|c|c|c|c|}
        \hline
        \textbf{Component}  & \textbf{Unit Cost (kEur)} & \textbf{Units req.} & \textbf{Total Cost (kEur)}\\\hline
         SiPMs & 0.06 & 100 & 6 \\\hline
         APDs & 0.26 & 100 & 26 \\\hline
         Readout electronics & 6.5 (32 channels) & 4 & 26 \\\hline 
         Straws & 0.005 & 200 & 1  \\\hline 
         PD PCB & 10 & 2 & 20 \\\hline 
         LED calibration board, fibers & 0.5 & 2 & 1  \\\hline
         cables, filters, small items & 10 & 1 & 10 \\\hline
         Slow-control and PC & 5 & 1 & 5 \\\hline
         Aluminium box & 0.5 & 1 & 0.5  \\\hline
         Gas system & 4 & 1 & 4 \\\hline\hline
         \textbf{Total} & & & 99.5 \\\hline
    \end{tabular}
    \label{tab:cost_EDS}
\end{table}

\subsection{Schedule and milestones}

Fig.~\ref{fig:cer_planning} shows an overview of the schedule and milestones for the LUXE \cer detector. The schedule for the \cer detectors is estimate until the point where the detector is ready for physics data-taking. It focuses on the EDS detector system, since this is a part of the minimal LUXE setup to take first physics measurements. Fig.~\ref{fig:cer_planning} shows the schedule with respect to $T_0$, the point in time, where the funding for LUXE is secured until three years from that point where the installation and commissioning phase is complete and the system is ready for data-taking. The first year is mainly dedicated to the finalization of the \cer detector design and test beam campaigns with a more advanced prototype with several channels and a more advanced electronics design. The second year is needed to procure the detector components, perform quality checks and to construct the full \cer detector. The first half of the third year is used to characterize the full detector, calibrate the channels and conduct the channel pre-alignment. In the second half of year three, the detector is installed and commissioned in the LUXE experimental area. For a more detailed discussion on the installation see section \ref{sec:instcommcal}.\\

%\begin{landscape}
\begin{figure}[h!]
   \centering  
    \makebox[\linewidth]{
    \includegraphics[width=1.1\textwidth]{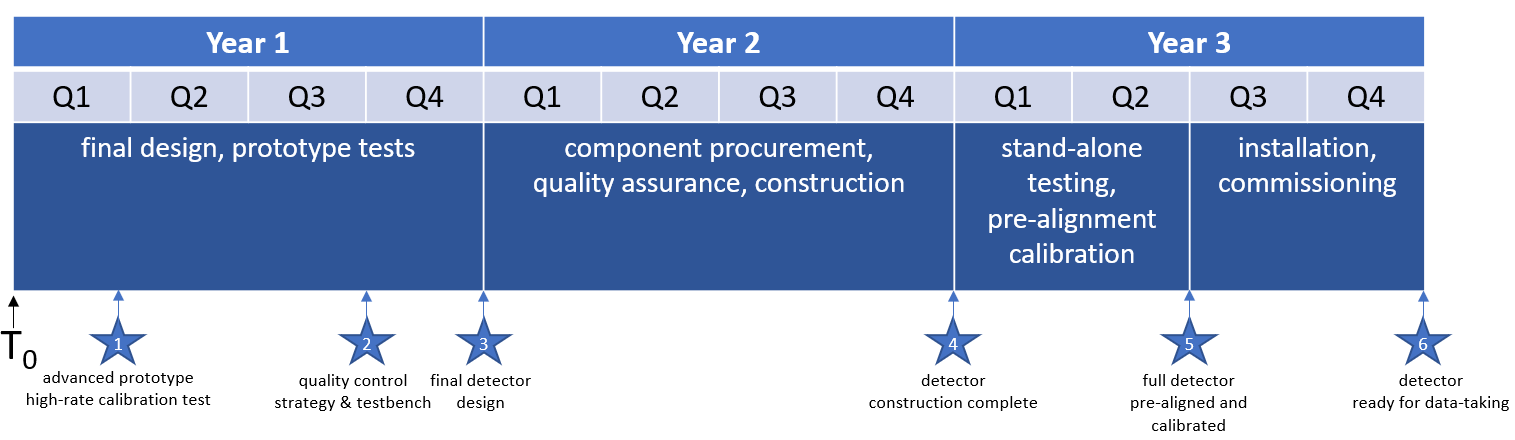}
    }
    \caption{Schedule and milestones for the LUXE \cer detector.}
    \label{fig:cer_planning}
\end{figure}
%\end{landscape}

The milestones associated with the LUIXE \cer system are:

\begin{itemize}
    \item MS 1: Calibration test with an advanced prototype at a high-rate testbeam facility. This milestone concludes the prototyping phase of the \cer detector. By testing the response of an advanced prototype with a representative and scaleable readout system at a high-statistics testbeam dataset, conclusions can be drawn if the detector design fulfils the requirements discussed in section~\ref{sec:requirements} and necessary adaptations to the design can be made if necessary.
    \item MS 2: Strategy and testbench for quality control completed. This step is necessary before orders of a large number of active components can be placed. The quality control testbench will be used to characterize the photodetectors as they arrive from the supplier.
    \item MS 3: The \cer detector design is fully completed, with all aspects of the system defined, such that orders to workshop, electronics components manufacturers etc. can be placed.
    \item MS 4: The \cer detector is fully assembled, basic funcionality tests are performed and the gas-tight box is sealed. This step is necessary to fill and start the characterization of the full detector.
    \item MS 5: The full \cer detector can be operated successfully stand-alone. All channels are pre-calibrated using LED and test beam runs and they fulfil the requirements discussed in section~\ref{sec:requirements}. The pre-alignment of the detector on its mounting structure is completed up to the required precision. The detector is ready for installation in the LUXE experimental area.
    \item MS 5: The detector is installed in the LUXE experimental area. Commissioning without beam is concluded. The detector is ready for beam-based commissioning. For a more detailed discussion of the steps needed during installation and commissioning, see section \ref{sec:instcommcal}.
\end{itemize}

\subsection{Risk management}

The risks to the LUXE \cer detector project associated with the Milestones above are estimated based on the following scale:

\begin{itemize}
    \item Insignificant: Risk is easily mitigated by day to day process. 
    \item Minor: Delays up to 10\% of schedule. Cost increase up to 10\% of budget. 
    \item Moderate: Delays up to 30\% of schedule. Cost increase up to 30\% of budget. 
    \item Major: Delays up to 50\% of schedule. Cost increase up to 50\% of budget. 
    \item Catastrophic: project abandoned
\end{itemize}

The probability of a risk to be realized is quantified as, rare: ($<3$\%), unlikely (3-10\%), moderate (10-50\%), likely (50-90\%) or certain ($>90\%$).\\

Table \ref{tab:risks} lists the risks associated with the milestones foreseen for the LUXE \cer detector system. Since Milestone I (low-rate TB with detector prototype) has been reached at the time of compiling the technical note, the risk assessment starts with Milestone II. Since the design of LUXE on purpose foresees two complementary detector technologies for the EDS and IBM systems (Scintillator screen and \cer detectors) no catastrophic risk to the LUXE experiment could be identified.\\

\begin{table}[htb!]
    \centering
    \caption{Risk description, potential impact on cost and schedule, probability to occur and strategy on how to mitigate the risk.}
\begin{tabular}{p{0.2\linewidth}|p{0.12\linewidth}|p{0.12\linewidth}|p{0.12\linewidth}|p{0.35\linewidth}}
        \hline
        \textbf{Description} & \textbf{Cost} & \textbf{Schedule} & \textbf{Prob.} & \textbf{Strategy}\\\hline
         \multicolumn{5}{c}{\textbf{Milestone 1: Advanced Prototype high-rate test}} \\\hline
         Delay in prototype construction & Insignificant & Moderate & Moderate & assign enough person-power \\\hline
         Suitable TB facility not available & Insignificant & Moderate & Moderate & apply for beam time early, at several places \\\hline
         \multicolumn{5}{c}{\textbf{Milestone 2: Electrical components test bench and routine}} \\\hline
         Delayed past order arrival & Minor & Minor & Moderate & assign enough person power \\\hline
         \multicolumn{5}{c}{\textbf{Milestone 3: Final detector design}} \\\hline
         Suboptimal design noticed late & Moderate & Moderate & Moderate & early engineering review, thorough beam tests with realistic prototype\\\hline
         \multicolumn{5}{c}{\textbf{Milestone 4: Detector construction}} \\\hline
         Delay in order of electrical components & Moderate & Moderate & Moderate & foresee enough time in planning \\\hline
         Electrical components failure & Minor & Minor &  Likely & establish quality control, order feasible amount of spares, exchange-friendly design \\\hline
         \multicolumn{5}{c}{\textbf{Milestone 5: Charge calibration}} \\\hline
         Detector construction delayed & Insignificant & Minor & Moderate & can do in-situ in LUXE experimental area\\\hline
         \multicolumn{5}{c}{\textbf{Milestone 6: Installation and Commissioning}} \\\hline
         Critical component failure unnoticed & Moderate & Minor & Unlikely & frequent functionality tests, exchange-friendly design  \\
         \hline
         \end{tabular}
         \label{tab:risks}
\end{table}

\subsection{Responsibilities}
The responsibility and human resources for the development, construction and installation of the \cer system will be taken by DESY Hamburg. Certain aspects of the construction and installation in the experimental area require access to central DESY services, such as mechanical and electronics workshops, electrical and gas system installations in the experimental area as well as lifting the detector systems into the LUXE area by crane. In addition the use of DESY test beam facilities is foreseen as a part of the detector development and calibration process.\\

\section{Gamma Spectrometer}
%\section{Project organisation}

We are aiming at starting installation during one of the longer planned shutdown of the EuXFEL operations. In Table~\ref{manpower}, a breakdown of required human resources is given for the different stages of preparation (Years -2 and -1), installation (Year 0), and data acquisition (Years 1,2, and 3). The available funding is shown assuming installation in 2025  and is currently obtained mainly via support of a national research council, the Engineering and Physical Science Research Council (EPSRC) in the UK. 

\begin{table}[t!]
\centering
\begin{tabular}{|l||c|c|c|c|c|c|}
\hline
\textbf{Human resource } & \textbf{Year -2} & \textbf{Year -1} & \textbf{Year 0} & \textbf{Year 1} & \textbf{Year 2} & \textbf{Year 3}  \\
\hline
\hline
PhD FTE & 1 & 1 & 1 & 1 & 1 & 1 \\
\hline
Post-doc FTE  & 1 & 1 & 1 & 1 & 1 & 1 \\
\hline
Senior scientist FTE & 0.2 & 0.2 & 0.2 & 0.2 & 0.2 & 0.2 \\
\hline
\hline
 \multicolumn{7}{|r|}{ \textbf{\centerline{\emph{Funding secured (assuming 2025 as Year 0)}}}} \\
\hline
PhD FTE & 0.5 & 0.5 & 0 & 0 & 0 & 0 \\
\hline
Post-doc FTE  & 0.5 & 0.5 & 0.5 & 0 & 0 & 0 \\
\hline
Senior scientist FTE & 0.1 & 0.1 & 0.1 & 0 & 0 & 0 \\
\hline
\hline
\end{tabular}
\caption{FTE requested for the preparation, installation, and running of the gamma-ray spectrometer in LUXE. Secured funding is shown in the bottom half of the table, assuming installation in 2025.}
\label{manpower}
\end{table}

Several milestones can be identified to reach a final version of the spectrometer to be installed in LUXE. The analysis and deconvolution algorithms have already been finalised and tested both numerically and experimentally at two proof-of-principle experimental campaigns carried out using the Astra-Gemini laser at the Central Laser Facility in the UK and the Apollon laser facility in France (results are currently being prepared for publication). In both cases the spectrometer has been tested using a bright bremsstrahlung source with a variable maximum energy of the order of 1 -- 2\,GeV. Crucially, both campaigns confirmed that the converter foil does not experience noticeable degradation during sustained high-dose irradiations and that single-shot electron and positron spectra can be obtained using commercially available scintillator screens, two critical points for the successful implementation of the spectrometer within LUXE.

The second step of the project will be the design and construction of the dedicated vacuum chamber and the lead collimator, which is expected to be provided by the facility by the end of 2023. The dipole magnet is also expected to be available at DESY.

In summary, the main milestones of the project are:
\begin{itemize}
    \item [1.] \textbf{Algorithms and deconvolution routine}: completed.
    \item [2.] \textbf{First tests at low energy (sub-GeV)}: completed.
    \item [3.] \textbf{Tests at moderate energy (2 GeV)}: completed.
    \item [4.] \textbf{Construction of the first prototype}: to be completed by the end of 2023.
     \item [5.] \textbf{Installation, testing, and calibration}: to be completed during dedicated access.
\end{itemize}

As one can see from the list above, all the preparatory numerical modelling and experimental testing have been successfully completed, placing high confidence in the successful implementation of the detector in LUXE.

An estimate of the overall cost of the detector is given in Table~\ref{cost}. The costs breakdown  does not include the cost of the dipole magnet (expected to be available at DESY) and vacuum chamber (quotes currently been sought from vendors). An estimate of 60 k\euro for the optical elements assumes the use of optical fiber bundles; a lower cost option would consist in using relay imaging with conventional optics. The group at Queen's University Belfast will provide the scintillator screens, CCD cameras, filters, and target mounts, for an overall contribution estimated to be of the order of 66 k\euro. 

\begin{table}[t!]
\centering
\footnotesize
\begin{tabular}{|l|c|c|c|l|}
\hline
\footnotesize{\textbf{Item}} & \textbf{Cost} & \textbf{Notes} & \textbf{Responsible}  \\
\hline
\hline
\footnotesize{10 $\mu$m W foil 25x25 mm} & 0.2 & & QUB\\
\hline
interference filters & 0.8 &  & QUB\\
\hline 
scintillators with mounts & 2 &  & QUB\\
\hline
2-D motorised mount & 3 & motorisation for fine alignment & QUB\\
\hline
collimator & 5 &  & QUB\\
\hline
2 iCCD cameras & 60 &  & QUB\\
\hline
optical elements & 60 & mirrors, lenses and fibre-bundles & DESY \\
\hline
dipole magnet & TBC &  & DESY\\
\hline
vacuum chamber & TBC & & DESY\\
\hline 
\hline
\textbf{TOTAL} & \textbf{131 + TBC} & & \\
\hline
\end{tabular}
\caption{Estimate of the equipment and consumables cost of the detector. All costs are given in k\euro.}
\label{cost}
\end{table}

A risk mitigation strategy has been devised and a summary of the main risks and associated actions is given in Table~\ref{risks}. It must be noted that the advanced stage of analysis and preliminary experimental testing of the detector result in all risks to be low to moderate. 

\begin{table}[b!]
\footnotesize
\centering
\begin{tabular}{|l|c|c|c|l|}
\hline
Issue  & Probability & Impact on cost & Impact on schedule & Mitigation  \\
\hline
\hline
Difficulty in  & Low & Moderate & Low & Explore alternative \\
securing funding& & & & funding streams\\
\hline
Low signal & Low & Low & Low & Increased shielding \\
to noise& & & & and improved analysis\\
& & & & tools\\
\hline
Area unsuited & Low & Moderate & Low & Move iCCD cameras \\
for iCCD cameras& & & & in shielded area\\
& & & & upstairs with\\
& & & & longer optical path\\
\hline
Degradation of & Low & Low & Moderate & Revert to \\
fibre bundles& & & & relay imaging\\
due to radiation& & & & with conventional\\
& & & & optics\\
\hline
Degradation & Low & Moderate & Low & Use GRS  \\
of W target& & & & for dedicated runs\\
& & & & or implement\\
& & & & replacement system\\
\hline
\hline
\end{tabular}
\caption{Identified potential risks and associated mitigation strategy. }
\label{risks}
\end{table}

\section{Gamma Beam Profiler}
\label{sec:gbp:organisation}

This chapter describes the organisation, the planning and the resources needed to build, install and commission the GBP system.

Section~\ref{sec:org_int} introduces the main elements of the organisation of the project, i.e.\ the high level product breakdown structure (PBS), the management structure and the responsibility matrix.  
Then, Section~\ref{sec:org_res} describes the costs of the project, with their basis of estimate, and an evaluation of the human resources needed. Foreseen contributions from the project institutions, in terms of effort  that is expected to be available, are also reported.  Section~\ref{sec:org_sch} discusses the schedule and timeline, including a list of the main milestones.
The risks involved with the project, and the strategies to mitigate them, are dealt with  in Section~\ref{sec:org_risk}. 

\subsection{Organisation}
\label{sec:org_int}

The GBP project will be performed by a group of institutions that commit to developing, designing, constructing and installing all the components, and then to commissioning the system, running it and analysing the data it will produce.  All groups participating in the project are represented in   the GBP institute board (IB) by group representatives. The current set of institutions and groups at the time of writing this report, with their representatives,
is reported in Table~\ref{gbp:instit}.
% Table generated by Excel2LaTeX from sheet 'Sheet1'
\begin{table}[htbp]
  \centering
%  \caption{Add caption}
\footnotesize
    \begin{tabular}{l|l|l}
    \multicolumn{1}{c|}{Institution} & \multicolumn{1}{c|}{Group} & \multicolumn{1}{c}{Representative} \\
    \hline
    INFN & Bologna Section & Marco Bruschi \\
    INFN & Padova Section & Mauro Morandin \\
    The Queen's University of Belfast & School of Math. and Phys. & Gianluca Sarri \\
    \hline
    \end{tabular}%
    \caption{Institutions and their representatives in the GBP IB.}
  \label{gbp:instit}%
\end{table}%

The activities within the project are coordinated by a project leader and the project’s PBS is shown in Table~\ref{tab:wbs} with the distribution of responsibility assignments across the participating groups.
\begin{table}
    \centering
    \includegraphics[width=\textwidth]{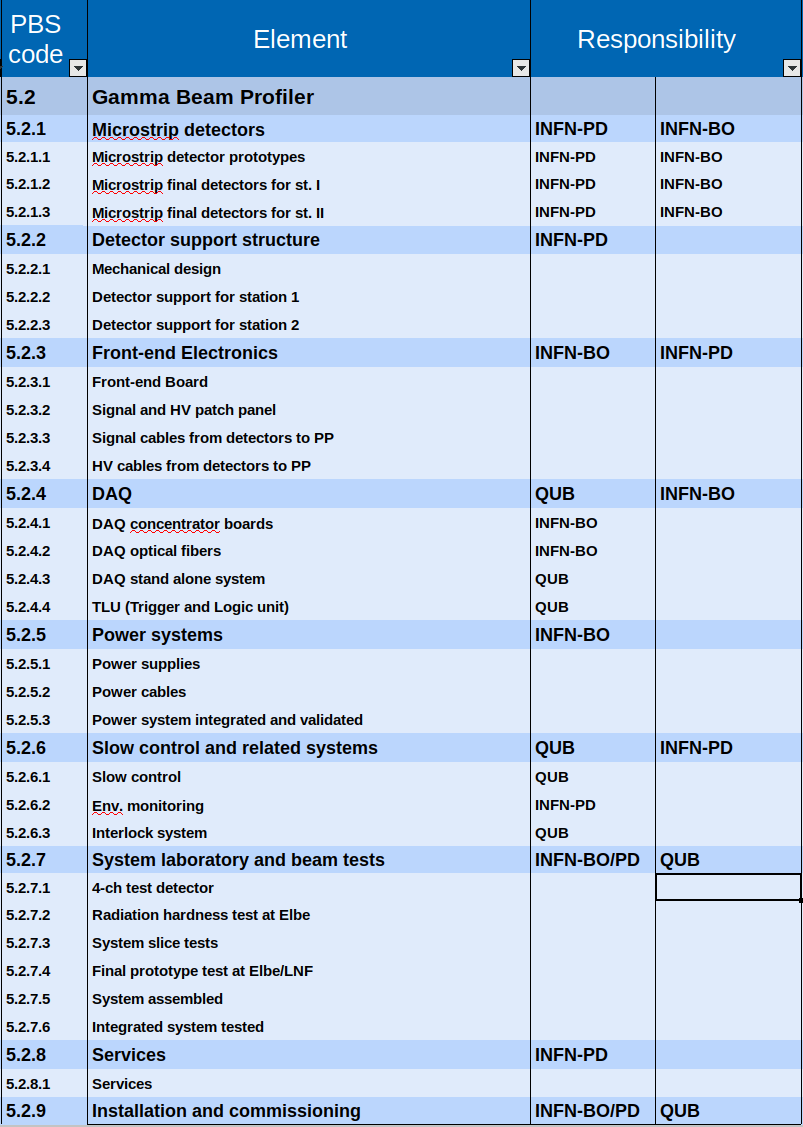}
    \caption{The level-3 GBP PBS.}
    \label{tab:wbs}
\end{table}
There are 9 entries at level-2 with the last three encompassing global deliverables of the project. At the time of writing, managers have been appointed for all the level-2 items. 
The level-2 and level-3 managers form the GBP coordination board.

Dedicated working groups have also been created, led by one or two coordinators each, that comprise experts collaborating on the key aspects of the project and report to the project leader.

The following groups have been setup:
\begin{itemize}
\item Sensors characterisation, tests and qualification process;
\item GBP sensors physics performance;
\item GBP stand-alone and global simulation.
\end{itemize}

In addition, a resource coordinator and a risk manager have been appointed. The resource coordinator maintains a database of required and pledged resources, both financial and human. The risk manager develops and maintains the risk register in coordination with
the level-2 and 3 managers. 

\subsection{Human and financial resources} \label{sec:org_res}

The estimates of the costs are explained in a basis of estimates document and Table~\ref{tab:GBP_costs} reports an overview of the costs at level-2 with the foreseen spending profile.

\begin{table}[htbp]
 \includegraphics[width=\textwidth,keepaspectratio]{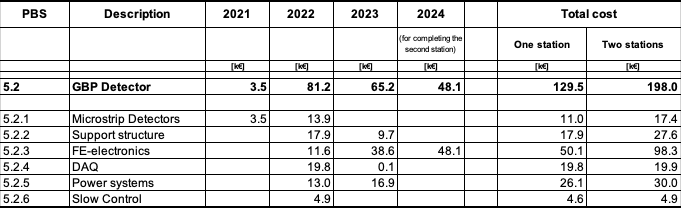}
      \caption{Estimated costs and foreseen spending profile.}
  \label{tab:GBP_costs}%
\end{table}%

The amount of resources needed to build, install and maintain the detector was originally evaluated for the years 2022--2025, assuming an installation taking place in 2024. The quantification has been performed for engineers, technicians, students (including PhD) and physicists and possible matching contributions from the various institutions have been assessed.  The  Table~\ref{tab:GBP_Resources} shows the requirements and the plausible amount of resources that institutions could provide, once the LUXE experiment has been approved.  The comparison indicates that the collaborating institutions should have sufficient resources to provide the needed effort. 

\begin{table}
    \centering
    \includegraphics[width=\textwidth,keepaspectratio]{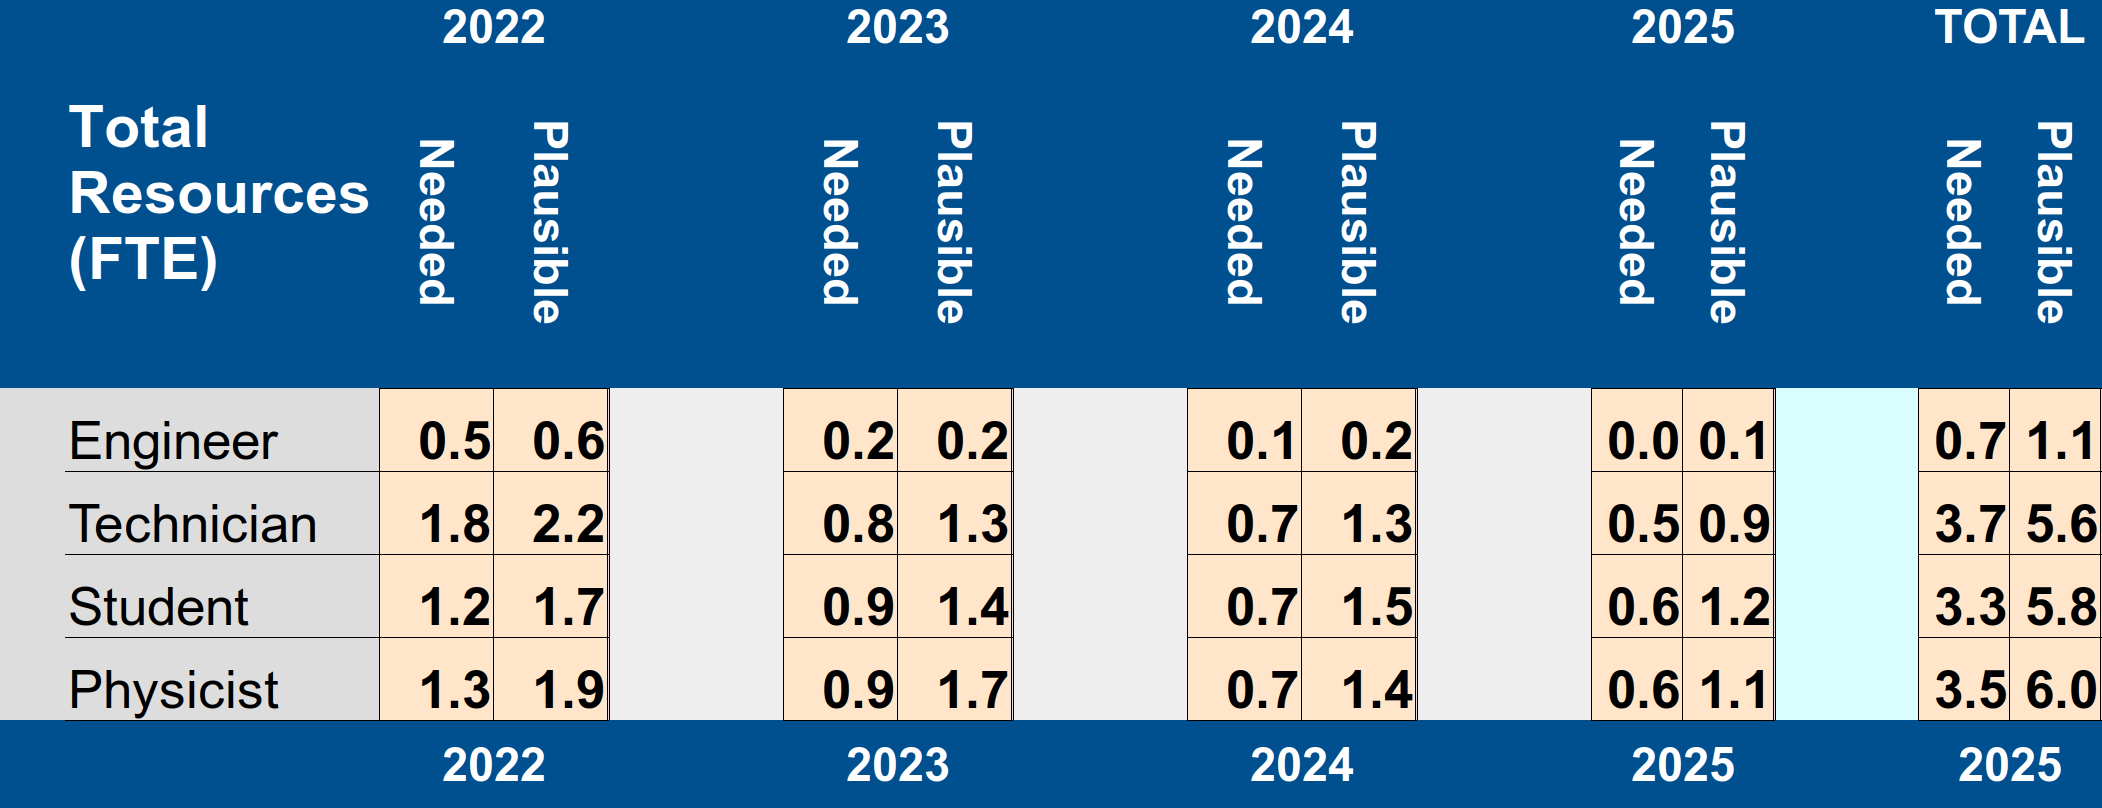}
    \caption{Estimated amount of resources needed and plausible to build, install and maintain the GBP, 2022--2025.}
    \label{tab:GBP_Resources}
\end{table}

\subsection{Schedule and milestones} \label{sec:org_sch}

A schedule for the construction and the installation of the GBP has been developed and is currently maintained as a ProjcetLibre file.  The GANNT chart illustrating the relationship among the various activities and the milestones appear in the Appendix separately for the construction phase, which is expected to be concluded in Summer 2025 and for the installation activities that are nominally taken to start in the 2025--26 shutdown. 

The main phases and milestones for the construction of the GBP are summarised in  Table~\ref{tab:GBP_milestones}.

\begin{table}[htbp]
  \centering
%  \caption{Add caption}
\footnotesize
    \begin{tabular}{l|l|c}
    \multicolumn{1}{c|}{Phase} & \multicolumn{1}{c|}{Milestone} & \multicolumn{1}{c}{Milestone date} \\
    \hline
    Prototype lab. and beam tests & Prototype validated & 30-6-2023 \\
    GBP construction & GBP ready for installation & 01-06-2025 \\
    GBP installation & GBP installed & 30-01-2026 \\
    \hline
    \end{tabular}%
    \caption{Main construction phases and milestones.}
  \label{tab:GBP_milestones}%
\end{table}%

\subsection{Risk management} \label{sec:org_risk}

Management of the risk is performed through the regular update of a risk register in which risks are classified for their impact: 

\begin{itemize}
    \item Irrelevant: Risk is easily mitigated by day to day process. 
    \item Minor: Delays up to 10\% of schedule. Cost increase up to 10\% of budget. 
    \item Moderate: Delays up to 30\% of schedule. Cost increase up to 30\% of budget. 
    \item Major: Delays up to 50\% of schedule. Cost increase up to 50\% of budget. 
    \item Catastrophic: project abandoned
\end{itemize}

and for the probability of realisation as follows:   rare ($<3$\%), unlikely (3-10\%), moderate (10-50\%), likely (50-90\%) or certain ($>90\%$).

In Table~\ref{tab:GBP_RR} the main risks are reported, together with their mitigation strategy. 

\begin{table}
    \centering
    \includegraphics[width=\textwidth,keepaspectratio]{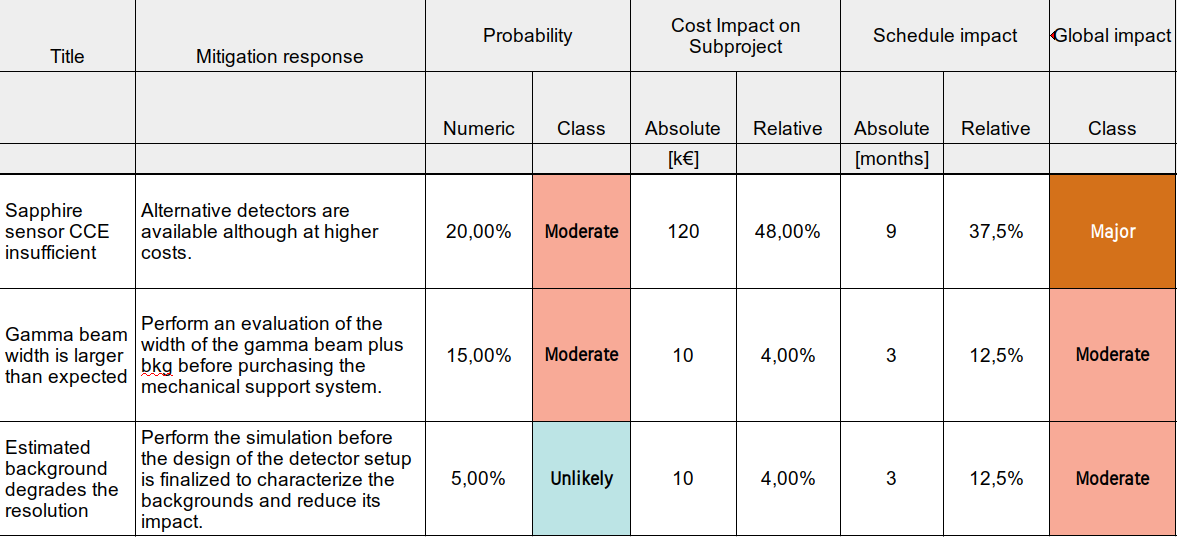}
    \caption{Risk description, mitigation strategy, probability to occur, cost and schedule impact.}
    \label{tab:GBP_RR}
\end{table}

The most critical risk is related to the possibility that the charge collection efficiency (CCE) of the sapphire sensors turns out to be significantly lower than the values extrapolated from previous measurements or that the CCE is not uniform across the sensors. The first possibility was ruled out with the first tests carried out at the INFN LNF in 2022 and described in this document.  Measurements to demonstrate the necessary CCE uniformity will be carried out in 2023.  In the worst case, it will be possible to replace the sapphire sensors with diamond microstrip detectors that have been successfully used as particle detectors in extremely high radiation environments. They represent a solid backup solution, though the costs would be higher, since the diamond wafers are more expensive and we would need to replace them more frequently.  
The realisation of the second risk would cause an increase of the sensors size but without changing the number of the strips and therefore the number of electronics channels, so the impact on the total costs would be minor and it could be compensated by the lower dose absorbed.   Finally the background due to charged tracks can have an impact since the gammas convert with a very low probability inside the sapphire while possible background charged tracks always produce a signal. The countermeasure in this case would be to insert a converter in front of the GBP with the proper thickness to create electron--positron pairs that would overcome the background.  This would cause an increase of the dose absorbed by the sensors with the need of more frequent sensors replacement.

\subsection{Construction and installation schedules}

The construction and installation schedules are shown in fig.~\ref{fig:construction_gannt} and fig.~\ref{fig:installation_gannt}

\begin{figure}    \includegraphics[width=\textwidth,keepaspectratio]{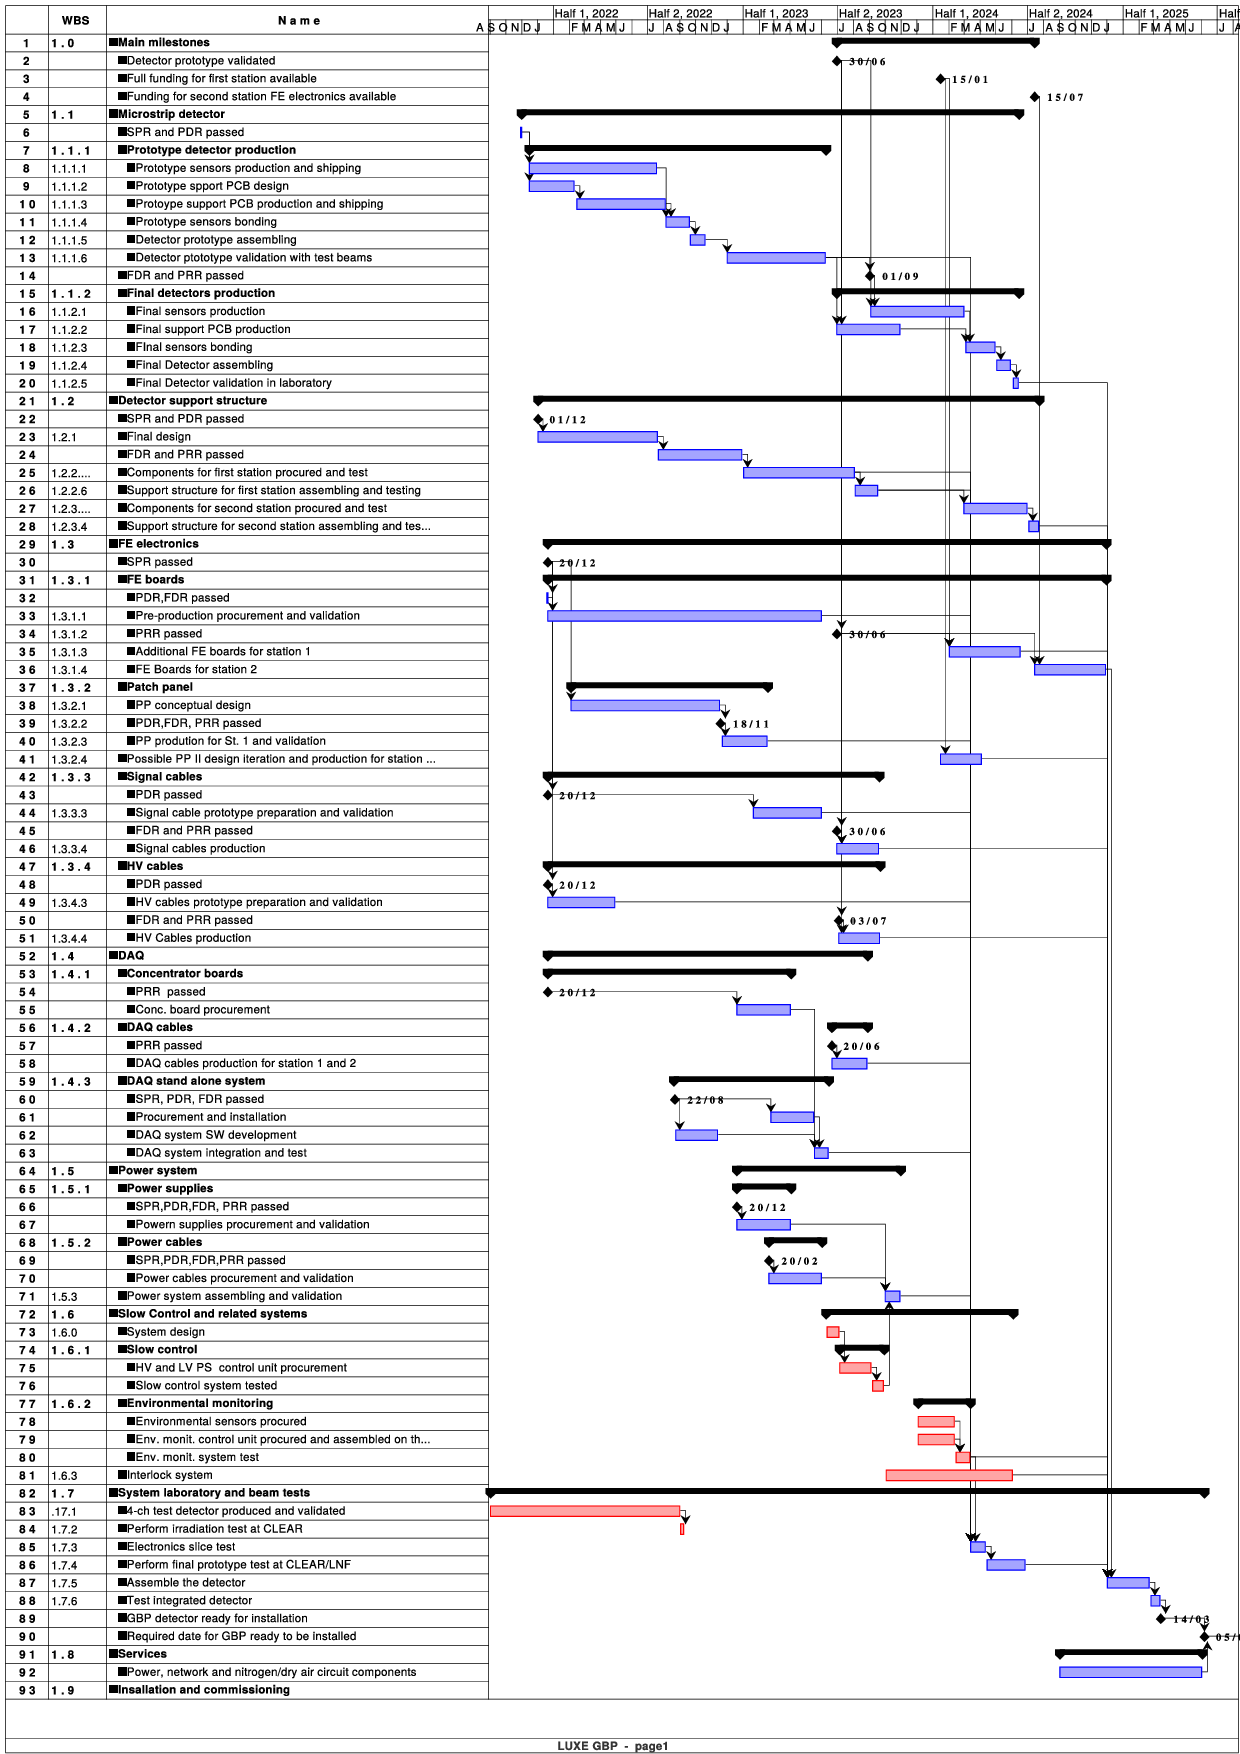}
    \caption{GBP construction GANNT chart.}
    \label{fig:construction_gannt}
\end{figure}

\begin{sidewaysfigure}    \includegraphics[width=\textwidth,keepaspectratio]{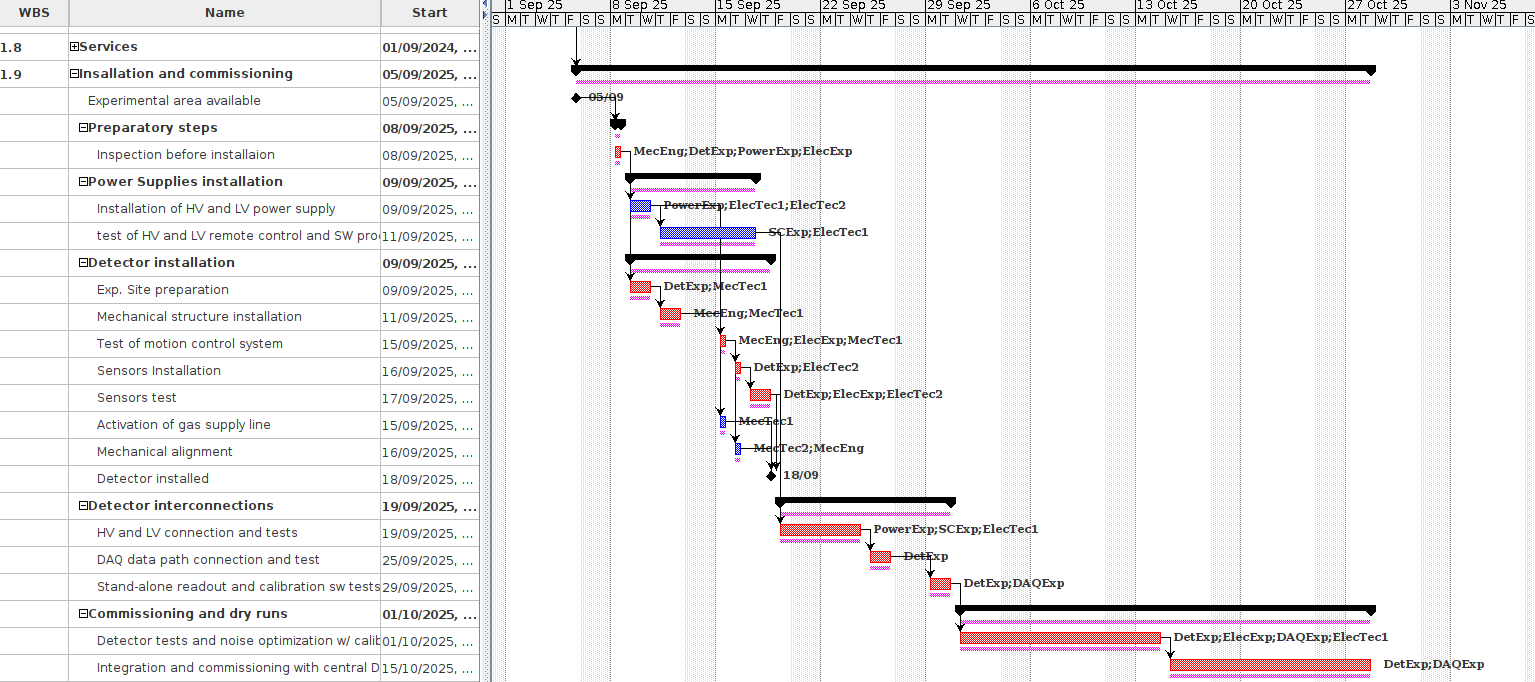}
    \caption{GBP installation GANNT chart.}
    \label{fig:installation_gannt}
\end{sidewaysfigure}

\section{Gamma Backscattering Calorimeter}

\subsection{Human and financial resources}

In terms of human resources the project requires 0.5 FTE for engineering, 1.0 FTE of a technician and 1.5 FTE of a postdoc and physicist each, integrated over 3 years (2022 -- 2024) as detailed in Table~\ref{tab:fte}.
\begin{table}
    \centering
    \caption{Summary of the FTE foreseen for the construction and installation of the LUXE GFM.}
    \vspace{0.2cm}    
    \begin{tabular}{p{2.5cm}|p{1.5cm}|p{1.5cm} |p{1.5cm}|p{1.5cm} }
         Year & 2021 & 2022& 2023 & 2024\\\hline
         Employment & existing / to hire	& existing / to hire & existing / to hire	& existing / to hire\\\hline
         Engineers  & 0/0 &	0/0.5 &	0/0	& 0/0\\
         Technicians & 0/0 &	0/0	&0/0.5&	0/0.5\\
         Physicist & 	1/0	&0.5/0&	0.5/0&	0.5/0 \\
         Postdocs & 0/0	&0/0.5&	0/0.5&	0/0.5 \\
\hline
\hline
         Sum              & 1/0	&0.5/1&	0.5/1.0&	0.5/1.0 \\ 
        \hline
    \end{tabular}
    \label{tab:fte}
\end{table}

The budget for the construction of the GFM detector is estimated and summarised in Table~\ref{tab:cost}. The price for PMTs coupled with voltage dividers comes from Hamamatsu quotations and for laser diagnostics from the ThorLabs website. QF is a quality factor (see Appendix) which quantifies the level of confidence in a price estimate.

\begin{table}
    \centering
    \caption{Summary of the budget required for the construction of the LUXE GFM, based on cost estimates for the still missing components. In addition the quality factor for each component and the average QF in the last line are given.}
    \vspace{0.2cm}
    \begin{tabular}{ p{4.5cm}|p{1.9cm}|p{0.8cm}|p{3cm} }
        Component  & Cost (kEur) & QF &Comment\\\hline
         Mechanical frame & 5 & 5& DESY\\
         Lead Glass blocks  & free & 0 & Available\\
         8 PMTs, 8 voltage dividers & 12 &2 & For 1 or 2 PMTs the QU Fund could be used, for others - N/D \\
         CAEN V1730SB 16/8 Channel 14 bit 500 MS/s Digitizer & 15 & 0 & Available\\
         Diagnostic Laser diode and Laser driver, fibers & 10 & 3 & N/D \\ 
         DAQ hardware, power supplies, cables, PCBs & 5 & 1 &  HV is available, others - N/D \\
         Tooling    & 10&3 & DESY \\
\hline
\hline
         Sum              & 57 &   2 &        \\\hline
    \end{tabular}
    \label{tab:cost}
\end{table}

\subsection{Schedule and milestones}

The readiness for installation is planned for January 2024. But it can fit in all three LUXE scenarios.
The global milestones for the GFM are (Fig.~\ref{fig:GM_milestones}):

\begin{enumerate}
    \item Finalise the design by February 2022;
    \item Assemble a detector module prototype by August 2022;
    \item Test the advanced detector module prototype by the end of 2022;
    \item Assemble the full detector and install by the forth quarter of 2023;
    \item Commission by first quarter of 2024.
\end{enumerate}

\begin{figure}[ht!]
  \begin{center}
    \includegraphics[width=0.9\textwidth]{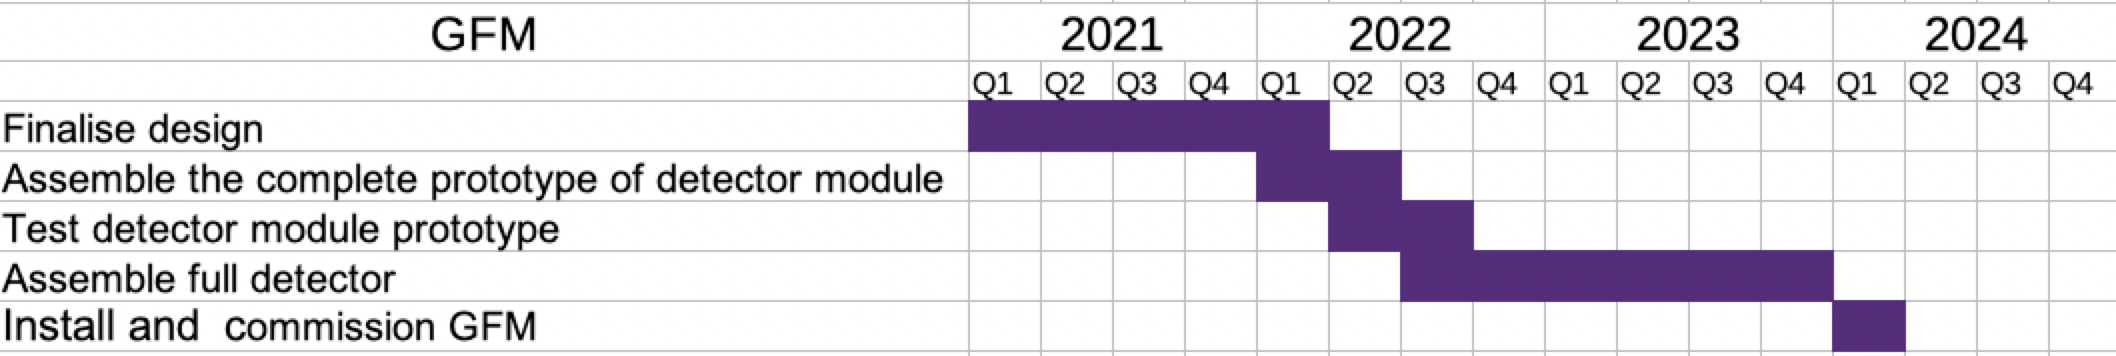}
      \end{center}
    \caption{Milestones and timeline for the GFM delivery and installation.}
    \label{fig:GM_milestones}
\end{figure}

\subsection{Risk management}
This section discusses the main risk factors, how/if they impact cost and/or schedule, their probability and how they are mitigated.  There are two dimensions, the impact and the probability. We separate the impact on the cost and on the schedule and use the following terms for impact risks:

\begin{itemize}
    \item Insignificant: Risk is easily mitigated by day to day process;
    \item Minor: Delays up to 10\% of the schedule. Cost increase up to 10\% of budget;
    \item Moderate: Delays up to 30\% of the schedule. Cost increase up to 30\% of budget; 
    \item Major: Delays up to 50\% of schedule. Cost increase up to 50\% of budget;
    \item Catastrophic: project abandoned.
\end{itemize}

The probability of a risk to be realised is quantified as, rare: ($<3$\%), unlikely (3--10\%), moderate (10--50\%), likely (50--90\%) or certain ($>90\%$). 

\begin{table}[]
    \centering
    \caption{Risk description for the GFM, potential impact on cost and schedule, probability to occur and strategy on how to mitigate the risk.}
\begin{tabular}{p{0.2\linewidth}|p{0.15\linewidth}|p{0.1\linewidth}|p{0.1\linewidth}|p{0.25\linewidth}}
         Description & Cost & Schedule & Prob. & Strategy\\\hline \hline
         Not radiation hard crystals &Insignificant &Minor &Moderate & Exchange-friendly design\\\hline
         Sub-optimal design identified in TB&Minor &Minor &Unlikely& Detailed simulation; use tested existing technologies wherever possible\\    \hline  
         Full detector: components failure&Insignificant &Minor &Unlikely & Develop components testing procedure in the lab before assembly. Design to provide for easy exchange of faulty elements.\\   \hline
         Full detector: design flaws&Insignificant &Minor &Unlikely& Detailed simulation; Build mechanical and technological prototypes in advance\\   \hline
         Installation, commissioning&Insignificant &Minor &Unlikely& Exchange-friendly design\\         
         \hline
         \end{tabular}
         \label{tab:risks}
\end{table}

Table~\ref{tab:risks} shows a summary of the risks. Considering the fact that the available crystals were stored for many years at a warehouse there was a risk, with potential high impact on schedule and cost, that because of ageing and/or sub-optimal storage they would not be in working conditions. This risk was mitigated in the recent lab and beam tests (see Section~\ref{sec:tests}).  Another risk is due to the lack of accurate information about the chemical composition of the lead-glass crystals and their radiation tolerance. Future beam-tests will clarify this aspect. The other risks mentioned in Table~\ref{tab:risks} can be easily mitigated and have no impact on the cost or schedule of the LUXE experiment.

\subsection{Responsibilities}
The responsibilities are shared by one senior physicist from KINR, Ukraine and the LUXE group at DESY. The work concerning simulation, \geant and MC, documentation, lab tests and beam-tests are the responsibility of the physicist from KINR and starting from 2022 also one postdoc employed by the LUXE team at DESY. 
In 2022 the engineering drawings of the detector (CAD model) will be produced with the help of an engineer from DESY.
To produce the supporting structure, technical support will be required but can be outsourced.
The help from technicians and the lab space at DESY will be needed to assemble the detector. 

\section{Data Acquisition, Computing \& Simulation}
\label{sec:organisation}

\subsection{Human and financial resources}

\subsubsection*{DAQ, DQM and slow control system costs}
The following human resources are required for delivery of the DAQ, DQM and slow control systems.  The costs associated with the DAQ hardware are given in Table~\ref{tab:cost}.

\begin{itemize}
    \item 0.2 FTE/yr physicist for oversight and communication with detector responsibles.
    \item 0.3 FTE/yr physicist/engineer for technical work, responsible for timing and synchronisation (TLU).
    \item 1 FTE/yr post-doc/engineer for DAQ software, EUDAQ2 (including DQM).
    \item 0.5 FTE/yr PhD student to support above, particularly software.
    \item Some effort for the DQM software is included in the full-time DAQ software post and some effort for the slow control system is included in the full-time common software post.  We therefore estimate that a further 0.5 FTE/yr physicist/engineer is needed to also work on the slow control and DQM systems for development and redundancy.
\end{itemize}

It is assumed that for completion of the DAQ system, the above effort is required for 3\,years.  Once data-taking starts, the above effort is expected to be reduced by 50\%.  Effort will be required for maintenance, new developments and on-call activities.  It is expected that data taking will be covered by a shift system and so expert help will not be constantly required.

\begin{table}[]
    \centering
    \caption{Cost estimates for the DAQ hardware. The comment discusses the source of the price.}
    \begin{tabular}{|l|c|c|c|l|}
        \hline
        Component  & Quantity & \vtop{\hbox{\strut Unit cost} \hbox{\strut (kEur)}} & \vtop{\hbox{\strut Total cost} \hbox{\strut (kEur)}} & Comment\\\hline
%%%        TLU & 4 & 4 & 16 & \vtop{\hbox{\strut From recent} \hbox{\strut production}}\\ \hline
        TLU & 15 & 3.3 & 50 & \vtop{\hbox{\strut From recent} \hbox{\strut production}}\\ \hline
        Fanout & 4 & 2 & 8 & --\\ \hline
        DAQ PC & 2 & 1 & 2 & PC costs\\ \hline
        Storage buffer & 1 & 20 & 20 & DELL website \\ \hline
    \end{tabular}
    \label{tab:cost}
\end{table}

\subsubsection*{Computing and software costs}
The following human resources are required for support of the common computing infrastructure and software:
\begin{itemize}
    \item 0.5 FTE/yr physicist for oversight, organisation of the procurement of storage and computing resources in conjunction with DESY IT, and communication with detector responsibles.
    \item 0.5 FTE/yr physicist/engineer to develop and maintain the LUXE simulation.
    \item 0.5 FTE/yr physicist/engineer for technical work on computing, grid, etc.
    \item 1 FTE/yr physicist/engineer for technical work on the common software. These responsibilities include for example the design, implementation and maintenance of a conditions database, and the maintenance of the combined positron reconstruction from the tracker and calorimeter inputs.
    \item 0.5 FTE/yr physicist/engineer dedicated to the development and maintenance of an overall software framework for the experiment.
\end{itemize}
The above effort is initially required for 3\,years until data taking starts.  At the start of data taking, a similar level of effort will be required, although it is expected that some aspects will be covered by PhD students. 

No costs are expected for the distribution of LUXE software, which will use freely-available public repositories\footnote{\url{https://github.com/LUXEsoftware}}. 

The expected costs for the storage of data and MC simulated events is summarised in Table~\ref{tab:computing_storage_costs}, assuming no compression for the data from the cameras and laser diagnostics.

The estimated cost for robust storage resources (i.e.\ backed-up disks or tapes) is of 50~\euro/TB on disk and 16.5~\euro/TB on tape. 

\begin{table}[hbt]
    \centering
    \caption{Size estimates for the various data formats per year of operation, assuming robust disk- or tape-based storage and the maximum event size for data events at a single site.}
    
    \begin{tabular}{|l|c|c|c|}
        \hline
        Type of data                   & \vtop{\hbox{\strut Data size} \hbox{\strut (PB)}}  & \vtop{\hbox{\strut Disk cost} \hbox{\strut (kEur)}} & \vtop{\hbox{\strut Tape cost} \hbox{\strut (kEur)}} \\
        \hline
        Raw data (filled BX)           & 0.46      & --  & 7.8 \\
        Raw data (empty BX)            & 0.01      & --  & 0.2 \\
        Reconstructed data & 0.40   & 50  & -- \\
        \hline
        Simulated data (1:1 filled BX) & 0.54      & 70  & -- \\
        \hline
        Total                          & 1.42      & 120 & 8.0\\
        \hline
    \end{tabular}
    \label{tab:computing_storage_costs}
\end{table}

\subsection{Schedule and milestones}

The 3-year schedules for the DAQ system, DQM and slow control systems and the computing and hardware is shown in Fig.~\ref{fig:DAQ-schedule}.

\begin{figure}[hbt]
\centering
    \includegraphics[trim={1.5cm 11cm 5.cm 1.5cm},clip,width=0.99\textwidth]{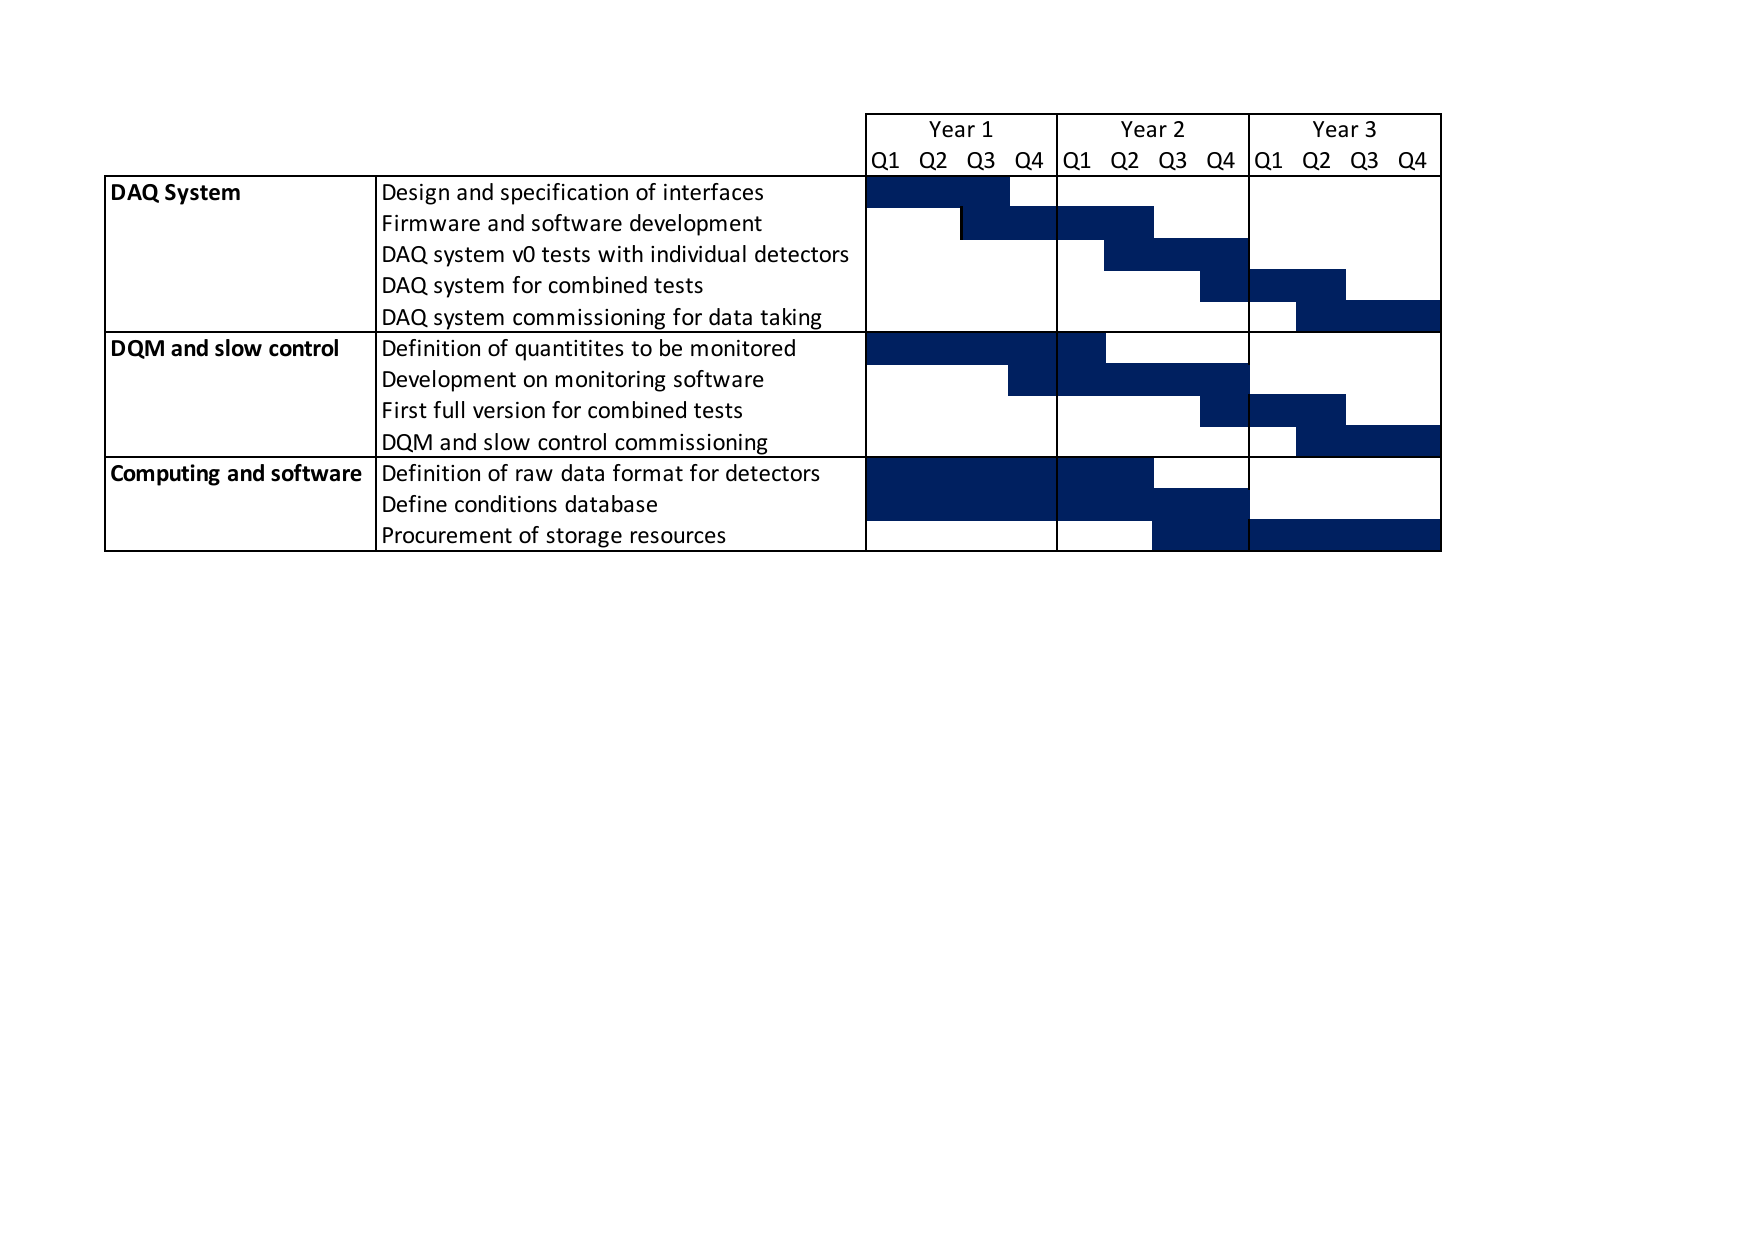}
    \caption{Schedule.}
    \label{fig:DAQ-schedule}
\end{figure}

%%% Computing milestones (to be included in the figure):
%%% \begin{itemize}
%%%    \item End 2022: Definition of RAW data byte-stream format for the LUXE detectors
%%%    \item 2022-2023: Design and implementation of data-taking conditions database 
%%%    \item End 2024: Procurement of initial storage resources
%%% \end{itemize}

\subsection{Risk management}

The major risk for each subject is given in Table~\ref{tab:risks} and discussed below.

It is expected that the simulation will undergo updates and improvements, even during data taking.  A risk is that the simulation is not of sufficient accuracy for the start of data analysis.  This will lead to possible delays in the first results and/or less precise measurements, but should not affect the start-up of the experiment.  To mitigate this, parts of the simulation need to be prioritised.

The main risk for the DAQ is that all systems are not fully integrated.  To try and ensure this does not happen, integration has started early, both testing in the lab and in beam tests.  The TLU has been used already by several detectors, as has EUDAQ2 and work continues.  Should this risk be realised, it would mean a slip in the schedule and the costs would be the extra effort needed to ensure integration is done within an extra 6\,months.  This may result in more work needed offline to ensure that the data is merged correctly.

The DQM and slow control monitoring require  software and the implementation of the checks within the software.  Delays in their operation may lead to delays in data taking or less efficient data taking as safe and continuous operation is not possible.

Computing risks are related to possible failures of computing hardware.  As the PCs, networks, etc.\ will make use of standard equipment, then (average) failure rates will be known and spares should be readily available.

The most important risk related to the software development affects the implementation of the detector condition database, which is required to be completed before the start of the data taking. Delays in the implementation might lead to loss, or poor quality of the reconstructed data.

Other minor risks affecting software development are related to the potential lack of a coherent software framework at the start of the data taking, because of the limited person power that will be available in this field. This can generally lead to poorly efficient workflows. The likelihood is considered to be relatively high. It is not expected to have an impact on the quality of the results released by the experiment, but rather on their timeliness.

\begin{table}[h]
    \centering
    \caption{Risk for the DAQ: description, potential impact on cost and schedule, probability to occur and strategy on how to mitigate the risk.}
\begin{tabular}{|p{0.22\linewidth}|p{0.12\linewidth}|p{0.1\linewidth}|p{0.12\linewidth}|p{0.3\linewidth}|}
         \hline
         Description & Cost & Schedule & Prob. & Strategy\\\hline
         Simulation not accurate & 0 kEUR & 0.0 & Moderate & Prioritise parts of simulation. \\ \hline
         Not all systems integrated in DAQ & 50 kEUR & 0.25 & Moderate & Start early.  May need extra integration offline. \\ \hline
         Slow control and/or DQM not ready & 50 kEUR & 0.25 & Moderate & Start early.  May need to do more manual checks. \\ \hline
         Conditions database not ready & 50 kEUR & 0.25 & Moderate & Start early. Decide on a minimum set of conditions. \\ \hline
         Integration in  software framework not complete & 0 kEUR & 0.0 & High & Choose well-known framework. \\
         \hline
         \end{tabular}
         \label{tab:risks}
\end{table}

\subsection{Responsibilities}

Each of the discussed activities has the following institutes taking responsibility for them.

\subsubsection*{DAQ, DQM and slow control systems}

\begin{itemize}
    \item \textbf{DAQ:} Primary responsibility lies with UCL, with contributions from DESY and also other institutes developing detectors.
    \item \textbf{DQM:} This is coordinated by UCL, with input from other institutes developing detectors.
    \item \textbf{Slow control:} Primary responsibility lies with DESY, with input from UCL.
\end{itemize}

\subsubsection*{Computing and software costs}

\begin{itemize}
    \item \textbf{Simulation:} The primary coordinating institute is DESY, but contributions are needed from sub-detector groups. 
    \item \textbf{Computing:} This is the responsibility of DESY.
\end{itemize}

\section{Technical Infrastructure}
\label{app:orga_technicalinfra}

\subsection{Human and financial resources}
\label{sec:ressources}

The human and financial resources are estimated assuming a schedule relative to the point in time $T_0$, where funding for the LUXE experiment is released, with more than three years until the experiment is ready for data-taking. No explicit assumptions are made about the schedule at which a long \euxfel shutdown could happen.\\

The cost model is made such that one separates core invest and material costs (in kEUR) and person power (in FTE) that is assumed to come from local resources (i.e. DESY groups, M or FH). The core invest estimates are based on (preliminary) quotes from vendors or on experience from experts at DESY. The estimates of the person power requirements come from experts. Overheads, escalation or contingency are not included. 

In the LUXE CDR~\cite{luxecdr}, different work packages were introduced to describe the deliverables needed by the experiment. The financial resources are based on a similar structure. Each estimate come with a confidence level index, 1 being the most reliable and 4 being the least reliable:

\begin{itemize}

      \item Confidence level 1:  Quote from a company

      \item Confidence level 2: Preliminary estimate from experts

      \item Confidence level 3: Preliminary estimate after consultation with experts

      \item Confidence level 4: Less reliable estimates, based on other methods

\end{itemize}  

Table~\ref{TC:Annex:Resources_WP61} shows the financial resources for the workpackage 1.1, technical coordination - outside building, which summarises the costs associated to the new building and the infrastructure that will need to be constructed outside of XS1. 

\begin{landscape}% Landscape page
\begin{table}[h]
\small
\begin{tabular}{lp{50mm}llp{50mm}}
\hline
Item 	                & Description  																	& Res. (kE) & Confidence  & Comments \\
\hline 
\hline

\hline
1 New outside building 					& Container building, contains lab space for clean room (100m2), service room (20m2),  and offices (control room, etc..) (180 m2)									&  995 		 		  &    2 	    & Based on discussion with Denny Drossmann, engineer responsible for design and construction of Innovation Village: 1.95kE/m2 for office and 6.05kE/m2 for lab (price taking into account inflation to beginning of 2022)\\      
\hline     
2 CR computers and desk equipment     & Computer and desk equipment for experimental control room in surface building of XS1				&  10 				  &    3 	     & Numbers estimated from survey of computers, screens,.. in IBISS  \\
  
\hline 
3 Electrical cabinet in surface building 		& Cabinets to host back-end electronics											&  25 		 		  &    3 	 	& 5keuros per cabinet (5 pieces), estimated with Daniel Thoden (engineer MEA)  \\

\hline 
\hline
\end{tabular}
\caption{Resources required for workpackage 1.1, technical coordination - New building. Confidence rules:1 - Quote from a company; 2 - Preliminary estimate from experts; 3 - Preliminary estimate after consultation with experts;4 – Less reliable estimates, based on other methods.}
\label{TC:Annex:Resources_WP61}
\end{table}
\end{landscape}% Landscape page
% \end{adjustwidth}

% \newpage

Table~\ref{TC:Annex:Resources_WP62} shows the financial resources for the workpackage 1.2, technical coordination - Installation/Experiment, which summarises item related to the electron beam-line. 

\begin{landscape}% Landscape page
\begin{table}[h]
\tiny
\begin{tabular}{lp{50mm}llp{50mm}}
\hline
Item 							    & Description  																	& Res. (kE) & Confidence   & Comments \\
\hline 
\hline                                                                                                                                      
1 Electron beam line 				& Including equipment (monitor, pumps,etc...)									&  300 		 		  &    2 	    & Machine experts said that beam line with instrument is 10k/m (assuming 30m)  \\      
\hline
          
2 Dumps 							& HICS dump and photon dumps													&  300		 		  &    2	 	& Machine experts said that one dump is around 100k. \\
\hline

3 Experimental dipoles 				& 3 experimental dipoles (target, IP, gamma spectrometer)						&  390		 		  &    1	 	& Quote from Efremov institute Dec. 2021 for 3 TDC magnets.\\
\hline

4 Dipole power supplies 			& Power supplies to power TDC magnets.											&  105		 		  &    1	 	& Discussion with MKK. Each HVPS would be ~35k. \\
\hline

5 Dipole cabling+ cooling			& services to TDC magnets														&  150		 		  &    4	 	& extrapolated from machine CDR. \\

\hline

6 Magnet support and adjustment plate			& 8k/pieces												         	&  24		 		  &    2	 	& Discussion with K. Gadow (FH engineer). \\

\hline

7 IP Chamber gate valve +control system			& IP Chamber gate valve +control system														&  50		 		  &    2	 	& Estimate from Matt Zepf. \\

\hline

7(bis) IP Chamber vacuum tank			&  Taken into account in Laser note! Shown here for information! Not accounted for in our pricing.														&  40		 		  &    2	 	& Estimate from K. Gadow(FH engineer) \\

\hline

8 Target vacuum chambers			& 20k each, chambers with movable targets													&  40		 		  &    2	 	& Discussion with K. Gadow(FH engineer). \\

\hline
\hline
\end{tabular}
\caption{Resources required for workpackage 1.2, technical coordination - Installation/Experiment. Confidence rules:1 - Quote from a company; 2 - Preliminary estimate from experts; 3 - Preliminary estimate after consultation with experts;4 – Less reliable estimates, based on other methods.}
\label{TC:Annex:Resources_WP62}
\end{table}
\end{landscape}% Landscape page

Tables~\ref{TC:Annex:Resources_WP63.1} and~\ref{TC:Annex:Resources_WP63.2} shows the financial resources for the workpackage 1.3, technical coordination - service/Experiment, which summarises item related to the services needed in the experiment. 

% \newpage
\begin{landscape}% Landscape page
\begin{table}[h]
\small
\begin{tabular}{lp{50mm}llp{50mm}}
\hline
Item 							    & Description  																	& Res. (kE) & Confidence   & Comments \\
\hline 
\hline                                                                                                                                      
1 Electrical cabinet in UG02 		& Cabinets to host back-end electronics											&  10 		 		  &    3 	    & 5keuros per cabinet (2 pieces), estimated with Daniel Thoden (MEA engineer)  \\      

\hline

3 Electrical cabinet in UG03 		& Front end electronic in experimental area										&  25 		 		  &    3 	    & 5keuros per cabinet (5 pieces), estimated with Daniel Thoden (MEA engineer), probably need shielded ones...  \\   
   \hline
       
4 Gas outlet+pipes+detectors					& Gas outlet+pipes+sniffer in experimental area									&  20		 		  &    3	 	    & Discussion with Daniel Thoden (MEA engineer), and adding ~10k for gas sniffer (O2, sniffer). \\
\hline

5 Networking 		 				& Network Infrastructure to experiment 											&  70		 		  &    2	 	    & Discussion with Kars Ohrenberg (IT). Estimate valid for about 100 device connected to network. \\
\hline

6 Cooling and cabling  				& Cooling and cabling of experiment including counting room.					&  100		 		  &    3	    & Discussion with Daniel Thoden (MEA engineer) and extrapolated from Matt Zepf AC quote. \\
\hline

7 UPS						 		& Battery for emergency urgent experiment										&  15		 		  &    4	 	    & 1 Schneider electric 10kW UPS (with battery pack) that can run for 20min at full capacity. \\
\hline

\hline
\end{tabular}
\caption{Resources required for workpackage 1.3, first part, technical coordination - Service/Experiment. Confidence rules:1 - Quote from a company; 2 - Preliminary estimate from experts; 3 - Preliminary estimate after consultation with experts;4 – Less reliable estimates, based on other methods.}
\label{TC:Annex:Resources_WP63.1}
\end{table}
\end{landscape}% Landscape page

% \newpage
\begin{landscape}% Landscape page
\begin{table}[h]
\small
\begin{tabular}{lp{50mm}llp{50mm}}
\hline
Item 							    & Description  																	& Res. (kE) & Confidence  & Comments \\
\hline 
\hline  

% 8 Small optic table for detectors			& Table to hold all IP detectors.												& 15 				  &    1            & Estimated by Noam and Weiz workshop. Should be moved to detector common note.\\
\hline

8 Mechanical tray and base platform	& Detector installation structure (12 pieces, 6k each).											& 72 				  &    2            & Estimated by Noam and Weizmann workshop.\\
\hline

9 Vacuum chamber for magnets	& Chamber from magnet (2 pieces needed, 65k each)															& 130 				  &    2            & Estimated by Noam and Weizmann workshop. Compared to CDR added 2 other chambers for other magnets. \\
\hline

10 Movable stage							& Or equivalent device to move positron side tracker.									& 30 				            &    1      & Noam Quote from company. \\

\hline
11 Support structure 	& Concrete supporting elements to hold instruments, magnets, etc.				&  30 		 		  &    2     & Estimation after design made from Karsten Gadow (FH engineer)- March 2022  \\  
\hline 

12 Movable bridges 				& Way to access instruments										   &  0		 		  &    2	      & Estimation from Karsten Gadow (FH engineer).  \\
\hline 
13 Shielding 				& Concrete elements to shield beam-line								    	& 0						 		  &    2	      &  Estimation after design made from Karsten Gadow (blocks recycled) - March 2022   \\

\hline

14 Vacuum Pumps 				& Pumps for vacuum chambers								    	& 65						 		  &    1	      &  1 for each of the 5 vacuum chambers (IP, target*2, magnets*2), 13k for each quote from M.Zepf.    \\

\hline

% \hline
% 16 Pandora detectors				& 	Radiation detectors (*5, dumps,IP, electronics)			    	& ??						 		  &    2	      &  Need to be checked with Albrecht?    \\
\hline
\hline
\end{tabular}
\caption{Resources required for workpackage 1.3, second part, technical coordination - Service/Experiment. Confidence rules:1 - Quote from a company; 2 - Preliminary estimate from experts; 3 - Preliminary estimate after consultation with experts;4 – Less reliable estimates, based on other methods.}
\label{TC:Annex:Resources_WP63.2}
\end{table}
\end{landscape}% Landscape page

% \newpage

Table~\ref{TC:Annex:Resources_WP64} shows the financial resources for the workpackage 1.4, technical coordination - Infrastructure Laser, which summarises item related to the Laser infrastructure. 

\begin{landscape}% Landscape page
\begin{table}[h]
\small
\begin{tabular}{lp{50mm}llp{50mm}}
\hline
Item 							    & Description  																	& Res. (kE) & Confidence  & Comments \\
\hline
1 Laser clean room+AC						& 100 m2									&  180 		 		  &    1 	    & Quote from LOEMAT company at 1000 Euro/m2 and 800 Euros/m2(clim) .\\      
  \hline     

% 2 Clean room						& Laser clean room to be install in XS1 UG02									&  500 		 		  &    3 	    & Based on discussion with U. Schneekloth: 500 for 300m3 class 6. For class 8 would be 200 - 300. Quote from LOEMAT company at 1000 Euro/m2 and 800 Euros/m2(clim), but seems low .\\      
%   \hline
        
% 3 Air Conditioning 					& AC for Laser area																&  250		 		  &    1	 	& Company quote to M. Zepf \\

% \hline                                                                                                                1 Non permanent building						& contains clean room, service room, and control room (300 m2)									&  250 		 		  &    3 	    & Based on future discussion with Denny Drossmann innovation village .\\      
%   \hline     

% 2 Clean room						& Laser clean room to be install in XS1 UG02									&  500 		 		  &    3 	    & Based on discussion with U. Schneekloth: 500 for 300m3 class 6. For class 8 would be 200 - 300. Quote from LOEMAT company at 1000 Euro/m2 and 800 Euros/m2(clim), but seems low .\\      
%   \hline
        
% 3 Air Conditioning 					& AC for Laser area																&  250		 		  &    1	 	& Company quote to M. Zepf \\
\hline
2 Water supply 						& Installation costs															&  20		 		  &    2	 	    & estimate from M. Zepf. \\
\hline

3 Cabling supply 					& Installation costs															&  20		 		  &    2	 	    & estimate from M. Zepf. \\
\hline

4 UPS						 		& Battery for emergency urgent experiment										&  15		 		  &    4	 	    & 1 Schneider electric 10kW UPS (with battery pack) that can run for 20min at full capacity. \\
        \hline

5 Laser beam line					& Laser vacuum pipe, turbo-pump, gatevalves to go from Surface to UG03									&  108 		 		  &    2 	     & estimate from M. Zepf.\\      
        \hline
        
% 6 Vacuum Pumps 				& Pumps laser beam line							    	& 26						 		  &    1	      &  2 turbo pumps 13k each    \\
        
        %   \hline

7 Interlocks system					& Interlocks system									&  50 		 		  &    4 	     & estimate after discussion with machine experts.\\      
        \hline
% 8 Monitoring hazardous system					& Monitor hazardous things around laser.								&  ?? 		 		  &    2 	     & estimate from K. Gadow.\\      
        \hline    
  
% 2 Gamma chamber and ICS beamline 	& Vacuum chamber for ICS with beam pipe											&  15		 		  &    2	 	& 		Q1 22	&  Q4 22    & estimate from M. Zepf. \\

\hline
\hline
\end{tabular}
\caption{Resources required for workpackage 1.4, technical coordination - Infrastructure/Laser. Confidence rules:1 - Quote from a company; 2 - Preliminary estimate from experts; 3 - Preliminary estimate after consultation with experts;4 – Less reliable estimates, based on other methods.}
\label{TC:Annex:Resources_WP64}
\end{table}
\end{landscape}% Landscape page

% \newpage

% Table~\ref{TC:Annex:Resources_WP65} shows the financial resources for the workpackage 1.5, technical coordination - Installation Laser, which summarises item related to the Laser beam-lines. 

% \begin{landscape}% Landscape page
% \begin{table}[]
% \begin{tabular}{lp{50mm}llp{50mm}}
% \hline
% Item 							    & Description  																	& Res. (kE) & Confidence   & Comments \\
% \hline 
% \hline                                                                                                                                      
% 1 Laser beam line					& Laser vacuum pipe to go from Surface to UG03									&  108 		 		  &    2 	   & estimate from M. Zepf.\\      
%         \hline
  
% % 2 Gamma chamber and ICS beamline 	& Vacuum chamber for ICS with beam pipe											&  15		 		  &    2	  & estimate from M. Zepf. \\

% \hline

% \hline
% \end{tabular}
% \caption{Resources required for workpackage 1.5, technical coordination - Installation/Laser. Confidence rules:1 - Quote from a company; 2 - Preliminary estimate from experts; 3 - Preliminary estimate after consultation with experts;4 – Less reliable estimates, based on other methods.}
% \label{TC:Annex:Resources_WP65}
% \end{table}
% \end{landscape}% Landscape page

\newpage

The total capital investment cost of the infrastructure combined amounts to about $3349\,\text{kEUR}$, out of which $23\%$ falls in confidence level  1, 65\% level 2, and 6\% for levels 3 and 4 respectively.
% Most of the hardware cost is expected to be spent during the second year after $T_0$, when equipment and components are ordered and delivered.\\
A time plan for the expenditure of this capital is given by Fig.~\ref{fig:luxeinfcostmap}

\begin{figure}
    \centering
    \includegraphics[width=\textwidth]{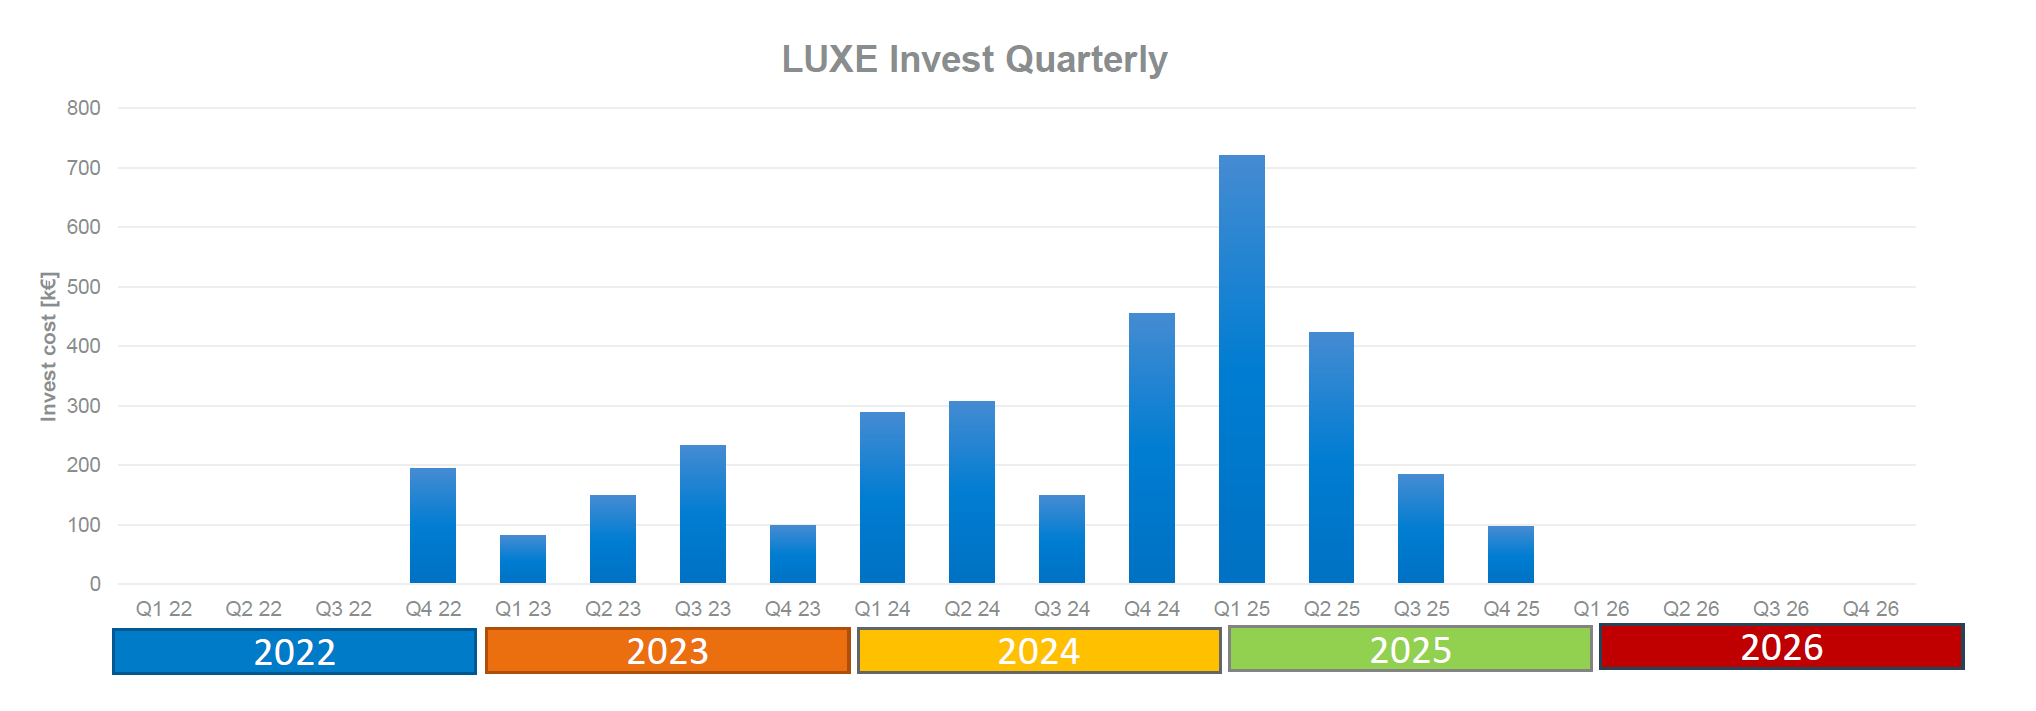}
    \caption{LUXE technical infrastructure spending profile.}
    \label{fig:luxeinfcostmap}
\end{figure}

The preliminary person-power needed to complete the design, and construction integrated over three years from $T_0$ is the following:

\begin{itemize}
    \item 5 FTE-years from M for LUXE beamline (4 (power, water, electrical, beam instrumentation)+1(interlock), charged to FH budget)
    \item 2 FTE-years for the Magnet, vacuum, dumps systems
    \item 3 FTE-years for Laser cleanroom design and the tranport line.
    \item 2 FTE-years for Detector support structures, Service room, Control room	
\end{itemize}

We are currently assuming the following FTE map for the coming years from $T_0$, flat distribution for FH, and peaking for M  for installation:
\begin{itemize}
    \item Y1: 2.34 (FH)  + 0.34 (M, LUXE)  
   \item Y Y2: 2.34 (FH) + 0.34 (M, LUXE) 
    \item YY3: 2.34 (FH) + 3.34 (M, LUXE) 
 \end{itemize}   

The different actors (DESY groups, external groups or companies) that needs to be involved to be able to deliver each of the previous items are summarized in Appendix~\ref{sec:Appendix:responsibilities}. 

\subsection{Milestones}

The schedule is given with respect to $T_0$, the point in time, where the funding for LUXE is secured until three years from that point where the installation and commissioning phase is complete and the system is ready for data-taking.

Table~\ref{TC:Annex:Milestone_WP11} shows the milestones that were determined for the LUXE workpackage 1.1, technical coordination - infrastructure.

\newcounter{mycounter}

% \begin{landscape}% Landscape page
\begin{table}[h]
\begin{tabular}{lp{60mm}cp{40mm}}
\hline
Name	&	Milestone	& Target Date	& Estimated time for completion (Months)\\
\hline\hline

IN\stepcounter{mycounter}\themycounter & Finish Support Structure Design				& Q2/Y1	 & 6 \\
IN\stepcounter{mycounter}\themycounter & Company Decision on Support structure Order	& Q4/Y1	 & 3 \\
IN\stepcounter{mycounter}\themycounter & Finish support structure construction			& Q3/Y2	 & 2 \\
IN\stepcounter{mycounter}\themycounter & Finish Shielding Design	        			& Q1/Y2	 & 6 \\
IN\stepcounter{mycounter}\themycounter & XS1 ready for beamline installation			& Q1/Y2	 & 0 \\

IN\stepcounter{mycounter}\themycounter & Finish new building Design			        	& Q3/Y1	 & 6 \\
IN\stepcounter{mycounter}\themycounter & Company Decision on new building           	& Q1/Y2	 & 6 \\
IN\stepcounter{mycounter}\themycounter & Finish support new building        			& Q1/Y3	 & 12 \\

IN\stepcounter{mycounter}\themycounter & Finish Control Room Design				     	& Q2/Y3	 & 1 \\
IN\stepcounter{mycounter}\themycounter & Finish Control Room Construction				& Q2/Y3	 & 1 \\

IN\stepcounter{mycounter}\themycounter & Outside building ready                         & Q2/Y3	 & 0 \\

\hline\hline
\hline
\end{tabular}
\caption{Major Milestones required for workpackage 1.1, technical coordination - infrastructure.}
\label{TC:Annex:Milestone_WP11}
\end{table}
% \end{landscape}% Landscape page

Table~\ref{TC:Annex:Milestone_WP12} shows the milestones that were determined for the LUXE workpackage 1.2, technical coordination - Installation/Experiment.

\begin{table}[h]
\begin{tabular}{lp{60mm}cp{40mm}}
\hline
Name	&	Milestone	& Target Date	& Time for completion (Months)\\
\hline\hline

IN\stepcounter{mycounter}\themycounter	 &	LUXE electron vacuum beamline design finalization	& Q1/Y1	& 12   \\
IN\stepcounter{mycounter}\themycounter &	LUXE electron vacuum beamline delivery				& Q4/Y2	& 3    \\
IN\stepcounter{mycounter}\themycounter &	LUXE electron vacuum beamline installed				& Q3/Y4	& 1    \\
IN\stepcounter{mycounter}\themycounter &	LUXE electron vacuum beamline running				& Q4/Y4	& 1    \\
IN\stepcounter{mycounter}\themycounter &	Electron beam dump design finished					& Q2/Y2	& 12   \\
IN\stepcounter{mycounter}\themycounter &	E-Beam Dump Received								& Q4/Y3	& 6    \\
IN\stepcounter{mycounter}\themycounter &	E-Beam Dump installed								& Q4/Y3	& 1    \\
IN\stepcounter{mycounter}\themycounter &	photon beam dump design finished					& Q2/Y2	& 12   \\
IN\stepcounter{mycounter}\themycounter &	ph-beam dump received								& Q4/Y3	& 6    \\
IN\stepcounter{mycounter}\themycounter &	ph-beam dump installed								& Q4/Y3	& 1    \\
IN\stepcounter{mycounter}\themycounter &	Magnet design finished								& Q1/Y1	& 9    \\
IN\stepcounter{mycounter}\themycounter &	Magnet Tender Decision								& Q1/Y1	& 3    \\
IN\stepcounter{mycounter}\themycounter &	Magnets received @DESY								& Q3/Y3	& 18   \\
IN\stepcounter{mycounter}\themycounter &	Magnets tested										& Q1/Y4	& 6    \\
IN\stepcounter{mycounter}\themycounter &	Magnets installed									& Q2/Y4	& 1    \\
IN\stepcounter{mycounter}\themycounter &	magnet HV system design finished					& Q2/Y2	& 9    \\
IN\stepcounter{mycounter}\themycounter &	Magnet HV system received							& Q3/Y2	& 3    \\
IN\stepcounter{mycounter}\themycounter &	Magnet HV system tested								& Q4/Y2	& 3    \\
IN\stepcounter{mycounter}\themycounter &	Magnet HV system installed							& Q1/Y3	& 1    \\
IN\stepcounter{mycounter}\themycounter &	Detector installation Plan finalized				& Q3/Y2	& 3    \\
IN\stepcounter{mycounter}\themycounter &	Receive all detectors @DESY							& Q1/Y4	& 1    \\
IN\stepcounter{mycounter}\themycounter &	Install detectors in XS1							& Q2/Y4	& 1    \\
IN\stepcounter{mycounter}\themycounter &	Finish design of Vacuum chamber						& Q3/Y3	& 9    \\
IN\stepcounter{mycounter}\themycounter &	Receive vacuum magnet chamber						& Q1/Y4	& 1    \\
IN\stepcounter{mycounter}\themycounter &	Install vacuum magnet chamber						& Q1/Y4	& 1    \\
IN\stepcounter{mycounter}\themycounter &	Fiducialisation of all items for alignment			& Q1/Y4	& 10   \\
IN\stepcounter{mycounter}\themycounter &	align experiment									& Q2/Y4	& 2 	\\

\hline\hline
\hline
\end{tabular}
\caption{Major Milestones required for workpackage 1.2, technical coordination - Installation/Experiment.}
\label{TC:Annex:Milestone_WP12}
\end{table}

Table~\ref{TC:Annex:Milestone_WP13} shows the milestones that were determined for the LUXE workpackage 1.3, technical coordination - Service/Experiment.

\begin{table}[h]
\begin{tabular}{lp{60mm}cp{40mm}}
\hline
Name	&	Milestone	& Target Date	& Time for completion (Months)\\
\hline\hline

IN\stepcounter{mycounter}\themycounter    &	Service Room Design finished	                   & Q3/Y1   &	1\\
IN\stepcounter{mycounter}\themycounter    &	Service Room Ready	                               & Q1/Y3   &	2\\
IN\stepcounter{mycounter}\themycounter    &	Final specifications of the electrical cabinets	   & Q3/Y2   &	3\\
IN\stepcounter{mycounter}\themycounter    &	electrical cabinets delivered	                   & Q4/Y3   &	3\\
IN\stepcounter{mycounter}\themycounter    &	electrical cabinets installed	                   & Q4/Y3   &	1\\
IN\stepcounter{mycounter}\themycounter    &	Finish design of electrical services	           & Q3/Y2   &	6\\
IN\stepcounter{mycounter}\themycounter    &	electrical services installed	                   & Q2/Y3   &	1\\
IN\stepcounter{mycounter}\themycounter    &	Finish Design of Cooling services	               & Q3/Y2   &	6\\
IN\stepcounter{mycounter}\themycounter    &	Colling services installed	                       & Q2/Y3   &	1\\
IN\stepcounter{mycounter}\themycounter    &	Finish design of gas services	                   & Q3/Y2   &	6\\
IN\stepcounter{mycounter}\themycounter    &	Gas services installed	                           & Q2/Y3   &	1\\
IN\stepcounter{mycounter}\themycounter    &	Finish IT services Design	                       & Q3/Y2   &	6\\
IN\stepcounter{mycounter}\themycounter    &	IT services installation	                       & Q2/Y3   &	1\\
IN\stepcounter{mycounter}\themycounter    &	DAQ installed	                                   & Q2/Y3   &	2\\
IN\stepcounter{mycounter}\themycounter    &	Detector back-end installed	                       & Q2/Y3   &	1\\

\hline\hline
\hline
\end{tabular}
\caption{Major Milestones required for workpackage 1.3, technical coordination - Service/Experiment.}
\label{TC:Annex:Milestone_WP13}
\end{table}

Table~\ref{TC:Annex:Milestone_WP14} shows the milestones that were determined for the LUXE workpackage 1.4, technical coordination - Infrastructure/Laser.

\begin{table}[h]
\begin{tabular}{lp{60mm}cp{40mm}}
\hline
Name	&	Milestone	& Target Date	& Time for completion (Months)\\
\hline\hline

IN\stepcounter{mycounter}\themycounter    &	Finish laser cleanroom specifications	 &   Q1/Y1	& 12\\
IN\stepcounter{mycounter}\themycounter    &	laser cleanroom company decision	     &   Q2/Y1	& 5\\
IN\stepcounter{mycounter}\themycounter    &	Finish laser cleanroom design	         &   Q4/Y1	& 6\\
IN\stepcounter{mycounter}\themycounter    &	cleanroom construction	                 &   Q2/Y3	& 3\\
IN\stepcounter{mycounter}\themycounter    &	cleanroom equipped	                     &   Q2/Y3	& 1\\
IN\stepcounter{mycounter}\themycounter    &	Finish Laser AC specifications	         &   Q1/Y1	& 12\\
IN\stepcounter{mycounter}\themycounter    &	Decide Laser AC company	                 &   Q4/Y1	& 3\\
IN\stepcounter{mycounter}\themycounter    &	Finish Laser AC design	                 &   Q1/Y2	& 3\\
IN\stepcounter{mycounter}\themycounter    &	Laser AC installed	                     &   Q2/Y3	& 1\\
IN\stepcounter{mycounter}\themycounter    &	Finish design of Laser transport line	 &   Q2/Y1	& 6\\
IN\stepcounter{mycounter}\themycounter    &	Laser transport line constructed	     &   Q4/Y1	& 2\\
IN\stepcounter{mycounter}\themycounter    &	Laser transport line installed	         &   Q1/Y2	& 1\\

\hline\hline
\hline
\end{tabular}
\caption{Major Milestones required for workpackage 1.4,  technical coordination - Infrastructure/Laser.}
\label{TC:Annex:Milestone_WP14}
\end{table}

Table~\ref{TC:Annex:Milestone_WP15} shows the milestones that were determined for the LUXE workpackage 1.5, technical coordination - Installation/Laser.

\begin{table}[h]
\begin{tabular}{lp{60mm}cp{40mm}}
\hline
Name	&	Milestone	& Target Date	& Time for completion (Months)\\
\hline\hline
% IN\stepcounter{mycounter}\themycounter &	Finish 40TW Laser Movement Plan	        & Q4/Y1 &	1\\
IN\stepcounter{mycounter}\themycounter &	Receive Phase 0 Laser to XS1	                & Q4/Y3 &	6\\
IN\stepcounter{mycounter}\themycounter &	Commision Phase 0 Laser	                        & Q1/Y4 &	3\\
% IN\stepcounter{mycounter}\themycounter &	Decommission Phase 0 Laser	                    & Q4/Y4 &	1\\
% IN\stepcounter{mycounter}\themycounter &	Phase 1 Laser installed	                & Q1/Y5 &	6\\
% IN\stepcounter{mycounter}\themycounter &	Phase 1 Laser commissioned	            & Q3/Y5 &	3\\
IN\stepcounter{mycounter}\themycounter &	Finish design of IP chamber						& Q3/Y3	& 9    \\
IN\stepcounter{mycounter}\themycounter &	Receive IP chamber						& Q3/Y3	& 1    \\
IN\stepcounter{mycounter}\themycounter &	Install IP chamber						& Q2/Y4	& 1    \\

% IN\stepcounter{mycounter}\themycounter &	Finish IP chamber movement plan	        & Q4/Y2 &	6\\
% IN\stepcounter{mycounter}\themycounter &	IP chamber in XS1	                    & Q1/Y3 &	2\\
IN\stepcounter{mycounter}\themycounter &	IP chamber commissioned	                & Q3/Y4 &	2\\
% IN\stepcounter{mycounter}\themycounter &	Finish gamma ICS chamber Movement plan	& Q4/Y4 &	6\\
% IN\stepcounter{mycounter}\themycounter &	ICS chamber in XS1	                    & Q1/Y5 &	1\\
% IN\stepcounter{mycounter}\themycounter &	ICS chamber commissioned	            & Q1/Y5 &	1\\

\hline\hline
\hline
\end{tabular}
\caption{Major Milestones required for workpackage 1.5, , technical coordination - Installation/Laser.}
\label{TC:Annex:Milestone_WP15}
\end{table}

\subsection{Risk management}

The risks to the LUXE technical coordination project associated with the Milestones above are estimated based on the following scale:

\begin{itemize}
    \item Insignificant: Risk is easily mitigated by day to day process. 
    \item Minor: Delays up to 10\% of schedule. Cost increase up to 10\% of budget. 
    \item Moderate: Delays up to 30\% of schedule. Cost increase up to 30\% of budget. 
    \item Major: Delays up to 50\% of schedule. Cost increase up to 50\% of budget. 
    \item Catastrophic: project abandoned
\end{itemize}

The probability of a risk to be realized is quantified as, rare: ($<3$\%), unlikely (3-10\%), moderate (10-50\%), likely (50-90\%) or certain ($>90\%$).\\

Table~\ref{tab:risks1} and~\ref{tab:risks2} lists the risks associated with the milestones foreseen for the LUXE experiment.\\

\begin{table}[htb!]
    \centering
    \caption{Risk description, potential impact on cost and schedule, probability to occur and strategy on how to mitigate the risk. Part 1.}
\begin{tabular}{p{0.2\linewidth}|p{0.1\linewidth}|p{0.1\linewidth}|p{0.1\linewidth}|p{0.2\linewidth}|p{0.2\linewidth}}
        \hline
Risk description & Impact on Cost & Impact on Schedule & Probability to occur & Actions required & Mitigation\\
        \hline
All installations have to be done at the same time during the shutdown period & low & moderate & likely & careful planing, hiring and training people & try to use earlier shutdowns or downscope experiment\\        \hline

Magnet delivery late & low & low & moderate  & Finalize magnet specs, and see if adequate one(s) are available or need to be ordered & Downscope initial experiment (e.g. suboptimal magnet or e-laser mode only)\\        \hline

Electron vacuum line delivery late & low & moderate & low & finish design and order ASAP & Delay installation of beam-line and data-taking\\        \hline

Electron vacuum line damaged during installation & low & low & low & careful planing, hiring and training people & Repair beam-line and delay data-taking\\        \hline

Electron beam-dumps delivery late & low & moderate & low & finish design and order ASAP & Only install e-laser configuration\\        \hline

Electron beam-dumps damaged during installation & low & moderate & low & careful planing, hiring and training people & Repair beam-dump, only install e-laser configuration\\        \hline

Photon beam-dump delivery late & low & moderate & low & finish design and order ASAP & Consider simpler beam dump, or dump beam in final wall.\\        \hline

Photon beam-dump damaged during installation & low & moderate & low & careful planing, hiring and training people & Repair beam-dump, consider simpler beam dump, or dump beam in final wall\\        \hline
         \hline
         \end{tabular}
         \label{tab:risks1}
\end{table}

\begin{table}[htb!]
    \centering
    \caption{Risk description, potential impact on cost and schedule, probability to occur and strategy on how to mitigate the risk. Part 2.}
\begin{tabular}{p{0.2\linewidth}|p{0.12\linewidth}|p{0.12\linewidth}|p{0.12\linewidth}|p{0.2\linewidth}|p{0.2\linewidth}}
        \hline
Risk description & Impact on Cost & Impact on Schedule & Probability to occur & Actions required & Mitigation\\
\hline
New building delivery late & low & low & low & finish design and order ASAP & Delay installation of laser and back-end electronics\\        \hline

\hline
Laser transport line delivery late & low & negligible & low & finish design and order ASAP & Delay installation of transport-line\\        \hline

Laser transport line damaged during installation & low & low & low & careful planing, hiring and training people & Installation in earlier shutdown\\        \hline

Laser system component(s) damaged during or prior to installation & low & negligible & moderate & careful planning and trained personell & Repair or work with degregated laser\\        \hline

IP Chamber damaged during or prior to installation & low & moderate & low & careful planning and trained personel & Repair chamber or get a new one\\        \hline

Detector damaged during installation & low & negligible & low & careful planning and trained personel & Repair detector, work with suboptimal detector configuration\\        \hline

Supporting structure construction late & low & low & low & Finish design early & Installation in earlier shutdown\\        \hline

Services to experiment installed late & low & negligible & low & Finish design early & Installation in earlier shutdown, stage service installation\\        \hline
         \hline
         \end{tabular}
         \label{tab:risks2}
\end{table}

\subsection{Responsibilities}
The responsibility and human resources for the development, construction and installation of the LUXE experiment system will be taken by the FH division in DESY Hamburg. Certain aspects of the construction and installation in the experimental area require access to the Machine group such as electrical and gas system installations in the experimental area as well as lifting the detector systems into the LUXE area by crane. The laser system is a joint responsibility of the FH DESY and Jena institute. Further details are given in Appendix~\ref{sec:Appendix:responsibilities}.\\

\subsection{DESY Infrastructure Resource Vetting}
\label{sec:desy_vetting}

The LUXE experiment will require the development, construction and installation of different elements that are detailed in chapter~\ref{chapt12}. This requires a collaborative effort between several DESY technical groups, notably from M-groups, in addition to personnel from FH. The following list shows which technical groups are leading and helping to deliver each of the main components. Personnel from ZBAU, IT and IPP are also expected to contribute throughout the lists but are not specifically reported.

\begin{itemize}
\item \textbf{Technical infrastructure and safety UG03:} Collaborative effort from all the technical groups.
\item \textbf{Safety:} D3, D5, MR with contributions from MEA, MPS, EuXFEL GmbH.
\item \textbf{The electron beam line} (including beam dumps, magnets and interaction chambers): MEA, MKK, MVS with contributions from MDI, MCS, MSK, MPC, MPS, D3, D5, EuXFEL GmbH.
\item \textbf{Laser infrastructure and beamline:} MEA with contributions from MKK, EuXFEL GmbH.
\item \textbf{Surface building} (including service and control room):  EuXFEL GmbH with contributions from MEA, MPS, MKK.
\end{itemize}

Following the CD0 decision by the DESY directorate in November 2021, the resources needed by  the LUXE experiment were detailed and then discussed with the relevant DESY groups which need to be involved. A summary of the answers received so far is given in fig.~\ref{fig:vettingtable}.

The technical groups with a major contributions or roles:
\begin{itemize}
    \item MKK will be responsible for the technical infrastructure of the experiment (water cooling, electricity, etc). Original estimates for power consumption and cooling needs were communicated to MKK. A first critical check of the estimates and needs indicate that some additional investment might be needed to meet both power and cooling demands by LUXE, beyond what has been included in the current cost estimate. For the installation of the beamline in the tunnel, the currently installed cooling power will be marginal, and most likely an update of the installations will be needed. For the experiment itself, about 200 kW of cooling power will be needed in the experimental area, and a similar power will be needed for the surface installation (laser \& laser building). Currently the electrical installation is judged to likely be sufficient, but a more careful study will be needed. 
    \item MKK estimated that the total investment needed to update the electrical and cooling power could be as much as 1.5 Mo EUR in 2022 costs. A more careful study on how already existing resources could be used, and how synergies with the ASPECT proposal which is currently under study for the same physical location at the \euxfel as the LUXE experiment is ongoing. 
    \item MEA will be involved in different areas including alignment \& survey, laser interlock, experiment magnets, experiment integration, transport \& logistics. In total 2 FTE-years spread over 4 years are deemed sufficient for the tasks. 
    \item MVS will be responsible for the LUXE beamline vacuum system. A major challenge will be the interface between the beam-line vacuum, and the large volume laser transport system. Differential pumping will be needed, to decouple the laser vacuum from the machine vacuum. MVS agrees with the strategy and - under the assumption that the system will be built by external companies - will be able to supervise and advise tha activities with 0.5 FTE in total.
    \item XFEL/Bau: The only major construction project will be the laser building located on the \euxfel grounds at Osdorfer Born. The building will be financed by LUXE, and constructed under responsibility of the \euxfel company. A detailed specification of the building was communicated to \euxfel, and will form the basis of a concrete planning proposal. Preliminary estimates done by DESY and based on recently erected buildings at DESY amount to about 1 Mo EUR construction costs of the building, but are not yet confirmed by the \euxfel company. 
    \item IT will provide the IT infrastructure at the experimental site. This includes the establishment of sufficient IT infrastructure at the experiment and the surface location, and adequate band-width to transfer data from the experiment to central storage on the DESY site. The resource estimate was originally done by the IT group. The estimate does not include the support of the operation of the experiment.
\end{itemize}

The LUXE experiment will be operated by DESY and be located at the \euxfel premises. Safety issues are therefore to be addressed from early on by both relevant groups from DESY and from \euxfel. The overall concept has been developed together with SAVE, the other involved groups are MEA for the laser, MPS for the interlock, D3 for radiation protection and D5 for gases. The safety concept is an integral part of the project definition. 
\begin{itemize}
  \item MPS is responsible for radiation interlocks and risk assessments. The group asked to be involved as soon as possible in the design of the experiment and confirmed that the budget allocated for the radiation interlocks and the integrated 0.5 FTE-year person-power will be enough to realize the project.
  \item SAVE will be essential in defining safety concepts of the experiment. They will be involved from the beginning, assessing and verifying that the concept can be implemented. No major concerns were raised with the plans presented by LUXE. The exact responsibilities will have to be defined, once the experiment is approved.
\end{itemize}

A number of technical groups will be involved with relatively small contributions, of typically a fraction of a FTE-year.

\begin{itemize}
\item MPC will be involved with the dipole magnet power supplies used in the experiment. The resource estimate was originally done by the MPC group.
\item MCS will be involved in the beamline control system used in the experiment. MCS approved the estimate.
\item MSK will be involved in the synchronization of the \euxfel with the laser system. The resource estimate was originally done by the MSK group, and \item MDI will be involved in the design of the beam instrumentation. The resource estimate was developed by the project engineer. Given the modest amount of beam instrumentation that is currently planned to be installed, no concerns were raised by the group after the estimate was submitted.
\end{itemize}

The directorate of the EuXFEL welcomes the initiative and is generally supportive. 

\begin{figure}
    \centering
    \includegraphics[width=\textwidth]{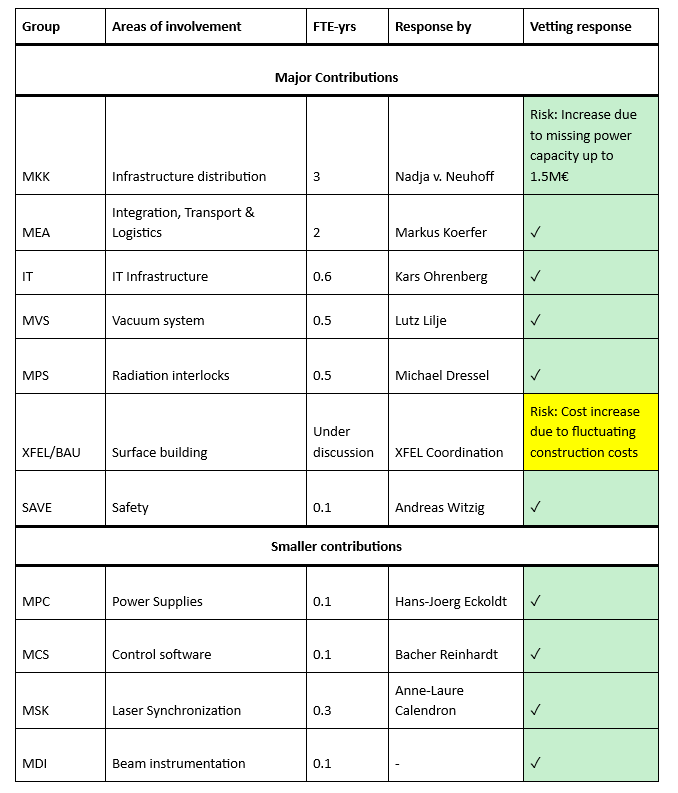}
    \caption{Responses from LUXE resource vetting at DESY.}
    \label{fig:vettingtable}
\end{figure}

\subsection*{Responsibilities required for each of the different work-package}

In the following tables the groups identified for each of the items required in the construction of the experiment are shown. The estimates presented here and also in Section~\ref{sec:ressources} still require further confirmations with each working groups.
\label{sec:Appendix:responsibilities}
\begin{landscape}% Landscape page
\begin{table}[]
\tiny
\begin{tabular}{|p{0.1\linewidth}|p{0.1\linewidth}|p{0.07\linewidth}|p{0.015\linewidth}|p{0.02\linewidth}|p{0.02\linewidth}|p{0.02\linewidth}|p{0.02\linewidth}|p{0.02\linewidth}|p{0.02\linewidth}|p{0.02\linewidth}|p{0.02\linewidth}|p{0.02\linewidth}|p{0.015\linewidth}|p{0.015\linewidth}|p{0.015\linewidth}|p{0.015\linewidth}|p{0.015\linewidth}|p{0.015\linewidth}|p{0.015\linewidth}|p{0.02\linewidth}|p{0.02\linewidth}|p{0.04\linewidth}|}
\hline

Workpackage & Item &  & FH & MEA & ZBAU & MDI & MVS & MCS & MSK & MPS & MPC & MKK & D3 & D5 & IT & IPP & MR & ZM3 & ZM5 & \euxfel Company & External company & Other institute\\ 
\multirow{19}{*}{\shortstack[l]{1) Electron beam \\line}} &  &  &  &  &  &  &  &  &  &  &  &  &  &  &  &  &  &  &  &  &  & \\ 
\hline
\cline{2-23}

 & \multirow{3}{*}{\shortstack[l]{Beampipe Apertures\\ and transition}} & Design & Or & Or &  &  & And &  &  &  &  &  &  &  &  &  &  &  &  &  &  & \\ 
 &  & Construction &  &  &  &  &  &  &  &  &  &  &  &  &  &  &  & Or &  &  & Or & \\ 
 &  & Installation & Or & Or &  &  & And &  &  &  &  &  &  &  &  &  &  &  &  &  &  & \\ 
\cline{2-23}

 & \multirow{3}{*}{\shortstack[l]{Beamline support \\and vibration}} & Design & Or & Or &  &  &  &  &  &  &  &  &  &  &  &  &  &  &  &  &  & \\ 
 &  & Construction &  & And &  &  &  &  &  &  &  &  &  &  &  &  &  & Or & Or &  & Or & \\ 
 &  & Installation & Or & Or &  &  &  &  &  &  &  &  &  &  &  &  &  &  &  &  &  & \\ 
\cline{2-23}

 & \multirow{3}{*}{\shortstack[l]{Alignment and Survey}} & Design & And & And &  &  &  &  &  &  &  &  &  &  &  &  &  &  &  &  &  & \\ 
 &  & Construction &  & And &  &  &  &  &  &  &  &  &  &  &  &  &  &  &  &  &  & \\ 
 &  & Installation & And & And &  &  &  &  &  &  &  &  &  &  &  &  &  &  &  &  &  & \\ 
\cline{2-23}

 & \multirow{3}{*}{\shortstack[l]{Transport}} & Design & Or & Or &  &  &  &  &  &  &  &  &  &  &  &  &  &  &  &  &  & \\ 
 &  & Construction &  & And &  &  &  &  &  &  &  &  &  &  &  &  &  &  &  & And &  & \\ 
 &  & Installation & Or & Or &  &  &  &  &  &  &  &  &  &  &  &  &  &  &  & And &  & \\ 
\cline{2-23}

 & \multirow{3}{*}{\shortstack[l]{Beam monitors}} & Design &  &  &  & And &  &  &  &  &  &  &  &  &  &  &  &  &  &  &  & \\ 
 &  & Construction &  &  &  & Or &  &  &  &  &  &  &  &  &  &  &  &  &  &  & Or & \\ 
 &  & Installation &  & And &  & And & And &  &  &  &  &  &  &  &  &  &  &  &  &  &  & \\ 
\cline{2-23}

 & \multirow{3}{*}{\shortstack[l]{Beam controls / ctrl\\ system and timing}} & Design &  &  &  &  &  & And & And & And &  &  &  &  &  &  &  &  &  &  &  & \\ 
 &  & Construction &  &  &  &  &  & And & And & And &  &  &  &  &  &  &  &  &  &  &  & \\ 
 &  & Installation &  &  &  &  &  & And & And & And &  &  &  &  &  &  &  &  &  &  &  & \\ 
%  &  &  &  &  &  &  &  &  &  &  &  &  &  &  &  &  &  &  &  &  &  & \\ 

\multirow{19}{*}{\shortstack[l]{2) Beam dumps}} &  &  &  &  &  &  &  &  &  &  &  &  &  &  &  &  &  &  &  &  &  & \\ 
\hline

 & \multirow{3}{*}{\shortstack[l]{Electron-laser \\ electron dump}} & Design & And &  &  &  &  &  &  &  &  &  & And &  &  &  &  &  &  &  &  & Dubna\\ 
 &  & Construction &  &  &  &  &  &  &  &  &  &  &  &  &  &  &  &  &  &  &  & Dubna\\ 
 &  & Installation & Or & Or &  &  &  &  &  &  &  &  & And &  &  &  &  &  &  &  &  & \\ 
 \cline{2-23}

 & \multirow{3}{*}{\shortstack[l]{Gamma-laser \\ electron dump}} & Design & And &  &  &  &  &  &  &  &  &  & And &  &  &  &  &  &  &  &  & Dubna\\ 
 &  & Construction &  &  &  &  &  &  &  &  &  &  &  &  &  &  &  &  &  &  &  & Dubna\\ 
 &  & Installation & Or & Or &  &  &  &  &  &  &  &  & And &  &  &  &  &  &  &  &  & \\ 
 \cline{2-23}

 & \multirow{3}{*}{\shortstack[l]{Final photon dump}} & Design & And &  &  &  &  &  &  &  &  &  & And &  &  &  &  &  &  &  &  & Dubna\\ 
 &  & Construction &  &  &  &  &  &  &  &  &  &  &  &  &  &  &  &  &  &  &  & Dubna\\ 
 &  & Installation & Or & Or &  &  &  &  &  &  &  &  & And &  &  &  &  &  &  &  &  & \\ 
 \cline{2-23}

 & \multirow{3}{*}{\shortstack[l]{Shielding}} & Design & Or & Or &  &  &  &  &  &  &  &  &  &  &  &  &  &  &  &  &  & Dubna\\ 
 &  & Construction & Or & Or &  &  &  &  &  &  &  &  & And &  &  &  &  &  &  &  & And & \\ 
 &  & Installation & Or & Or &  &  &  &  &  &  &  &  & And &  &  &  &  &  &  &  & And & \\ 
 \cline{2-23}

 & \multirow{3}{*}{\shortstack[l]{Monitoring}} & Design & And & And &  &  &  &  &  &  &  &  & And &  &  &  &  &  &  &  &  & \\ 
 &  & Construction & And &  &  &  &  &  &  &  &  &  & And & And  &  &  &  &  &  &  &  & \\ 
 &  & Installation & And &  &  &  &  &  &  &  &  &  & And & And &  &  &  &  &  &  &  & \\ 
 \cline{2-23}

 & \multirow{3}{*}{\shortstack[l]{Services}} & Design & And &  &  &  &  &  &  &  &  & And &  &  &  &  &  &  &  &  &  & \\ 
 &  & Construction & And &  &  &  &  &  &  &  &  & And &  &  &  &  &  &  &  &  &  & \\ 
 &  & Installation & And &  &  &  &  &  &  &  &  & And &  &  &  &  &  &  &  &  &  & \\ 
 \cline{2-23}

 & \multirow{3}{*}{\shortstack[l]{Transport}} & Design & Or & Or & And &  &  &  &  &  &  &  &  &  &  &  &  &  &  &  &  & \\ 
 &  & Construction &  &  &  &  &  &  &  &  &  &  &  &  &  &  &  &  &  &  &  & \\ 
 &  & Installation & Or & Or & And &  &  &  &  &  &  &  &  &  &  &  &  &  &  &  &  & \\ 
 &  &  &  &  &  &  &  &  &  &  &  &  &  &  &  &  &  &  &  &  &  & \\ 
 
 \hline

\hline
\end{tabular}
\caption{Identified responsibilities for the different items required by the LUXE experiment, for the design, construction and installation. When a group is needed it is assigned with "And". If two groups can achieve the same task they are assigned and "Or".}
% \label{TC:Annex:Resources_WP65}
\end{table}
\end{landscape}% Landscape page

\begin{landscape}% Landscape page
\begin{table}[]
\tiny
\begin{tabular}{|p{0.1\linewidth}|p{0.1\linewidth}|p{0.07\linewidth}|p{0.015\linewidth}|p{0.02\linewidth}|p{0.02\linewidth}|p{0.02\linewidth}|p{0.02\linewidth}|p{0.02\linewidth}|p{0.02\linewidth}|p{0.02\linewidth}|p{0.02\linewidth}|p{0.02\linewidth}|p{0.015\linewidth}|p{0.015\linewidth}|p{0.015\linewidth}|p{0.015\linewidth}|p{0.015\linewidth}|p{0.015\linewidth}|p{0.015\linewidth}|p{0.02\linewidth}|p{0.02\linewidth}|p{0.04\linewidth}|}
\hline

Workpackage & Item &  & FH & MEA & ZBAU & MDI & MVS & MCS & MSK & MPS & MPC & MKK & D3 & D5 & IT & IPP & MR & ZM3 & ZM5 & \euxfel Company & External company & Other institute\\
\multirow{7}{*}{\shortstack[l]{3) Experiment \\magnets}} &  &  &  &  &  &  &  &  &  &  &  &  &  &  &  &  &  &  &  &  &  & \\ 
\hline
\cline{2-23}
 &\multirow{3}{*}{\shortstack[l]{Procurement tests \\and measurements}} & Design &  & And &  &  &  &  &  &  &  &  &  &  &  &  &  &  &  &  &  & \\ 
 &  & Construction &  & And &  &  &  &  &  &  &  &  &  &  &  &  &  &  &  &  &  & \\ 
 &  & Installation &  & And &  &  &  &  &  &  &  &  &  &  &  &  &  &  &  &  &  & \\ 
 \cline{2-23}

 &\multirow{3}{*}{\shortstack[l]{Power network}} & Design &  &  &  &  &  &  &  &  &  & And &  &  &  &  &  &  &  &  &  & \\ 
 &  & Construction &  &  &  &  &  &  &  &  &  & And &  &  &  &  &  &  &  &  &  & \\ 
 &  & Installation &  &  &  &  &  &  &  &  &  & And &  &  &  &  &  &  &  &  &  & \\ 
  \cline{2-23}

 &\multirow{3}{*}{\shortstack[l]{Power supplies}} & Design &  &  &  &  &  &  &  &  & And &  &  &  &  &  &  &  &  &  &  & \\ 
 &  & Construction &  &  &  &  &  &  &  &  &  & And &  &  &  &  &  &  &  &  &  & \\ 
 &  & Installation &  &  &  &  &  &  &  &  &  & And &  &  &  &  &  &  &  &  &  & \\ 
  \cline{2-23}
 &\multirow{3}{*}{\shortstack[l]{Cooling}} & Design &  &  &  &  &  &  &  &  & And &  &  &  &  &  &  &  &  &  &  & \\ 
 &  & Construction &  &  &  &  &  &  &  &  &  & And &  &  &  &  &  &  &  &  &  & \\ 
 &  & Installation &  &  &  &  &  &  &  &  &  & And &  &  &  &  &  &  &  &  &  & \\ 
  \cline{2-23}

 &\multirow{3}{*}{\shortstack[l]{Cabling}} & Design &  &  &  &  &  &  &  &  & And &  &  &  &  &  &  &  &  &  &  & \\ 
 &  & Construction &  &  &  &  &  &  &  &  & And &  &  &  &  &  &  &  &  &  &  & \\ 
 &  & Installation &  &  &  &  &  &  &  &  & And &  &  &  &  &  &  &  &  &  &  & \\ 
  \cline{2-23}

 &\multirow{3}{*}{\shortstack[l]{Vacuum chambers\\ and Exit windows}} & Design &  &  &  &  & And &  &  &  &  &  &  &  &  &  &  &  &  &  &  & Weizmann\\ 
 &  & Construction &  &  &  &  & And &  &  &  &  &  &  &  &  &  &  &  &  &  &  & Weizmann\\ 
 &  & Installation & And & And &  &  & And &  &  &  &  &  &  &  &  &  &  &  &  &  &  & \\ 
  \cline{2-23}

 &\multirow{3}{*}{\shortstack[l]{Survey and positions}} & Design & And & And &  &  &  &  &  &  &  &  &  &  &  &  &  &  &  &  &  & \\ 
 &  & Construction &  &  &  &  &  &  &  &  &  &  &  &  &  &  &  &  &  &  &  & \\ 
 &  & Installation & And & And &  &  &  &  &  &  &  &  &  &  &  &  &  &  &  &  &  & \\ 
 &  &  &  &  &  &  &  &  &  &  &  &  &  &  &  &  &  &  &  &  &  & \\ 
  \cline{2-23}

 \hline

\hline
\end{tabular}
\caption{Identified responsibilities for the different items required by the LUXE experiment, for the design, construction and installation. When a group is needed it is assigned with "And". If two groups can achieve the same task they are assigned and "Or".}
% \label{TC:Annex:Resources_WP65}
\end{table}
\end{landscape}% Landscape page

\begin{landscape}% Landscape page
\begin{table}[]
\tiny
\begin{tabular}{|p{0.1\linewidth}|p{0.1\linewidth}|p{0.07\linewidth}|p{0.015\linewidth}|p{0.02\linewidth}|p{0.02\linewidth}|p{0.02\linewidth}|p{0.02\linewidth}|p{0.02\linewidth}|p{0.02\linewidth}|p{0.02\linewidth}|p{0.02\linewidth}|p{0.02\linewidth}|p{0.015\linewidth}|p{0.015\linewidth}|p{0.015\linewidth}|p{0.015\linewidth}|p{0.015\linewidth}|p{0.015\linewidth}|p{0.015\linewidth}|p{0.02\linewidth}|p{0.02\linewidth}|p{0.04\linewidth}|}
\hline

Workpackage & Item &  & FH & MEA & ZBAU & MDI & MVS & MCS & MSK & MPS & MPC & MKK & D3 & D5 & IT & IPP & MR & ZM3 & ZM5 & \euxfel Company & External company & Other institute\\
% \hline
% \multirow{19}{*}{\shortstack[l]{1) Electron beam \\line}} &  &  &  &  &  &  &  &  &  &  &  &  &  &  &  &  &  &  &  &  &  & \\ 
% \hline
% \cline{2-23}

%  & \multirow{3}{*}{\shortstack[l]{Beampipe Apertur\\ and transition}} & Design & Or & Or &  &  & And &  &  &  &  &  &  &  &  &  &  &  &  &  &  & \\ 
%  &  & Construction &  &  &  &  &  &  &  &  &  &  &  &  &  &  &  & Or &  &  & Or & \\ 
%  &  & Installation & Or & Or &  &  & And &  &  &  &  &  &  &  &  &  &  &  &  &  &  & \\ 
% \cline{2-23}
\multirow{12}{*}{\shortstack[l]{4) Technical \\infrastructure\\ UG03}} &  &  &  &  &  &  &  &  &  &  &  &  &  &  &  &  &  &  &  &  &  & \\ 
\hline
\cline{2-23}
 &\multirow{3}{*}{\shortstack[l]{Power network}} & Design &  &  &  &  &  & And &  &  & And & And &  &  &  &  &  &  &  &  &  & \\ 
 &  & Construction &  &  &  &  &  & And &  &  & And & And &  &  &  &  &  &  &  &  &  & \\ 
 &  & Installation &  &  &  &  &  & And &  &  & And & And &  &  &  &  &  &  &  &  &  & \\ 
 \cline{2-23}
 & Air conditioning & Design &  &  &  &  &  & And &  &  &  & And &  &  &  &  &  &  &  &  &  & \\ 
 &  & Construction &  &  &  &  &  & And &  &  &  & And &  &  &  &  &  &  &  &  &  & \\ 
 &  & Installation &  &  &  &  &  & And &  &  &  & And &  &  &  &  &  &  &  &  &  & \\ 
  \cline{2-23}

 & \multirow{3}{*}{\shortstack[l]{Liquids and\\ gas supply}} & Design &  & And &  &  &  & And &  &  &  &  &  &  &  &  &  &  &  &  &  & \\ 
 &  & Construction &  & And &  &  &  & And &  &  &  &  &  &  &  &  &  &  &  &  & And & \\ 
 &  & Installation &  & And &  &  &  & And &  &  &  &  &  &  &  &  &  &  &  &  & And & \\ 
  \cline{2-23}

 & \multirow{3}{*}{\shortstack[l]{Cabling (detector \\signal+beam \\monitoring)}} & Design & And &  &  & And &  &  &  &  &  &  &  &  &  &  &  &  &  &  & And & \\ 
 &  & Construction &  &  &  &  &  &  &  &  &  &  &  &  &  &  &  &  &  & And & And & \\ 
 &  & Installation &  &  &  &  &  &  &  &  &  &  &  &  &  &  &  &  &  & And & And & \\ 
  \cline{2-23}

 & \multirow{3}{*}{\shortstack[l]{Cable tray}} & Design &  &  &  & And &  &  &  &  &  &  &  &  &  &  &  &  &  & And & And & \\ 
 &  & Construction &  &  &  & And &  &  &  &  &  &  &  &  &  &  &  &  &  & And & And & \\ 
 &  & Installation &  &  &  & And &  &  &  &  &  &  &  &  &  &  &  &  &  & And & And & \\ 
  \cline{2-23}

 & \multirow{3}{*}{\shortstack[l]{Networking}} & Design &  &  &  & And &  &  &  &  &  &  &  &  & And &  &  &  &  &  &  & \\ 
 &  & Construction &  &  &  & And &  &  &  &  &  &  &  &  & And &  &  &  &  &  &  & \\ 
 &  & Installation &  &  &  & And &  &  &  &  &  &  &  &  &  &  &  &  &  &  & And & \\ 
  \cline{2-23}

 & \multirow{3}{*}{\shortstack[l]{Front-end racks}} & Design & And &  &  & And & And &  & And &  &  &  &  &  &  &  &  &  &  &  &  & \\ 
 &  & Construction & And &  &  & And & And &  & And &  &  &  &  &  &  &  &  &  &  &  &  & \\ 
 &  & Installation & And &  &  & And & And &  & And &  &  &  &  &  &  &  &  &  &  &  &  & \\ 
  \cline{2-23}

 & \multirow{3}{*}{\shortstack[l]{Detector movable \\structure}} & Design & And &  &  &  &  &  &  &  &  &  &  &  &  &  &  &  &  &  &  & \\ 
 &  & Construction &  &  &  &  &  &  &  &  &  &  &  &  &  &  &  &  &  &  & And & \\ 
 &  & Installation & And &  &  &  &  &  &  &  &  &  &  &  &  &  &  &  &  &  &  & \\ 
  \cline{2-23}

 & \multirow{3}{*}{\shortstack[l]{Detector support \\structure}} & Design & And &  &  &  &  &  &  &  &  &  &  &  &  &  &  &  &  &  &  & \\ 
 &  & Construction & And &  &  &  &  &  &  &  &  &  &  &  &  &  &  &  &  &  &  & \\ 
 &  & Installation & And &  &  &  &  &  &  &  &  &  &  &  &  &  &  &  &  &  &  & \\ 
  \cline{2-23}

 & \multirow{3}{*}{\shortstack[l]{Positioning and \\survey}} & Design & And & And &  &  &  &  &  &  &  &  &  &  &  &  &  &  &  &  &  & \\ 
 &  & Construction &  &  &  &  &  &  &  &  &  &  &  &  &  &  &  &  &  &  &  & \\ 
 &  & Installation & And & And &  &  &  &  &  &  &  &  &  &  &  &  &  &  &  &  &  & \\ 
  \cline{2-23}

 & \multirow{3}{*}{\shortstack[l]{Environment \\monitoring \\(temp and  hum..)}} & Design &  &  &  &  &  &  &  &  &  & And &  &  &  &  &  &  &  &  &  & \\ 
 &  & Construction &  &  &  &  &  &  &  &  &  & And &  &  &  &  &  &  &  &  &  & \\ 
 &  & Installation &  &  &  &  &  &  &  &  &  & And &  &  &  &  &  &  &  &  &  & \\ 
  \cline{2-23}

 & \multirow{3}{*}{\shortstack[l]{Development of \\integration concept}} & Design & And & And &  &  &  &  &  &  &  &  &  &  &  & And &  &  &  &  &  & \\ 
 &  & Construction &  &  &  &  &  &  &  &  &  &  &  &  &  &  &  &  &  &  &  & \\ 
 &  & Installation &  &  &  &  &  &  &  &  &  &  &  &  &  &  &  &  &  &  &  & \\ 
 &  &  &  &  &  &  &  &  &  &  &  &  &  &  &  &  &  &  &  &  &  & \\ 
 
 \hline

\hline
\end{tabular}
\caption{Identified responsibilities for the different items required by the LUXE experiment, for the design, construction and installation. When a group is needed it is assigned with "And". If two groups can achieve the same task they are assigned and "Or".}
% \label{TC:Annex:Resources_WP65}
\end{table}
\end{landscape}% Landscape page

\begin{landscape}% Landscape page
\begin{table}[]
\tiny
\begin{tabular}{|p{0.1\linewidth}|p{0.1\linewidth}|p{0.07\linewidth}|p{0.015\linewidth}|p{0.02\linewidth}|p{0.02\linewidth}|p{0.02\linewidth}|p{0.02\linewidth}|p{0.02\linewidth}|p{0.02\linewidth}|p{0.02\linewidth}|p{0.02\linewidth}|p{0.02\linewidth}|p{0.015\linewidth}|p{0.015\linewidth}|p{0.015\linewidth}|p{0.015\linewidth}|p{0.015\linewidth}|p{0.015\linewidth}|p{0.015\linewidth}|p{0.02\linewidth}|p{0.02\linewidth}|p{0.04\linewidth}|}
\hline

Workpackage & Item &  & FH & MEA & ZBAU & MDI & MVS & MCS & MSK & MPS & MPC & MKK & D3 & D5 & IT & IPP & MR & ZM3 & ZM5 & \euxfel Company & External company & Other institute\\

\multirow{10}{*}{\shortstack[l]{5) Surface building \\(include service \\and control room ) }} &  &  &  &  &  &  &  &  &  &  &  &  &  &  &  &  &  &  &  &  &  & \\ 
\hline
\cline{2-23}
 &\multirow{3}{*}{\shortstack[l]{Building }} & Design & And &  &  &  &  &  &  &  &  &  &  &  &  &  &  &  &  &  And &  And & \\ 
 &  & Construction &  &  &  &  &  &  &  &  &  &  &  &  &  &  &  &  &  &  And &  And & \\ 
 &  & Installation &  &  &  &  &  &  &  &  &  &  &  &  &  &  &  &  &  &  &  & \\ 
\cline{2-23}
 &\multirow{3}{*}{\shortstack[l]{Power network}} & Design &  &  &  &  &  & And &  &  & And & And &  &  &  &  &  &  &  &  &  & \\ 
 &  & Construction &  &  &  &  &  & And &  &  & And & And &  &  &  &  &  &  &  &  &  & \\ 
 &  & Installation &  &  &  &  &  & And &  &  & And & And &  &  &  &  &  &  &  &  &  & \\ 
 \cline{2-23}
 & Air conditioning & Design &  &  &  &  &  & And &  &  &  & And &  &  &  &  &  &  &  &  &  & \\ 
 &  & Construction &  &  &  &  &  & And &  &  &  & And &  &  &  &  &  &  &  &  &  & \\ 
 &  & Installation &  &  &  &  &  & And &  &  &  & And &  &  &  &  &  &  &  &  &  & \\ 
 \cline{2-23}

 & \multirow{3}{*}{\shortstack[l]{Liquids and\\ gas supply}} & Design &  & And &  &  &  & And &  &  &  &  &  &  &  &  &  &  &  &  &  & \\ 
 &  & Construction &  & And &  &  &  & And &  &  &  &  &  &  &  &  &  &  &  &  & And & \\ 
 &  & Installation &  & And &  &  &  & And &  &  &  &  &  &  &  &  &  &  &  &  & And & \\ 
  \cline{2-23}

 & \multirow{3}{*}{\shortstack[l]{Cabling}} & Design & And &  &  & And &  &  &  &  &  &  &  &  &  &  &  &  &  &  & And & \\ 
 &  & Construction &  &  &  &  &  &  &  &  &  &  &  &  &  &  &  &  &  & And & And & \\ 
 &  & Installation &  &  &  &  &  &  &  &  &  &  &  &  &  &  &  &  &  & And & And & \\ 
  \cline{2-23}

 & \multirow{3}{*}{\shortstack[l]{Cable tray}} & Design &  &  &  & And &  &  &  &  &  &  &  &  &  &  &  &  &  & And & And & \\ 
 &  & Construction &  &  &  & And &  &  &  &  &  &  &  &  &  &  &  &  &  & And & And & \\ 
 &  & Installation &  &  &  & And &  &  &  &  &  &  &  &  &  &  &  &  &  & And & And & \\ 
  \cline{2-23}

 & \multirow{3}{*}{\shortstack[l]{Networking}} & Design &  &  &  & And &  &  &  &  &  &  &  &  & And &  &  &  &  &  &  & \\ 
 &  & Construction &  &  &  & And &  &  &  &  &  &  &  &  & And &  &  &  &  &  &  & \\ 
 &  & Installation &  &  &  & And &  &  &  &  &  &  &  &  &  &  &  &  &  &  & And & \\ 
  \cline{2-23}

 & \multirow{3}{*}{\shortstack[l]{Front-end racks}} & Design & And &  &  &  &  &  &  &  &  &  &  &  &  &  &  &  &  &  &  & \\ 
 &  & Construction & And &  &  &  &  &  &  &  &  &  &  &  &  &  &  &  &  &  &  & \\ 
 &  & Installation & And &  &  &  &  &  &  &  &  &  &  &  &  &  &  &  &  &  &  & \\ 
  \cline{2-23}
 & \multirow{3}{*}{\shortstack[l]{Environment \\monitoring \\(temp and  hum..)}} & Design &  &  &  &  &  &  &  &  &  & And &  &  &  &  &  &  &  &  &  & \\ 
 &  & Construction &  &  &  &  &  &  &  &  &  & And &  &  &  &  &  &  &  &  &  & \\ 
 &  & Installation &  &  &  &  &  &  &  &  &  & And &  &  &  &  &  &  &  &  &  & \\ 
  \cline{2-23}

 & \multirow{3}{*}{\shortstack[l]{Development of \\integration concept}} & Design & And & And &  &  &  &  &  &  &  &  &  &  &  & And &  &  &  &  &  & \\ 
 &  & Construction &  &  &  &  &  &  &  &  &  &  &  &  &  &  &  &  &  &  &  & \\ 
 &  & Installation &  &  &  &  &  &  &  &  &  &  &  &  &  &  &  &  &  &  &  & \\ 
 &  &  &  &  &  &  &  &  &  &  &  &  &  &  &  &  &  &  &  &  &  & \\ 

 \hline

\hline
\end{tabular}
\caption{Identified responsibilities for the different items required by the LUXE experiment, for the design, construction and installation. When a group is needed it is assigned with "And". If two groups can achieve the same task they are assigned and "Or".}
% \label{TC:Annex:Resources_WP65}
\end{table}
\end{landscape}% Landscape page

\begin{landscape}% Landscape page
\begin{table}[]
\tiny
\begin{tabular}{|p{0.1\linewidth}|p{0.1\linewidth}|p{0.07\linewidth}|p{0.015\linewidth}|p{0.02\linewidth}|p{0.02\linewidth}|p{0.02\linewidth}|p{0.02\linewidth}|p{0.02\linewidth}|p{0.02\linewidth}|p{0.02\linewidth}|p{0.02\linewidth}|p{0.02\linewidth}|p{0.015\linewidth}|p{0.015\linewidth}|p{0.015\linewidth}|p{0.015\linewidth}|p{0.015\linewidth}|p{0.015\linewidth}|p{0.015\linewidth}|p{0.02\linewidth}|p{0.02\linewidth}|p{0.04\linewidth}|}
\hline

Workpackage & Item &  & FH & MEA & ZBAU & MDI & MVS & MCS & MSK & MPS & MPC & MKK & D3 & D5 & IT & IPP & MR & ZM3 & ZM5 & \euxfel Company & External company & Other institute\\

\multirow{16}{*}{\shortstack[l]{6) Laser \\infrastructure\\ and beamline}} &  &  &  &  &  &  &  &  &  &  &  &  &  &  &  &  &  &  &  &  &  & \\  

\hline
\cline{2-23}
 &\multirow{3}{*}{\shortstack[l]{Laser clean room}} & Design & And &  &  &  &  &  &  &  &  &  &  &  &  &  &  &  &  &  & And & \\ 
 &  & Construction &  &  &  &  &  &  &  &  &  &  &  &  &  &  &  &  &  &  & And & \\ 
 &  & Installation &  & And &  &  &  &  &  &  &  &  &  &  &  &  &  &  &  &  & And & \\ 
\cline{2-23}
 &\multirow{3}{*}{\shortstack[l]{Laser service room}} & Design & And &  &  &  &  &  &  &  &  &  &  &  &  &  &  &  &  &  & And & \\ 
 &  & Construction &  &  &  &  &  &  &  &  &  &  &  &  &  &  &  &  &  &  & And & \\ 
 &  & Installation &  &  &  &  &  &  &  &  &  &  &  &  &  &  &  &  &  &  & And & \\ 
\cline{2-23}
 &\multirow{3}{*}{\shortstack[l]{Power network}} & Design &  &  &  &  &  & And &  &  & And & And &  &  &  &  &  &  &  &  &  & \\ 
 &  & Construction &  &  &  &  &  & And &  &  & And & And &  &  &  &  &  &  &  &  &  & \\ 
 &  & Installation &  &  &  &  &  & And &  &  & And & And &  &  &  &  &  &  &  &  &  & \\ 
 \cline{2-23}
 & Air conditioning & Design &  &  &  &  &  & And &  &  &  & And &  &  &  &  &  &  &  &  &  & \\ 
 &  & Construction &  &  &  &  &  & And &  &  &  & And &  &  &  &  &  &  &  &  &  & \\ 
 &  & Installation &  &  &  &  &  & And &  &  &  & And &  &  &  &  &  &  &  &  &  & \\ 
  \cline{2-23}
  & \multirow{3}{*}{\shortstack[l]{Liquids and\\ gas supply}} & Design &  & And &  &  &  & And &  &  &  &  &  &  &  &  &  &  &  &  &  & \\ 
 &  & Construction &  & And &  &  &  & And &  &  &  &  &  &  &  &  &  &  &  &  & And & \\ 
 &  & Installation &  & And &  &  &  & And &  &  &  &  &  &  &  &  &  &  &  &  & And & \\ 
  \cline{2-23}

 & \multirow{3}{*}{\shortstack[l]{Cabling}} & Design & And &  &  & And &  &  &  &  &  &  &  &  &  &  &  &  &  &  & And & \\ 
 &  & Construction &  &  &  &  &  &  &  &  &  &  &  &  &  &  &  &  &  & And & And & \\ 
 &  & Installation &  &  &  &  &  &  &  &  &  &  &  &  &  &  &  &  &  & And & And & \\ 
  \cline{2-23}

 & \multirow{3}{*}{\shortstack[l]{Cable tray}} & Design &  &  &  & And &  &  &  &  &  &  &  &  &  &  &  &  &  & And & And & \\ 
 &  & Construction &  &  &  & And &  &  &  &  &  &  &  &  &  &  &  &  &  & And & And & \\ 
 &  & Installation &  &  &  & And &  &  &  &  &  &  &  &  &  &  &  &  &  & And & And & \\ 
  \cline{2-23}

 & \multirow{3}{*}{\shortstack[l]{Networking}} & Design &  &  &  & And &  &  &  &  &  &  &  &  & And &  &  &  &  &  &  & \\ 
 &  & Construction &  &  &  & And &  &  &  &  &  &  &  &  & And &  &  &  &  &  &  & \\ 
 &  & Installation &  &  &  & And &  &  &  &  &  &  &  &  &  &  &  &  &  &  & And & \\ 
  \cline{2-23}

 & \multirow{3}{*}{\shortstack[l]{Front-end racks}} & Design & And &  &  &  &  &  &  &  &  &  &  &  &  &  &  &  &  &  &  & \\ 
 &  & Construction & And &  &  &  &  &  &  &  &  &  &  &  &  &  &  &  &  &  &  & \\ 
 &  & Installation & And &  &  &  &  &  &  &  &  &  &  &  &  &  &  &  &  &  &  & \\ 
  \cline{2-23}
 & \multirow{3}{*}{\shortstack[l]{Environment \\monitoring \\(temp and  hum..)}} & Design &  &  &  &  &  &  &  &  &  & And &  &  &  &  &  &  &  &  &  & \\ 
 &  & Construction &  &  &  &  &  &  &  &  &  & And &  &  &  &  &  &  &  &  &  & \\ 
 &  & Installation &  &  &  &  &  &  &  &  &  & And &  &  &  &  &  &  &  &  &  & \\ 
  \cline{2-23}

 &\multirow{3}{*}{\shortstack[l]{Mirrors structure}} & Design &  &  & And &  &  &  &  &  &  &  &  &  &  &  &  &  &  &  &  & Jena\\ 
 &  & Construction &  &  &  &  &  &  &  &  &  &  &  &  &  &  &  & And &  &  &  & \\ 
 &  & Installation &  & And &  &  &  &  &  &  &  &  &  &  &  &  &  &  &  &  &  & \\ 
\cline{2-23}
 &\multirow{3}{*}{\shortstack[l]{Beampipe and\\  apertures and\\ transition}} & Design &  &  &  &  &  &  &  &  &  &  &  &  &  &  &  &  &  &  &  & Jena\\ 
 &  & Construction &  &  &  &  &  &  &  &  &  &  &  &  &  &  &  & And &  &  &  & \\ 
 &  & Installation &  & And &  &  &  &  &  &  &  &  &  &  &  &  &  &  &  &  &  & \\ 
\cline{2-23}
 &\multirow{3}{*}{\shortstack[l]{Beamline support}} & Design &  &  &  &  &  &  &  &  &  &  &  &  &  &  &  &  &  &  &  & Jena\\ 
 &  & Construction &  &  &  &  &  &  &  &  &  &  &  &  &  &  &  & And &  &  &  & \\ 
 &  & Installation &  & And &  &  &  &  &  &  &  &  &  &  &  &  &  &  &  &  &  & \\ 
\cline{2-23}
 &\multirow{3}{*}{\shortstack[l]{Positioning \\and survey}} & Design & And & And &  &  &  &  &  &  &  &  &  &  &  &  &  &  &  &  &  & Jena\\ 
 &  & Construction &  &  &  &  &  &  &  &  &  &  &  &  &  &  &  &  &  &  &  & \\ 
 &  & Installation & And & And &  &  &  &  &  &  &  &  &  &  &  &  &  &  &  &  &  & \\ 
\cline{2-23}
 &\multirow{3}{*}{\shortstack[l]{Beam monitors}} & Design &  &  &  &  &  &  &  &  &  &  &  &  &  &  &  &  &  &  &  & Jena\\ 
 &  & Construction &  &  &  &  &  &  &  &  &  &  &  &  &  &  &  & And &  &  &  & \\ 
 &  & Installation &  &  &  &  &  &  &  &  &  &  &  &  &  &  &  &  &  &  &  & \\ 
\cline{2-23}
 & \multirow{3}{*}{\shortstack[l]{Development of \\integration concept}} & Design & And & And &  &  &  &  &  &  &  &  &  &  &  & And &  &  &  &  &  & \\ 
 &  & Construction &  &  &  &  &  &  &  &  &  &  &  &  &  &  &  &  &  &  &  & \\ 
 &  & Installation &  &  &  &  &  &  &  &  &  &  &  &  &  &  &  &  &  &  &  & \\ 
 &  &  &  &  &  &  &  &  &  &  &  &  &  &  &  &  &  &  &  &  &  & \\

 \hline

\hline
\end{tabular}
\caption{Identified responsibilities for the different items required by the LUXE experiment, for the design, construction and installation. When a group is needed it is assigned with "And". If two groups can achieve the same task they are assigned and "Or".}
% \label{TC:Annex:Resources_WP65}
\end{table}
\end{landscape}% Landscape page

\begin{landscape}% Landscape page
\begin{table}[]
\tiny
\begin{tabular}{|p{0.1\linewidth}|p{0.1\linewidth}|p{0.07\linewidth}|p{0.015\linewidth}|p{0.02\linewidth}|p{0.02\linewidth}|p{0.02\linewidth}|p{0.02\linewidth}|p{0.02\linewidth}|p{0.02\linewidth}|p{0.02\linewidth}|p{0.02\linewidth}|p{0.02\linewidth}|p{0.015\linewidth}|p{0.015\linewidth}|p{0.015\linewidth}|p{0.015\linewidth}|p{0.015\linewidth}|p{0.015\linewidth}|p{0.015\linewidth}|p{0.02\linewidth}|p{0.02\linewidth}|p{0.04\linewidth}|}
\hline

Workpackage & Item &  & FH & MEA & ZBAU & MDI & MVS & MCS & MSK & MPS & MPC & MKK & D3 & D5 & IT & IPP & MR & ZM3 & ZM5 & \euxfel Company & External company & Other institute\\

\multirow{5}{*}{\shortstack[l]{7) Interaction\\ Chamber}} &  &  &  &  &  &  &  &  &  &  &  &  &  &  &  &  &  &  &  &  &  & \\ 
\hline
\cline{2-23}
 &\multirow{3}{*}{\shortstack[l]{Vacuum system}} & Design & And &  &  &  & And &  &  &  &  &  &  &  &  &  &  &  &  &  &  & \\ 
 &  & Construction &  &  &  &  & And &  &  &  &  &  &  &  &  &  &  &  &  &  & And & \\ 
 &  & Installation & And & And &  &  & And &  &  &  &  &  &  &  &  &  &  &  &  &  &  & \\ 
\cline{2-23}
 &\multirow{3}{*}{\shortstack[l]{Services}} & Design &  & And &  &  &  &  &  &  &  & And &  &  & And &  &  &  &  &  &  & \\ 
 &  & Construction &  & And &  &  &  &  &  &  &  & And &  &  & And &  &  &  &  &  &  & \\ 
 &  & Installation &  & And &  &  &  &  &  &  &  & And &  &  & And &  &  &  &  &  &  & \\ 
\cline{2-23}
 &\multirow{3}{*}{\shortstack[l]{Inner components}} & Design & And &  &  &  &  &  &  &  &  &  &  &  &  &  &  &  &  &  &  & Jena\\ 
 &  & Construction & And &  &  &  &  &  &  &  &  &  &  &  &  &  &  &  &  &  &  & Jena\\ 
 &  & Installation & And &  &  &  &  &  &  &  &  &  &  &  &  &  &  &  &  &  &  & Jena\\ 
\cline{2-23}
 &\multirow{3}{*}{\shortstack[l]{Monitoring}} & Design & And &  &  &  &  &  &  &  &  &  &  &  &  &  &  &  &  &  &  & Jena\\ 
 &  & Construction & And &  &  &  &  &  &  &  &  &  &  &  &  &  &  &  &  &  &  & Jena\\ 
 &  & Installation & And &  &  &  &  &  &  &  &  &  &  &  &  &  &  &  &  &  &  & Jena\\ 
\cline{2-23}
 &\multirow{3}{*}{\shortstack[l]{Positioning \\and survey}} & Design & And & And &  &  &  &  &  &  &  &  &  &  &  &  &  &  &  &  &  & \\ 
 &  & Construction &  &  &  &  &  &  &  &  &  &  &  &  &  &  &  &  &  &  &  & \\ 
 &  & Installation & And & And &  &  &  &  &  &  &  &  &  &  &  &  &  &  &  &  &  & \\ 
\hline
\end{tabular}
\caption{Identified responsibilities for the different items required by the LUXE experiment, for the design, construction and installation. When a group is needed it is assigned with "And". If two groups can achieve the same task they are assigned and "Or".}
% \label{TC:Annex:Resources_WP65}
\end{table}
\end{landscape}% Landscape page

\begin{landscape}% Landscape page
\begin{table}[]
\tiny
\begin{tabular}{|p{0.1\linewidth}|p{0.1\linewidth}|p{0.07\linewidth}|p{0.015\linewidth}|p{0.02\linewidth}|p{0.02\linewidth}|p{0.02\linewidth}|p{0.02\linewidth}|p{0.02\linewidth}|p{0.02\linewidth}|p{0.02\linewidth}|p{0.02\linewidth}|p{0.02\linewidth}|p{0.015\linewidth}|p{0.015\linewidth}|p{0.015\linewidth}|p{0.015\linewidth}|p{0.015\linewidth}|p{0.015\linewidth}|p{0.015\linewidth}|p{0.02\linewidth}|p{0.02\linewidth}|p{0.04\linewidth}|}
\hline

Workpackage & Item &  & FH & MEA & ZBAU & MDI & MVS & MCS & MSK & MPS & MPC & MKK & D3 & D5 & IT & IPP & MR & ZM3 & ZM5 & \euxfel Company & External company & Other institute\\
\multirow{4}{*}{\shortstack[l]{8) Safety }} &  &  &  &  &  &  &  &  &  &  &  &  &  &  &  &  &  &  &  &  &  & \\ 
\hline
\cline{2-23}
 &\multirow{3}{*}{\shortstack[l]{Interlocks}} & Design &  & And &  &  &  &  &  & And &  &  & And &  &  &  & And &  &  &  &  & \\ 
 &  & Construction &  & And &  &  &  &  &  & And &  &  & And &  &  &  & And &  &  &  &  & \\ 
 &  & Installation &  & And &  &  &  &  &  & And &  &  & And &  &  &  & And &  &  &  &  & \\ 
\cline{2-23}
 &\multirow{3}{*}{\shortstack[l]{Radiation \\protection\\ monitoring}} & Design &  &  &  &  &  &  &  &  &  &  & And &  &  &  & And &  &  &  &  & \\ 
 &  & Construction &  &  &  &  &  &  &  &  &  &  & And &  &  &  & And &  &  &  &  & \\ 
 &  & Installation &  &  &  &  &  &  &  &  &  &  & And &  &  &  & And &  &  &  &  & \\ 
\cline{2-23}
 &\multirow{3}{*}{\shortstack[l]{Other safety \\monitorings}} & Design &  &  &  &  &  &  &  &  &  &  &  & And &  &  &  &  &  &  &  & \\ 
 &  & Construction &  &  &  &  &  &  &  &  &  &  &  & And &  &  &  &  &  &  &  & \\ 
 &  & Installation &  &  &  &  &  &  &  &  &  &  &  & And &  &  &  &  &  &  &  & \\ 
\cline{2-23}
 &\multirow{3}{*}{\shortstack[l]{Safety concepts}} & Design &  &  &  &  &  &  &  &  &  &  &  &  &  &  & And &  &  & And &  & \\ 
 &  & Construction &  &  &  &  &  &  &  &  &  &  &  &  &  &  &  &  &  &  &  & \\ 
 &  & Installation &  &  &  &  &  &  &  &  &  &  &  &  &  &  &  &  &  &  &  & \\

\hline
\end{tabular}
\caption{Identified responsibilities for the different items required by the LUXE experiment, for the design, construction and installation. When a group is needed it is assigned with "And". If two groups can achieve the same task they are assigned and "Or".}
% \label{TC:Annex:Resources_WP65}
\end{table}
\end{landscape}% Landscape page

\subsection*{Extra figures}
\label{sec:Appendix:Extrafig}
\begin{figure}[ht]
   \centering
   \includegraphics*[height=8cm]{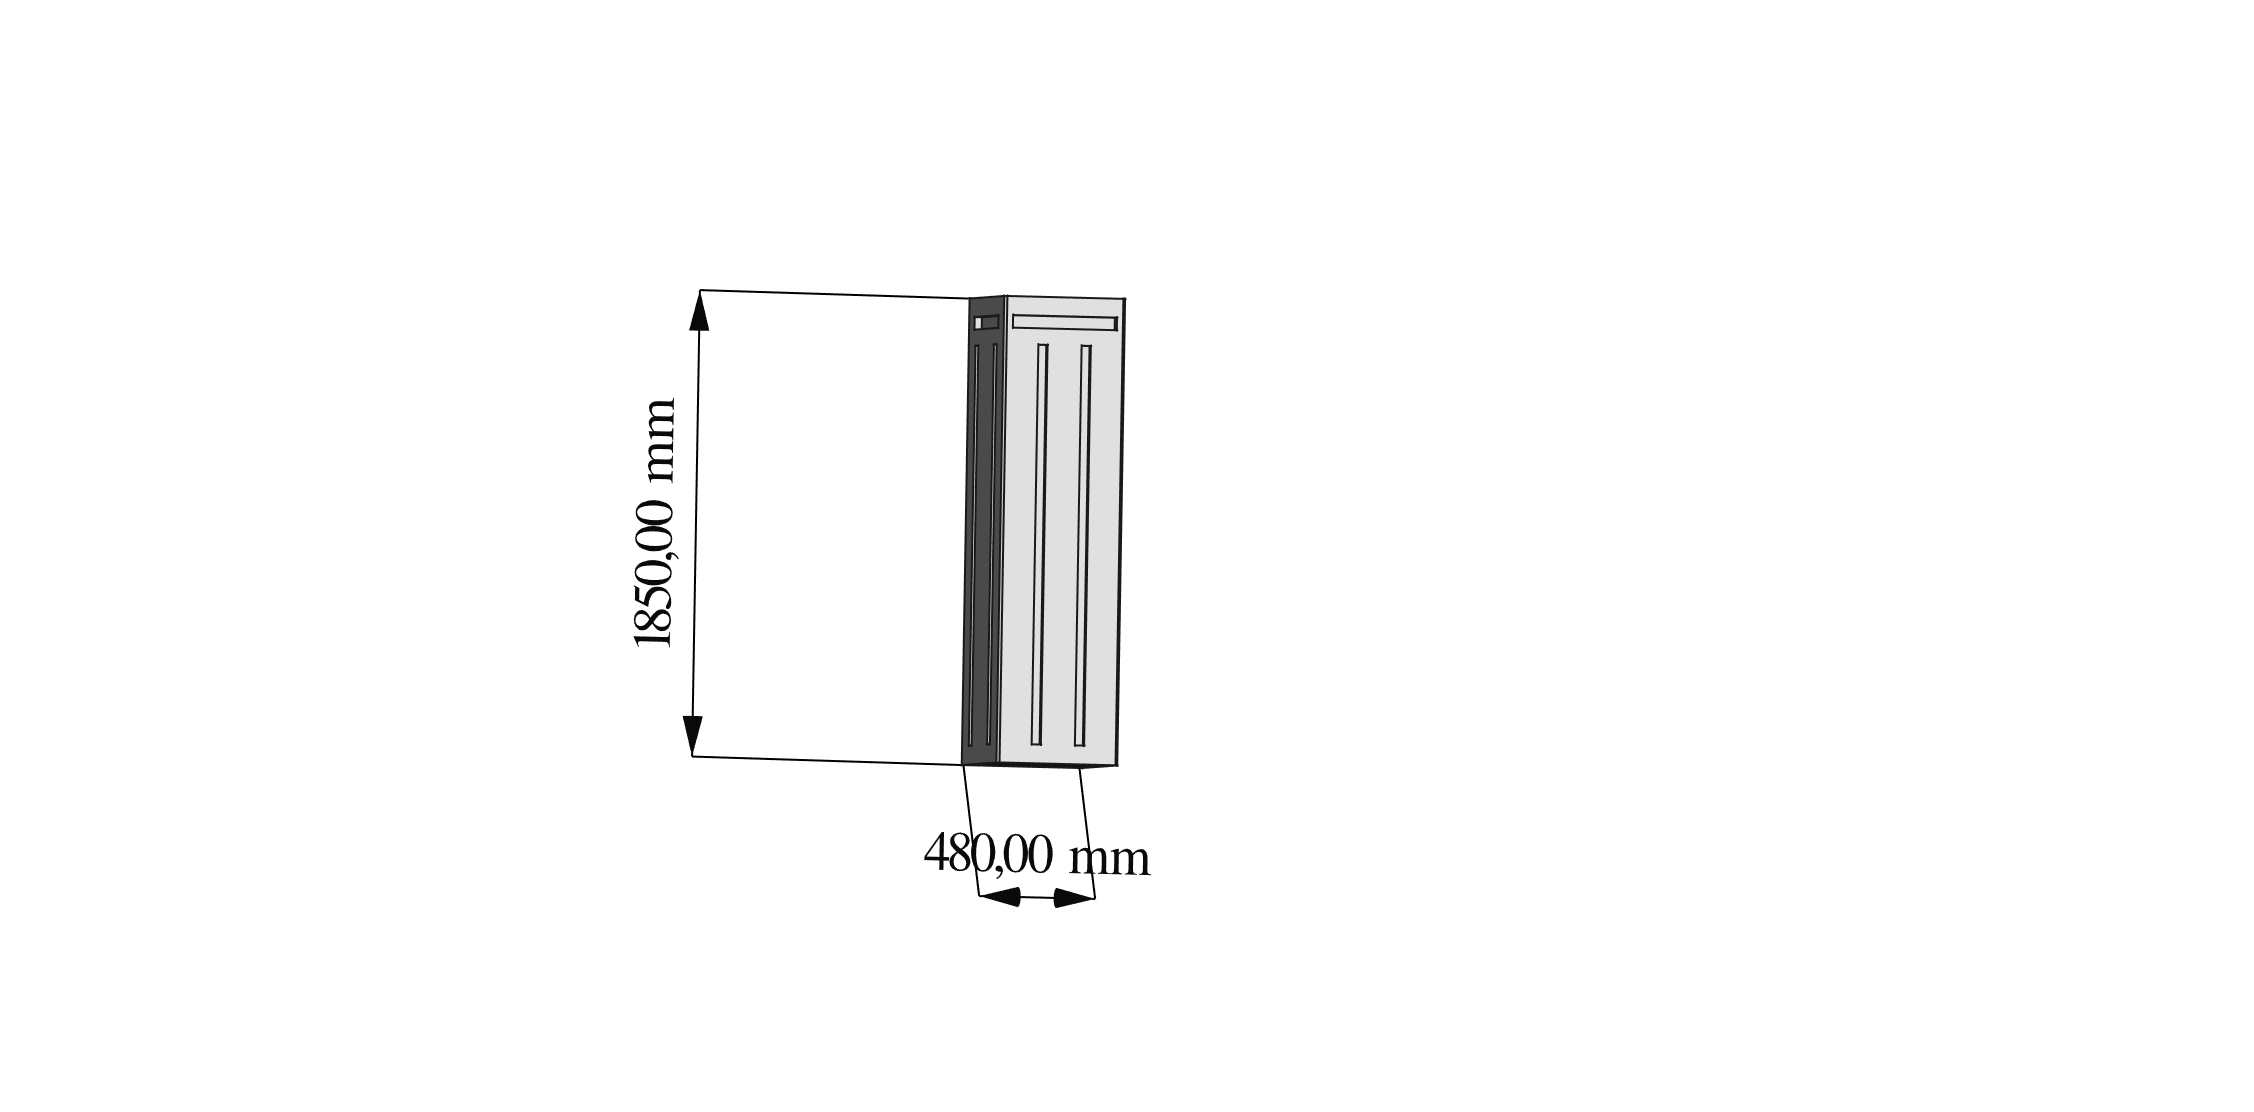} \hspace{2 cm} 
   \includegraphics*[height=8cm]{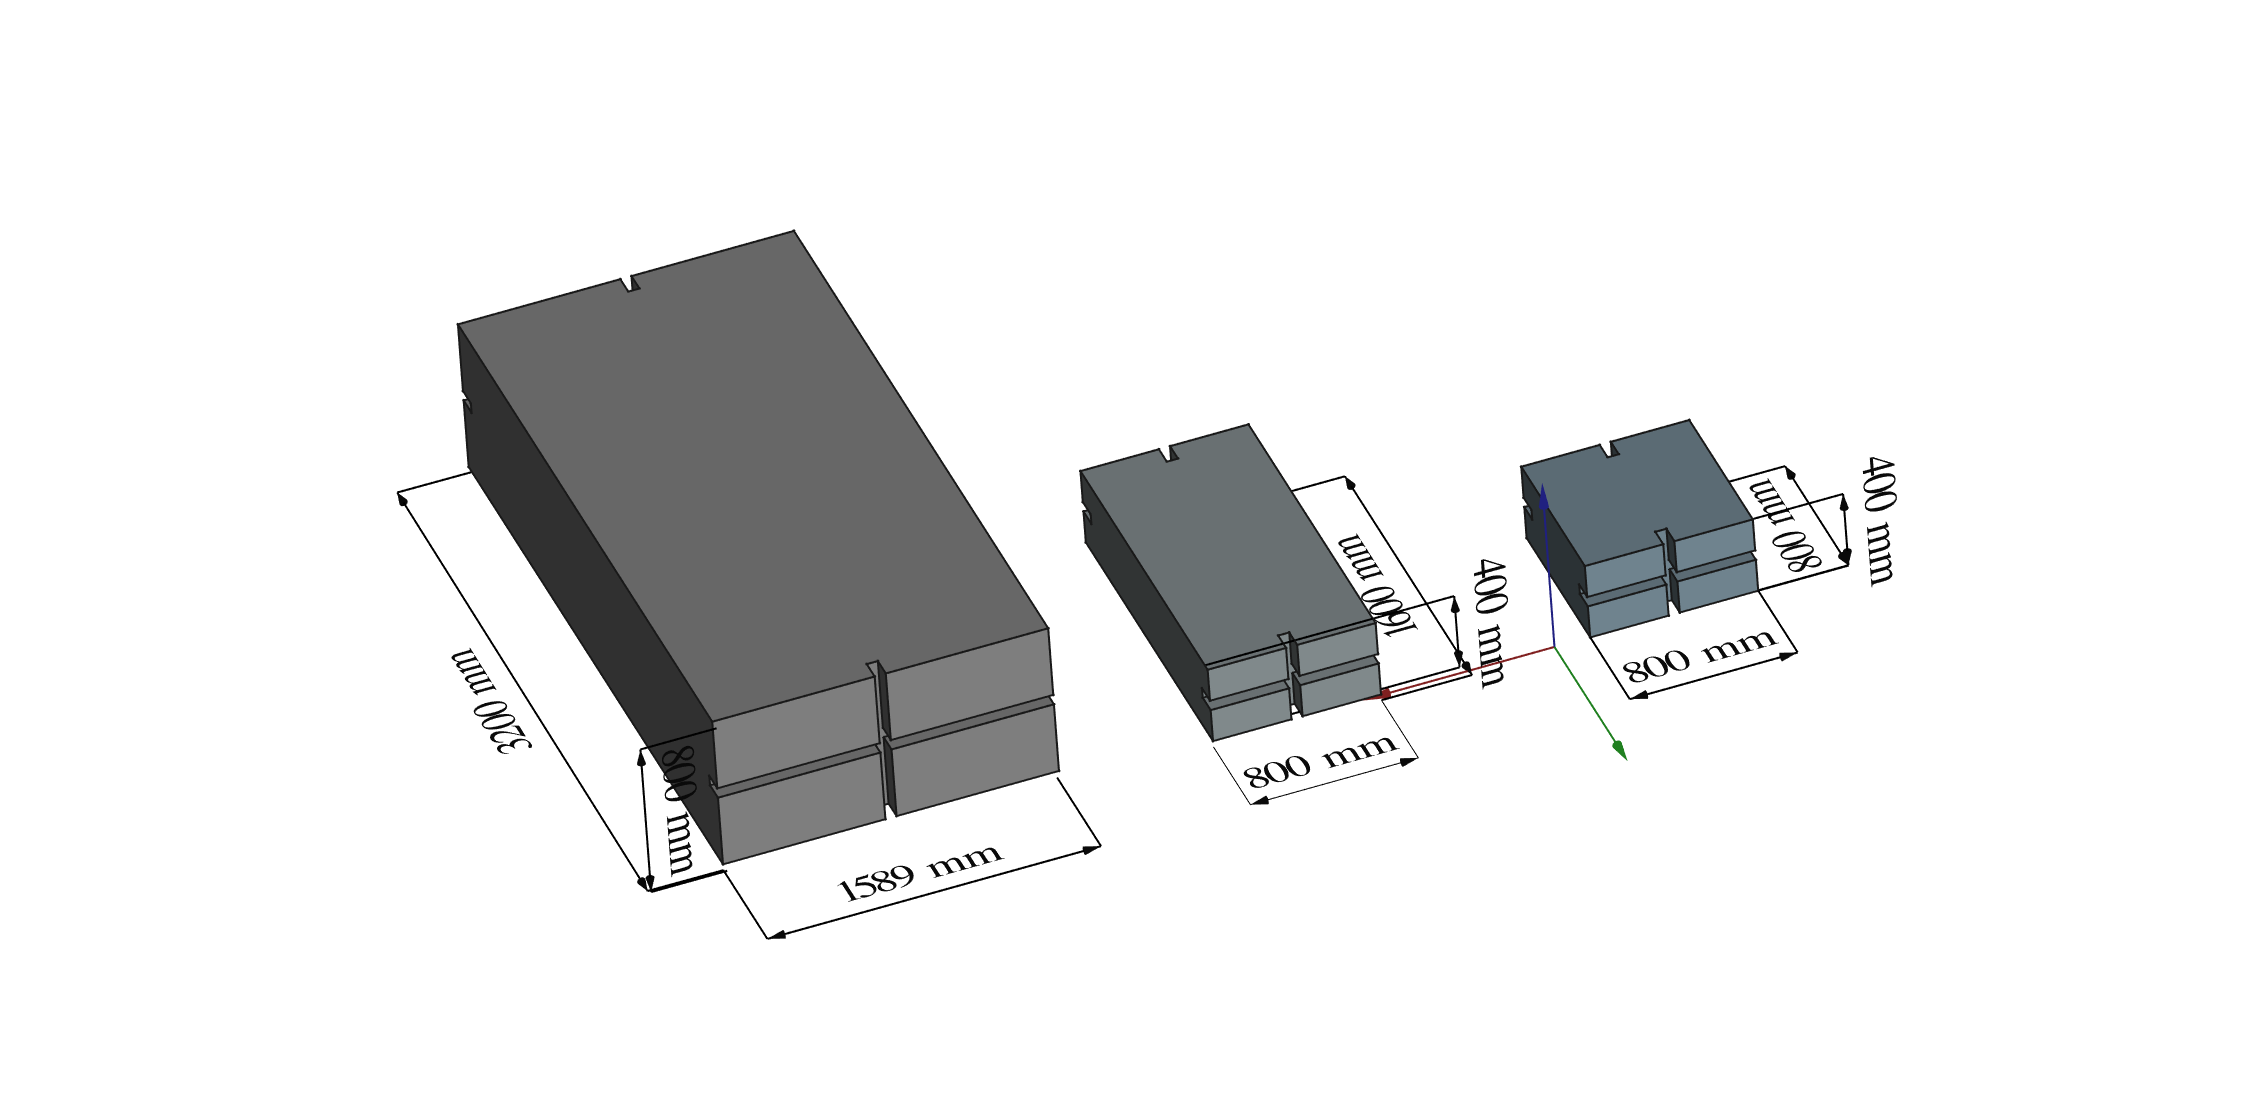}
   
   \caption{CAD drawing of the building elements used in the construction of the experiment, (Top) support structure element, (Bottom) concrete blocks used for shielding.
   \label{fig:LUXE_CAD_SupportAndShieldingElements}}
\end{figure}

%A test change for committing by Ruth
