# Supplementary material for: Technical Design Report for the LUXE Experiment
Source: arXiv:2308.00515 source file (2023-08-02)
Supplement: Supplementary file 2 [file appendix_ProjectManagement.tex]

% Discuss here how PM is structured in LUXE
\chapterauthors{R.~Jacobs \\\desyaffil}

\chaptabstract{This chapter contains an overview of the LUXE project management and project organisation of the LUXE experiment, as well as a summary of the major items planning and resources scheduling.}

\section{Project Structure}
\label{ref:proj_structure}

\begin{table}
\begin{center}
\begin{tabular}{|c|c|p{5cm}|}
    \hline
    \textbf{WP \#} & \textbf{WP Name} & \textbf{Description}\\\hline
    1 & Laser, Optics, Diagnostics & LUXE Terawatt optical laser system, beamline optics, diagnostics suite\\\hline
    2 & Vacuum Systems & Electron and Laser beam pipes, chambers, pumps, control software \\\hline
    3 & Magnets & Experiment dipole magnets, power and cooling \\\hline
    4 & Beam Dumps & Electron and photon beam dumps, shielding, cooling \\\hline
    5 & Detectors & LUXE particle detectors \\\hline
    6 & Electron Beam Control & Beam monitoring, control, timing \\\hline
    7 & DAQ, Computing, Core Software & Data acquisition, reconstruction, processing, storage \\\hline
    8 & Theory, MC, Simulation & SFQED Signal simulation, Geant 4 detector simulation \\\hline
    9 & Surface Building & Building hosting the Laser cleanroom, control room, counting room \\\hline
    10 & Service Infrastructure & Building media services for XS1 and surface building \\\hline
    11 & Laser Cleanroom & Cleanroom interior \\\hline
    12 & Experiment Integration & Integration concept for the experiment, integrated design \\\hline
    13 & Operations & Experiment operations concept \\\hline
    14 & Safety & LUXE safety concept and safety-related infrastructure \\\hline
    15 & Technical Coordination & Central cordination and support of activities in all WP \\\hline
    16 & Project Management & Project organization, planning, tracking, resources, documentation, risks \\\hline
\end{tabular}
\caption{LUXE WBS highest level elements. }
\label{tab:wbs}
\end{center}
\end{table}

The LUXE project structure is defined by its two base project management documents, namely the work breakdown structure (WBS) and the product breakdown structure (PBS). The WBS lists and groups tasks that need to be completed to realize, operate and maintain the LUXE experimental complex. The PBS is a structured list of all components and deliverables of the LUXE experimental complex. Both WBS and PBS are closely linked. Table~\ref{tab:wbs} summarizes the highest level of the LUXE WBS elements. The WBS structure intends to mirror the areas of responsibilities of technical service groups during lifecycle of the experiment. Each WBS element, or work package, is provided with a scoping statement that precisely describes the scope of each task and the desired outcome. Finally, each WBS element is linked to one or several deliverables, i.e. an element of the PBS. For the sake of brevity, the scoping statements and list of deliverables have been omitted. Fig.~\ref{fig:wbspbs} shows a graphical representation of the LUXE WBS and PBS. \\

\begin{figure}[htbp!]
    \centering
    \begin{subfigure}{0.5\textwidth} 
    \includegraphics[width=\textwidth]{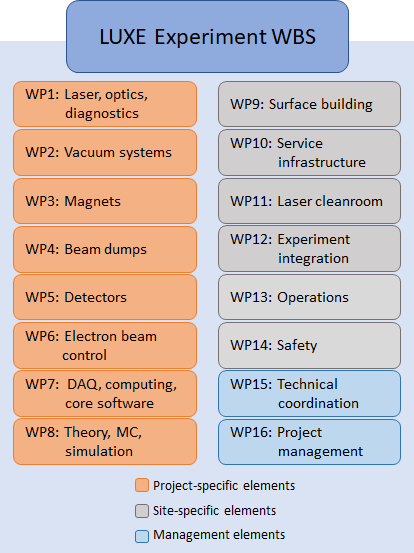}
    \caption{ }
    \end{subfigure}
    \begin{subfigure}{0.5\textwidth} 
    \includegraphics[width=\textwidth]{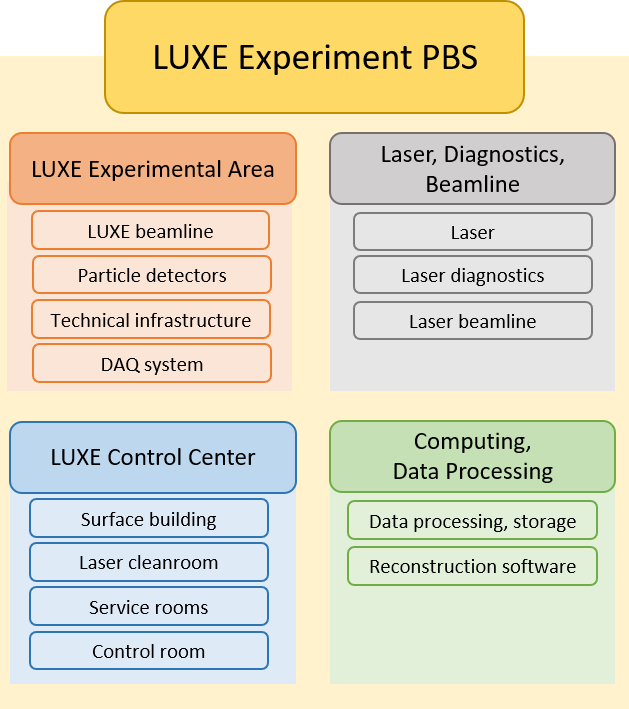}
    \caption{ }
    \end{subfigure}
    \caption{a) LUXE work breakdown structure (WBS). b) LUXE product breakdown structure (PBS). }
     \label{fig:wbspbs}   
\end{figure}

The WBS is used as basis for all further project management activities and documents. The tasks listed in the WBS enter the schedule and resource estimates, and are linked to the project documentation using a so-called project lifecycle management (PLM) tool.\\

\section{Organisational Structure}

The LUXE collaboration currently consists of 19 international institutes and about 100 members. Fig.~\ref{fig:luxemap} shows a map of Europe with the locations of the LUXE collaborating institutes indicated. There is interest from more institutions.

\begin{figure}
    \centering
    \includegraphics[width=0.75\textwidth]{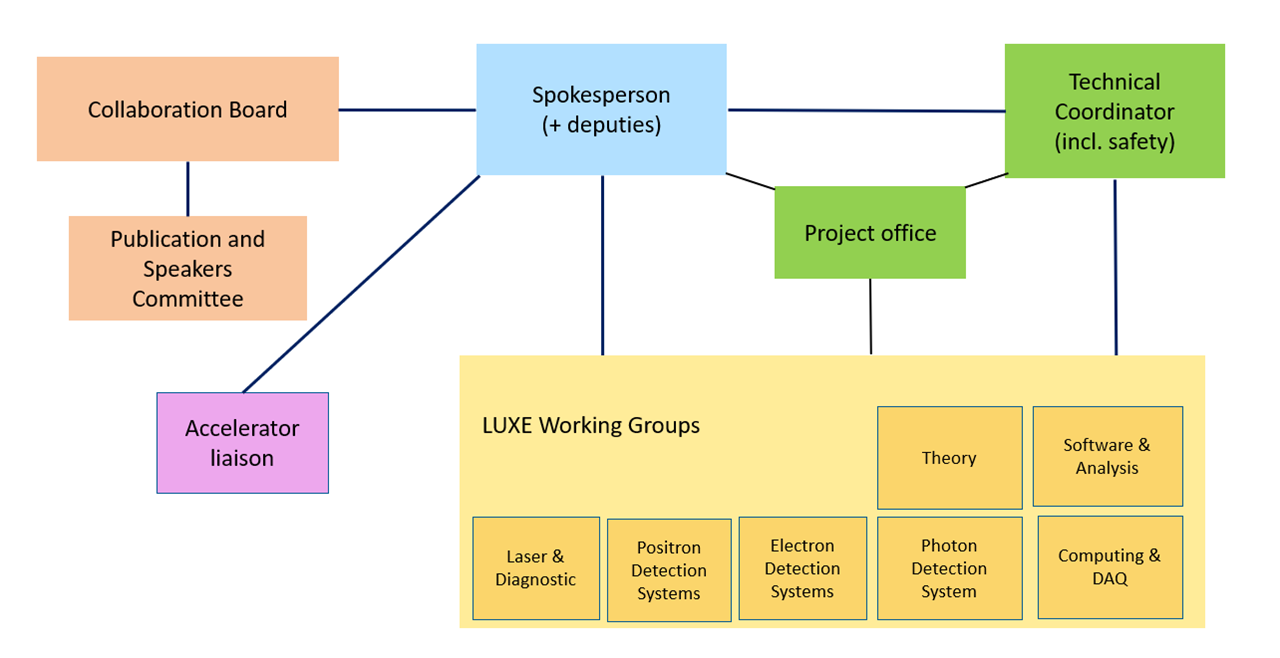}
    \caption{LUXE Organigram.}
        \label{fig:organigram}
\end{figure}

\begin{figure}
    \centering
    \includegraphics[width=0.75\textwidth]{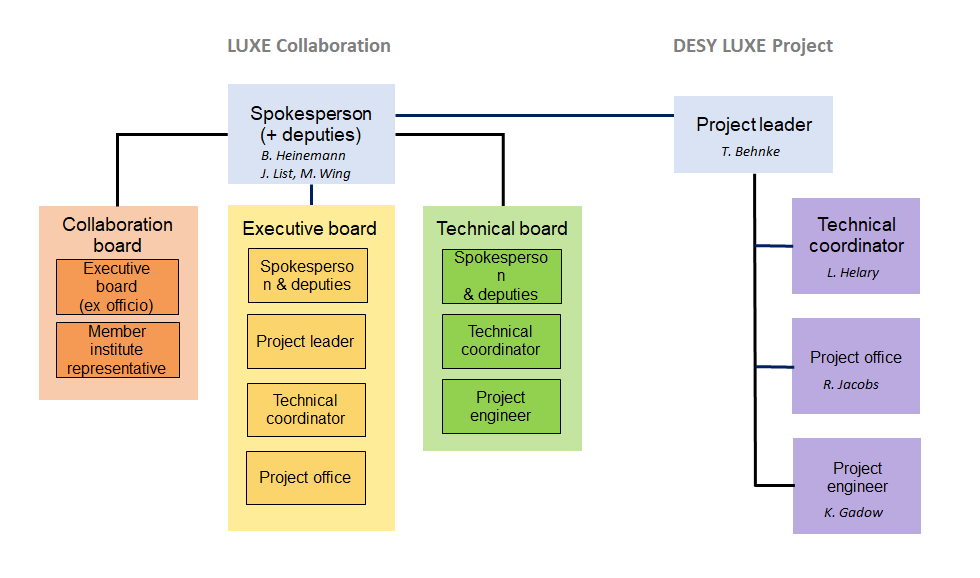}
    \caption{LUXE-DESY Organigram.}
        \label{fig:organigram-DESY}
\end{figure}

\begin{figure}
    \centering
    \includegraphics[width=0.75\textwidth]{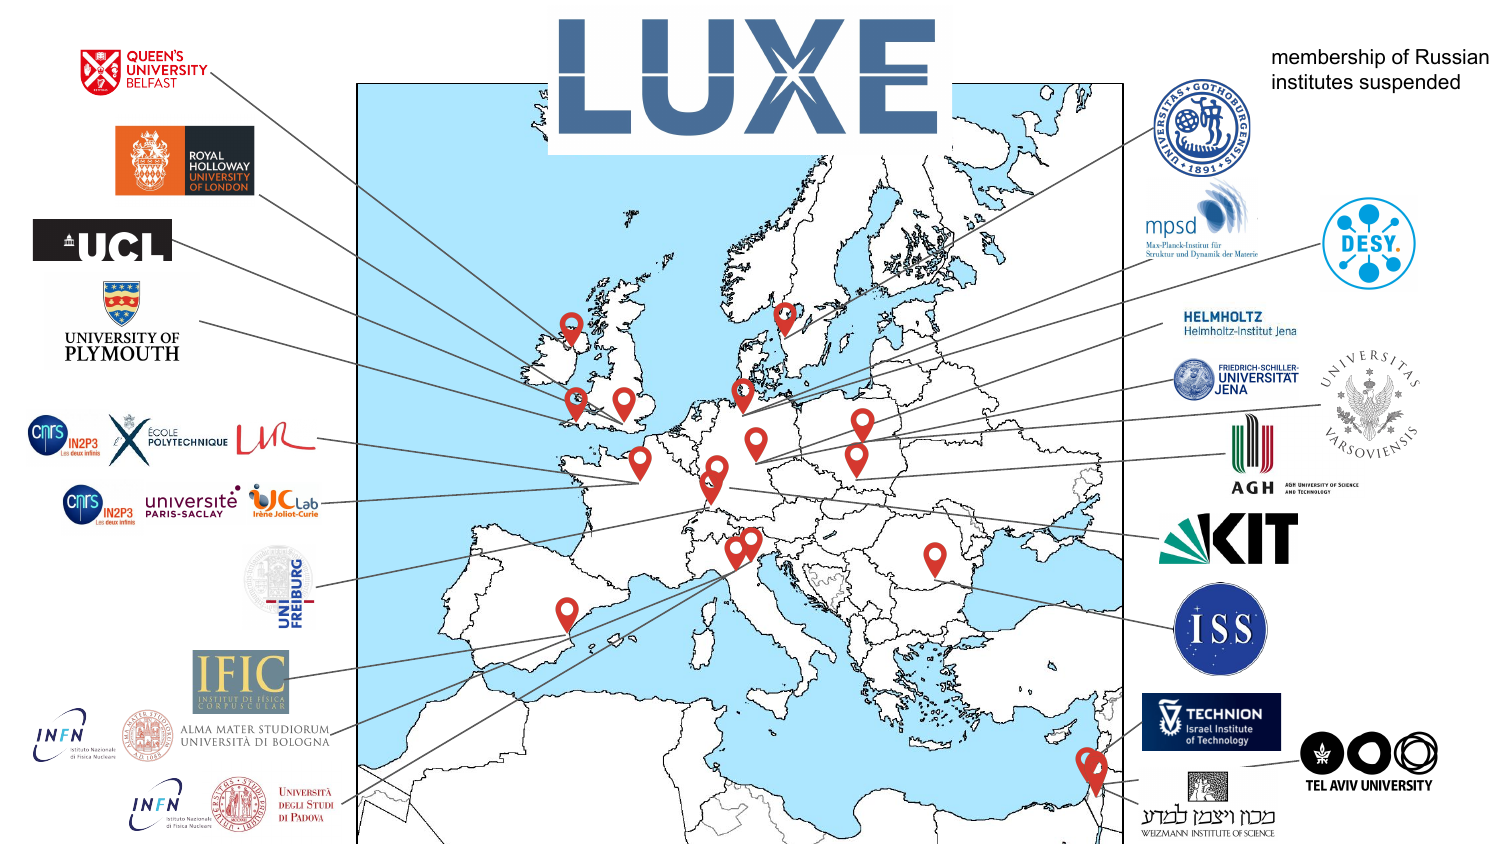}
    \caption{LUXE collaboration participating institutes map, as of early 2023.}
        \label{fig:luxemap}
\end{figure}

The LUXE organisational structure is summarized in the organigram shown in fig.~\ref{fig:organigram}. The interrelation between the LUXE collaboration and DESY as the experiment host lab is indicated in fig.~\ref{fig:organigram-DESY}, with the persons in their role as of beginning of 2023.

\begin{table}
\begin{center}
\begin{tabular}{|p{0.25\textwidth}|p{0.5\textwidth}|}
    \hline
    \textbf{Area} & \textbf{Responsible Institutes} \\\hline
    Technical Infrastructure & Deutsches Elektronen-Synchrotron (DESY), (overall coordination)
Royal Holloway University London (RHUL),  (beam simulation) \\\hline
    Laser \& Diagnostics & Friedrich-Schiller University Jena, Helmholtz Institute Jena,
(Laser, diagnostics, overall coordination)
Deutsches Elektronen-Synchrotron (DESY), (Infrastructure)
Tel Aviv University, (IP chamber)
Max Planck Institute for the Structure and Dynamics of Matter (MPI), (overall coordination)\\\hline
    Positron Detection Systen & AGH-University of Technology (AGH-UST) Cracow,
Institute of Space Science (ISS) Bucharest,
Tel Aviv University (TAU),
Laboratoire Leprince Ringuet (LLR) Palaiseau,
Irene Joliot Curie Lab (JCLab) Orsay,
University of Warsaw,
Instituto de Fisica Corpuscular (IFIC)
(Electromagnetic Calorimeter),
Weizmann Institute of Science (Pixel Tracker)\\\hline
    Electron Detection System & University College London (UCL) (Scintillator Screen \& Camera system),
Deutsches Elektronen-Synchrotron (DESY) (Cherenkov Detector)\\\hline
    Photon Detection System & IINFN Bologna, INFN Padova, The Queen’s University of Belfast
(Gamma Beam Profiler),
The Queen’s University of Belfast (Gamma Ray Spectrometer),
Deutsches Elektronen-Synchrotron (DESY)
(Gamma Backscattering Calorimeter)  \\\hline
    DAQ, Core Software \& Computing & Deutsches Elektronen-Synchrotron (DESY), University College London (UCL), Weizmann Institute of Science \\\hline
    Theory \& Monte Carlo & University of Gothenburg, University of Plymouth + contributors \\\hline
    Technical Coordination \& Project Management & Deutsches Elektronen-Synchrotron (DESY) \\\hline
\end{tabular}
\caption{Areas of responsibility in LUXE.}
\label{tab:resp}
\end{center}
\end{table}

Table~\ref{tab:resp} summarizes different areas of responsibility for areas within the LUXE experimental complex.

\section{Resource-Loaded Schedule}

The LUXE project schedule is driven mainly by the design, procurement and production lead times of the major elements in the experimental complex, namely the laser cleanroom surface building and laser system as well as the dipole magnets, beam dumps and interaction vacuum chamber (see fig. \ref{fig:majitemtimeline}). The installation schedule of the LUXE experiment is primarily driven by the \euxfel shutdown schedule, which foresees each year an end-of-year shutdown (duration of order one month) and a short summer shutdown (duration of order two weeks). In addition an extended long shutdown for six months is foreseen in the second half of the year 2025.Preliminary installation works will start in the shorter summer and end-of-year shutdowns in the years leading up to 2025 and the main installation of the long-lead-time major beamline elements and detectors will take place in the long shutdown in 2025. It should be noted that the experiment installation can be staggered, such that an installation over several shorter \euxfel shutdowns is possible.\\

\begin{figure}
    \centering
    \includegraphics[width=\textwidth]{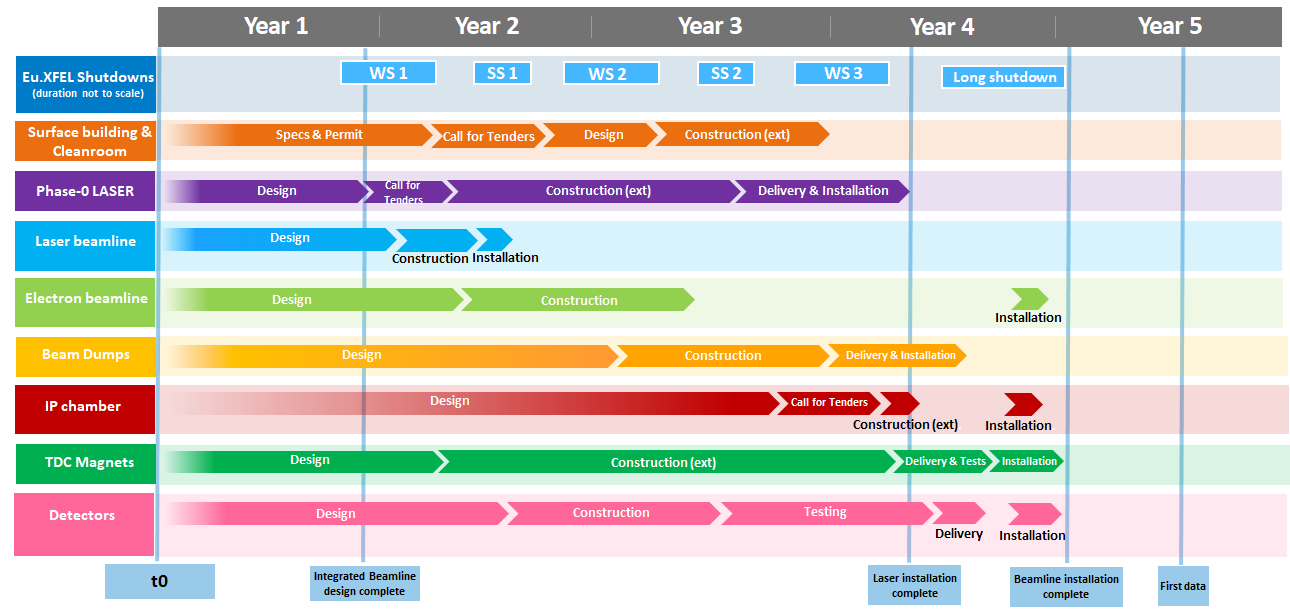}
    \caption{LUXE major items timeline.}
    \label{fig:majitemtimeline}
\end{figure}

The order of the installation works and duration of individual tasks as listed in tab.~\ref{TC:Annex:Milestone_WP11} to~\ref{TC:Annex:Milestone_WP15} and shown in fig.~\ref{fig:luxeschedule} has been discussed with the main contributing engineer of the LUXE project. The main boundary conditions to consider for the installation are the availability of space in the LUXE cavern, availability of transport such as forklift and crane, limited allowed number of workers, especially respecting parallel works on the XTD20 extraction beamline during the 2025 shutdown, as well as the ordering and manufacturing schedule of the long lead-time components in the beamline.

A preliminary schedule of the XTD20 extraction beamline installation was discussed in a recent meeting with the XFEL technical team. The team acknowledged that the next extraction line could be installed in a regular End-of-year shutdown of the facility assuming that the items required for the installation would be made available on time, and that sufficient well-trained person power would be made available for the duration of the installation. The installation of the transfer line to the experimental area could then be staged in regular shutdown as it would not impact the EU.XFEL operations. 

\begin{figure}[htbp!]
\centering
\includegraphics[width=0.75\textwidth]{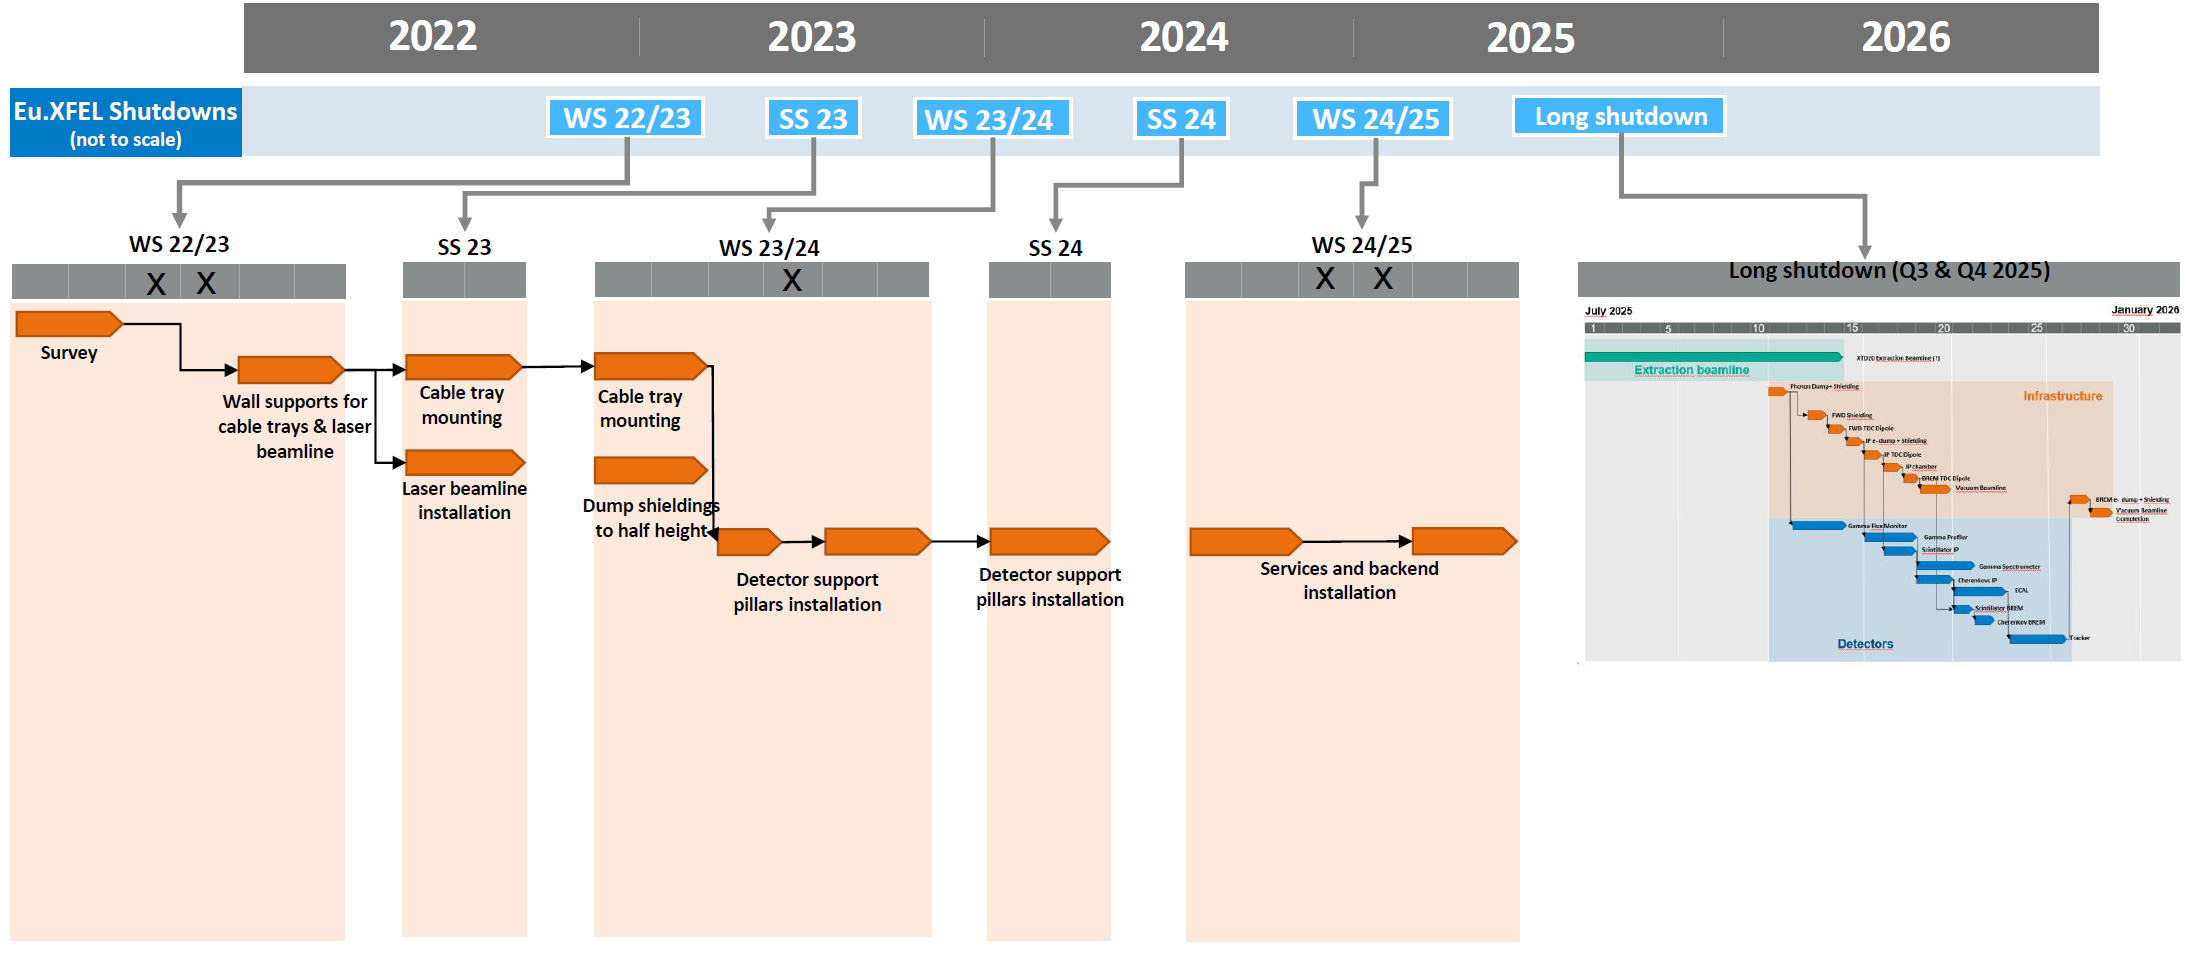}
\includegraphics[width=0.75\textwidth]{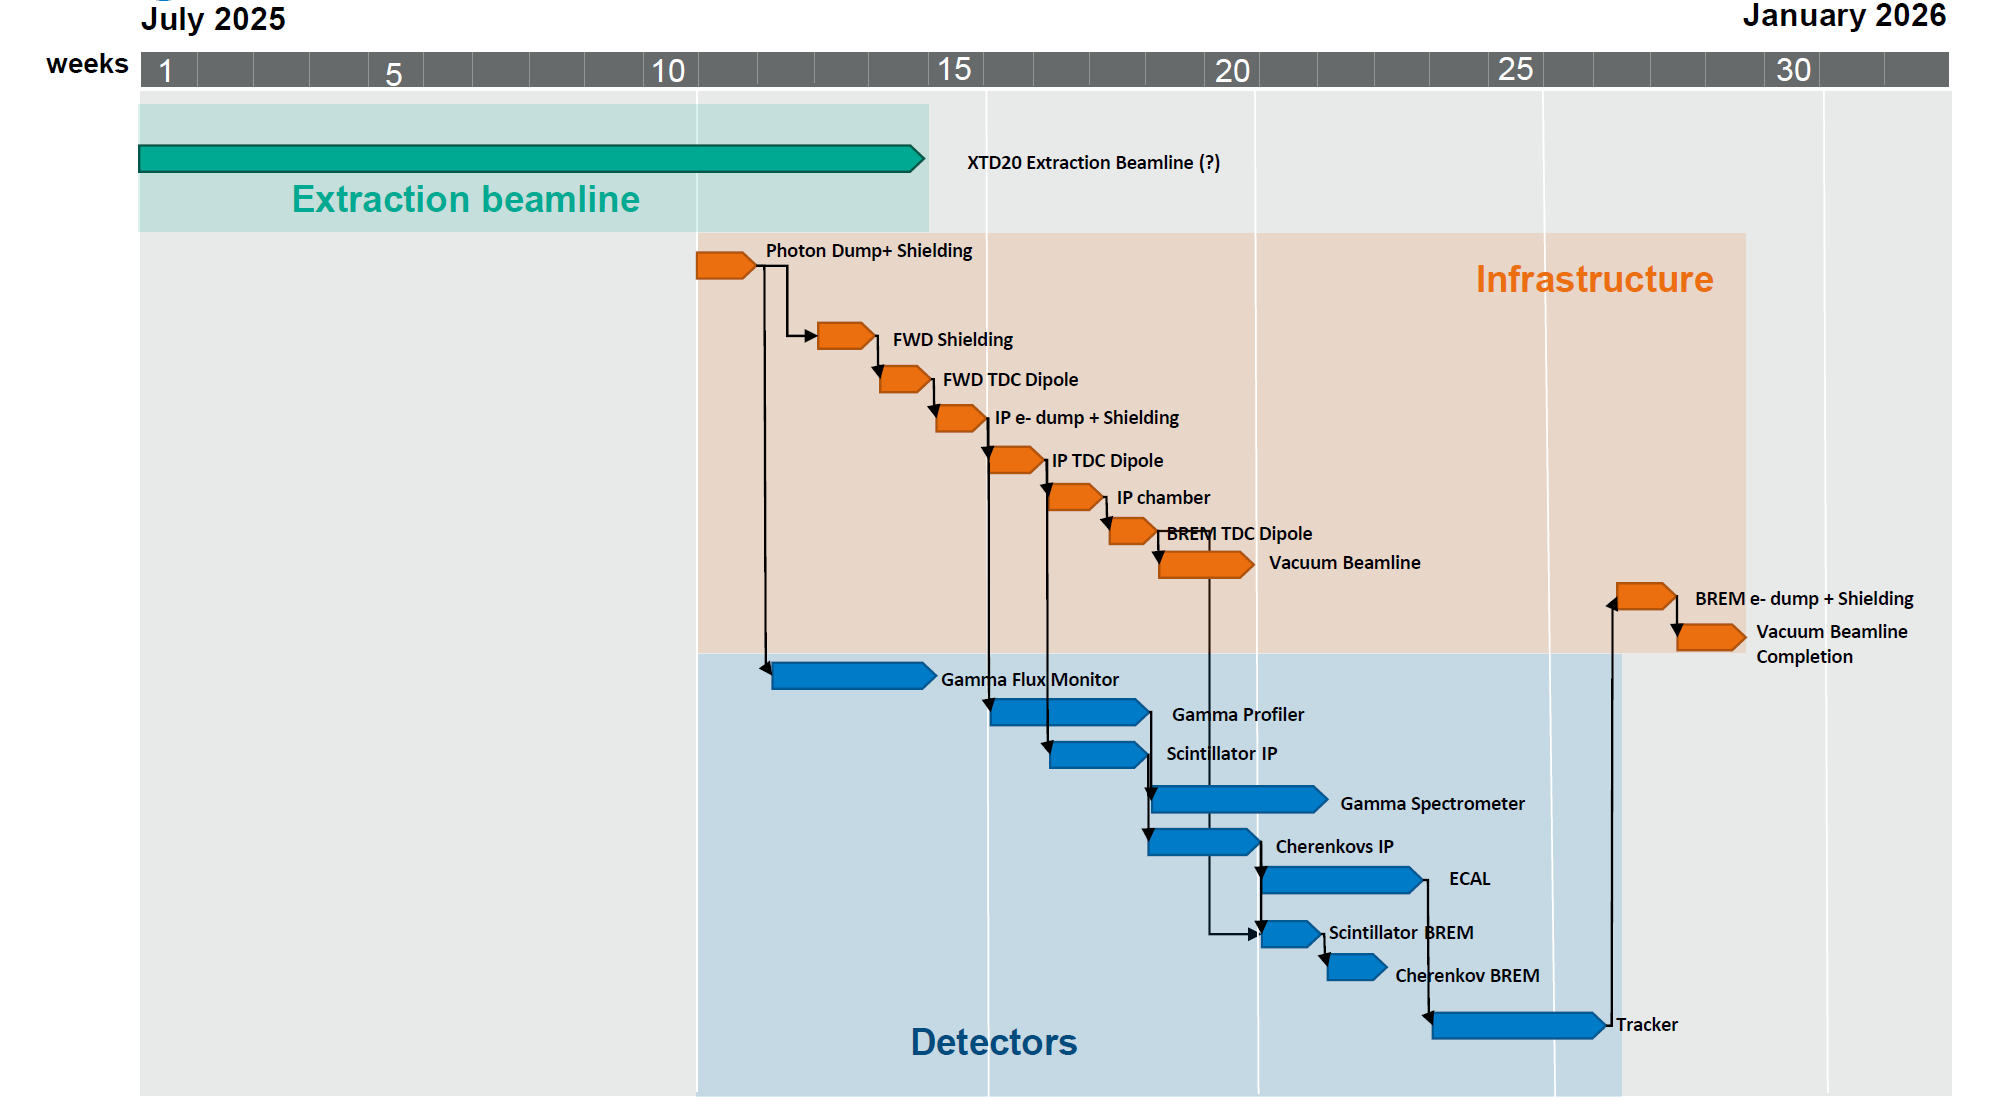} 
\caption{LUXE overall installation schedule (top). Detailed installation schedule in 2025 long shutdown (bottom).} 
\label{fig:luxeschedule} 
\end{figure}

\begin{figure}
    \centering
    \includegraphics[width=0.75\textwidth]{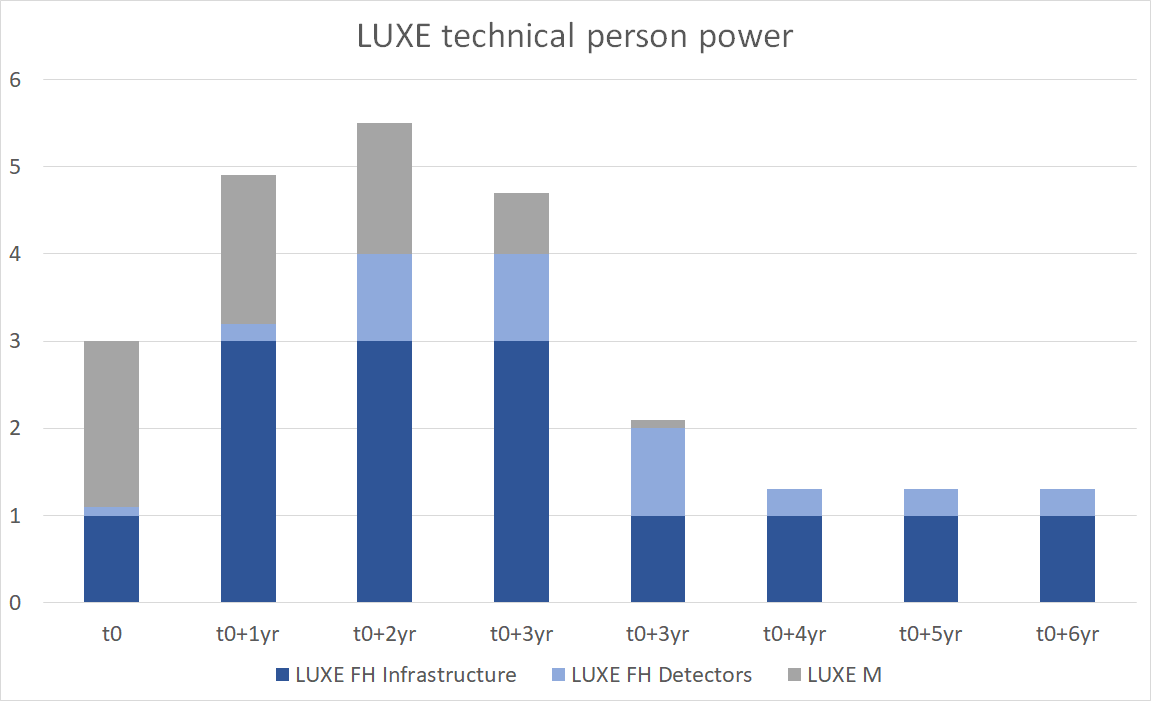}
    \caption{LUXE technical infrastructure FTE timeline by DESY technical groups,relative to the time of project start ($t_0$).}
    \label{fig:luxeinfftemap}
\end{figure}

%Fig.~\ref{fig:luxeinfftemap} shows the preliminary timeline of the DESY technical person-power needed for the design as well as the supervision of the manufacturing and installation of the LUXE technical infrastructure. The per-year FTE-need average is 2-3 FTE/year in FH and 1-2 FTE/year in the M-division, resulting in an integrated 18 FTE-years required in FH and 6 FTE-years in the M-division, in agreement with earlier estimates. The basis of estimate for this timeline is the list of tasks necessary to complete the infrastructure as shown in section~\ref{sec:Appendix:responsibilities}. Each task is fractionally assigned to one or several DESY groups according to the expertise profile needed. The scenario assumed in the timeline shown is that any task which lies in the expertise of FH technical personnel is completed to a major fraction by the FH personnel and technical personnel of other DESY groups is only used where necessary. A preliminary estimate of the duration, FTE and group participation needed for the individual tasks were made in discussion with the main contributing LUXE engineer and received feedback by the technical note review panel, resulting in fig.~\ref{fig:luxeschedule}. It should be emphasized that further discussions with the relevant experts from the accelerator groups are required to arrive at a more granular and precise estimate.

\begin{figure}
    \centering
    \includegraphics[width=0.75\textwidth]{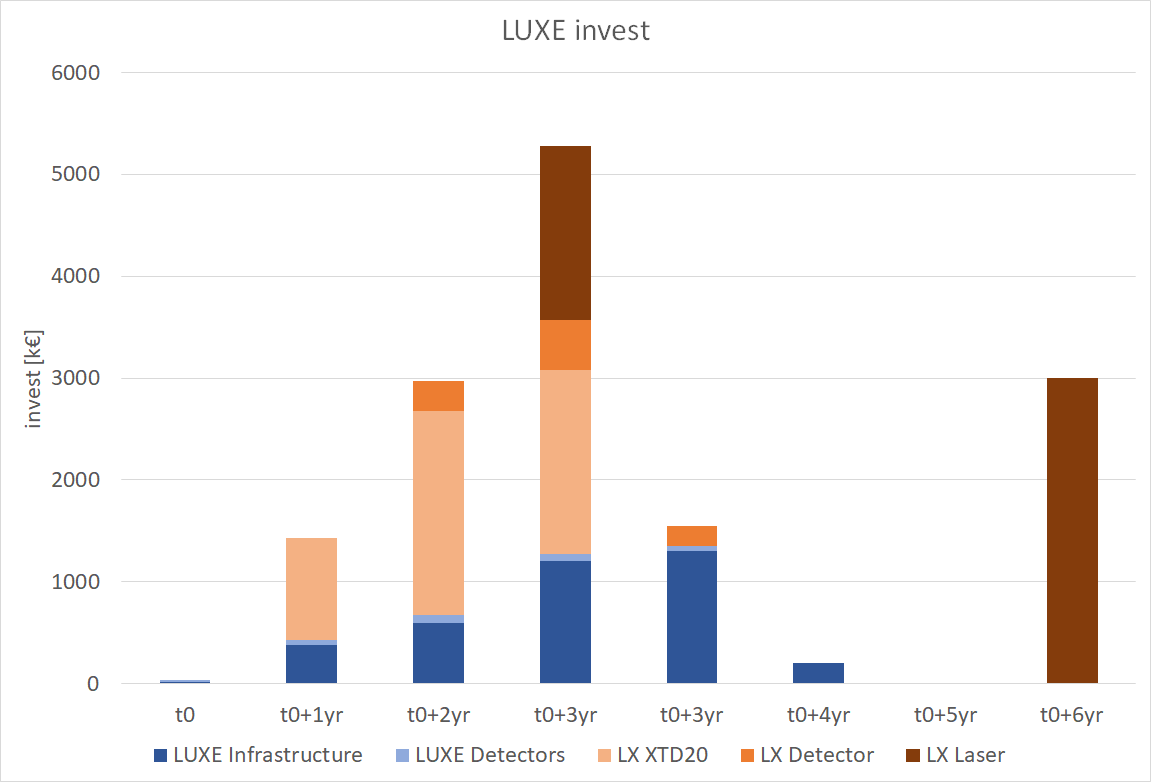}
    \caption{LUXE technical infrastructure spending profile, relative to the time of project start ($t_0$). Blue color and label \"LUXE\" indicate expected contributions from DESY, orange color and label \"LX\" indicate expected in-kind or third-party contributions.}
    \label{fig:luxeinfcostmap}
\end{figure}

%Finally, fig.~\ref{fig:luxeinfcostmap} shows a preliminary estimate of the invest cost schedule for the LUXE technical infrastructure relative to the time of project start ($t_0$). The integrated cost corresponds to 3.5MEUR with a yearly average spending of 1MEUR.  The timeline shown is based on the list of items and cost from the technical infrastructure note tab.~\ref{TC:Annex:Resources_WP61} to \ref{TC:Annex:Resources_WP64}. The cost model is made such that one separate core invest and material cost (in MEUR) and person power (in FTE) that is assumed to come from local resources (i.e. DESY groups, M or FH). The core invest estimates are based on (preliminary) quotes from vendors or on experience from experts at DESY. The estimates of the personnel resources needed come from experts. Overheads, escalation or contingency are not included. 

The current cost estimate for the experiment  is based on the list of items and cost shown in the technical infrastructure organisational appendix~\ref{app:orga_technicalinfra}. It amounts to approximately 15 Mio EUR in 2022 EUR, including the cost of the TD20 beamline. In many instances the estimate is based on a conceptual design of components and infrastructure, based on close interaction with experienced engineers with a background in building up similar experiments. The cost distribution across the different work packages is shown in figure~\ref{fig:luxewpcostfraction}.

\begin{figure}
    \centering
    \includegraphics[width=0.75\textwidth]{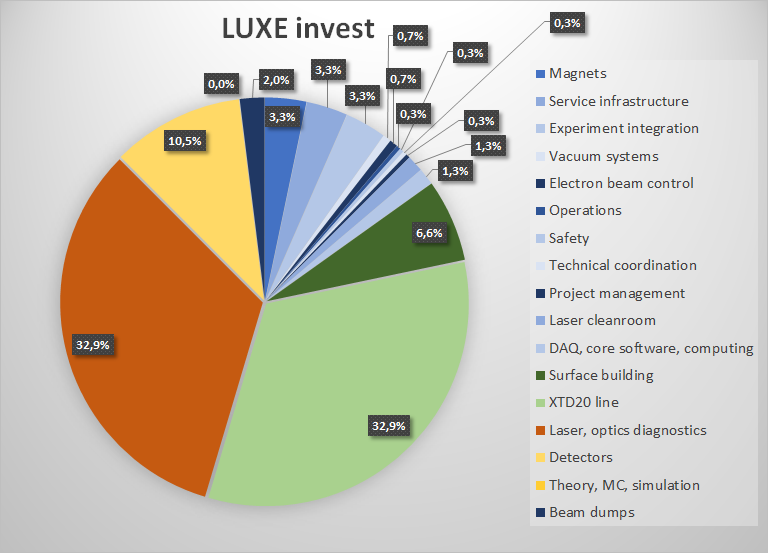}
    \caption{Budget fraction per LUXE work package, including the TD20 extraction beamline.}
    \label{fig:luxewpcostfraction}
\end{figure}

The cost model is separating core invest and material cost (in MEUR, see figure~\ref{fig:luxeinfcostmap}) from person power (in FTE-years, see figure~\ref{fig:luxeinfcostmap}) that is assumed to come from host-laboratory resources (i.e. DESY groups, M or FH) and external resources. The core invest estimates are based on (preliminary) quotes from vendors or on experience from experts at DESY. The estimates of the personnel resources needed come from experts. Overheads, escalation or contingency are not included. 

The total core investment, supported by DESY, has been estimated to be 3.5 MEUR, excluding the laser and extraction beamline . The LUXE detector investment of 1.1 MEUR will be covered to 20\% by DESY and 80\% by external contributions. The total person power required  has been estimated to be 18 FTE-years required in FH (including technical contributions from scientific personnel) and 6 FTE-years required in the M-division integrated from the time the LUXE project is approved (denoted $t_0$ in the following) over the following seven years. 

Several funding options are pursued to finance the LUXE experiment, in addition to the contribution from the DESY FH budget. An ERC Synergy grant application has been recently submitted (Prof. M. Wing principle investigator), with a funding volume of 14 MEUR, which would cover investment for equipment such as the laser system, the DAQ and computing infrastructure and parts of the detector system, and personnel costs. An application for a Horizon-Europe Infrastructure Consolidation grant to cover the TD20 extraction beamline is currently being pursued (coordinator: T. Behnke) which would cover the extraction beamline, target chamber, one magnet and two beam dumps at a total volume of 5MEUR. It is expected that parts of the infrastructure, e.g., the surface building at the Osdorfer Born, and other parts of the extraction beamline and experimental infrastructure, could be contributed to from the DESY strategic invest (about 7.5 MEUR). Other funding lines, including additional support from the BMBF, are being pursued. It should be noted that there is overlap between the items potentially covered by the ERC and the strategic investment in order to allow for contingency.

A significant contribution to LUXE is expected to consist of in-kind contributions from the collaboration member institutes (ca. 3 MEUR). Items covered by this are the LUXE particle detectors, the laser diagnostics, as well as the spectrometer vacuum chambers. The commitments of the LUXE member institutes are summarized in table 2. Several of the LUXE member institutes have funding applications ongoing.

\section{Risk assessment}

Dedicated risk estimates were made for every component of the LUXE experimental setup and documented in the respective systems technical notes. Tab.~\ref{tab:risk} summarizes the main risks for LUXE. The primary risks of the experiment are associated with the delay in approval and funding which can potentially result in a significant cost increase and delay in schedule. In particular the on-time completion of the XTD20 is critical, because its completion is a prerequisite for running LUXE. It is also important to note that it is likely that more in-kind contributions can be secured from other funding agencies. Discussions are ongoing in several areas. 

\begin{table}[h]
\begin{center}
\begin{longtable}{|p{0.1\textwidth}|p{0.15\textwidth}|p{0.1\textwidth}|p{0.1\textwidth}|p{0.15\textwidth}|p{0.15\textwidth}|}
    \hline
    \textbf{Name} & \textbf{Description} & \textbf{Impact on Cost} & \textbf{Impact on Schedule} & \textbf{Actions required} & \textbf{Mitigation}  \\\hline
    Delay of Approval & Approval of DESY directorate not forthcoming in timely manner & n.a. & High: Collaboration may lose interest & Early approval of directorate, decouple from funding & diversify funding \\\hline
    Delay of funding & Major cost items rely on external funding which is not yet confirmed & High: Inflation & High, especially for XTD20 beamline & Decision from funding agencies & diversify funding \\\hline
    DESY  Projects Schedule collision & LUXE schedule collides with other DESY high priority project & Low & High & Careful planning and Coordination with other DESY activities & Plan for contingencies in installation schedule \\\hline
    Cost increase for service infrastructure & Unforeseen extra material and infrastructure costs & Moderate, estimated 10-20\% & Low & Careful planning, vetting of resource estimate & Exploit synergies with other XFEL projects \\\hline
    Surface building cost increase & Market prices fluctuate drastically & High & Low & Plan for contingency & Exploit synergies with other XFEL projects \\\hline
    Major infrastructure items delay & Delay of delivery of major infrastructure item & Low & Moderate & Early identification of critical path & Develop backup plans for delays, use available components wherever possible \\\hline
    Laser diagnostics performance low & Delivered laser diagnostics performance is below technical specifications & Moderate & Low & Start effort early, 
    Careful testing & Complementary measurements, improve precision with time \\\hline
    Laser beamline optical components failure & Highly specialized system of expensive components & Moderate & Moderate & Careful testing of optical components, careful handling during installation & Plan for spares where expense allows \\\hline
    Delay in detector delivery & Detector system delivery is delayed & Low & Moderate & Plan for contingencies and minimal experimental setup & Plan for two complementary systems per location, run with minimal setup \\\hline
    
    \caption{Overview of risks and risk management strategies for the LUXE experiment}
    \label{tab:risk}
\end{longtable}
\end{center}
\end{table}
