# Supplementary material for: Technical Design Report for the LUXE Experiment
Source: arXiv:2308.00515 source file (2023-08-02)
Supplement: Supplementary file 3 [file appendix.tex]

\section{The JETI40 Laser System}
 
JETI40 is a continuously developed system based on a commercial CPA platform (Amplitude Technologies). 

The JETI40 laser is a well-characterised system that is in continuous operation for over 10 years to this date and is used for high field science in Jena. %\BH{add since when, and it would be good to comment on a few more things it has achieved, e.g. stability. Maybe we can add 1-2 figures illustrating key performance parameters?} 
 It produces pulses down to $25$~fs duration of high quality (near the Fourier-transform limit in time and space) with maximum energy after compression exceeding $1$~J. A schematic layout of the systems is shown in Fig.~\ref{fig:JETI}, and this system can be transferred and installed at the LUXE experiment (in case the first option of buying new laser system does not happen). This power level is well suited for first stage of LUXE and will allow $\chi \sim 1$  to be achieved with focussing to a 3 $\mu$m laser spot size. 

\begin{figure}[ht]
    \centering
    \includegraphics[width=0.3\textwidth]{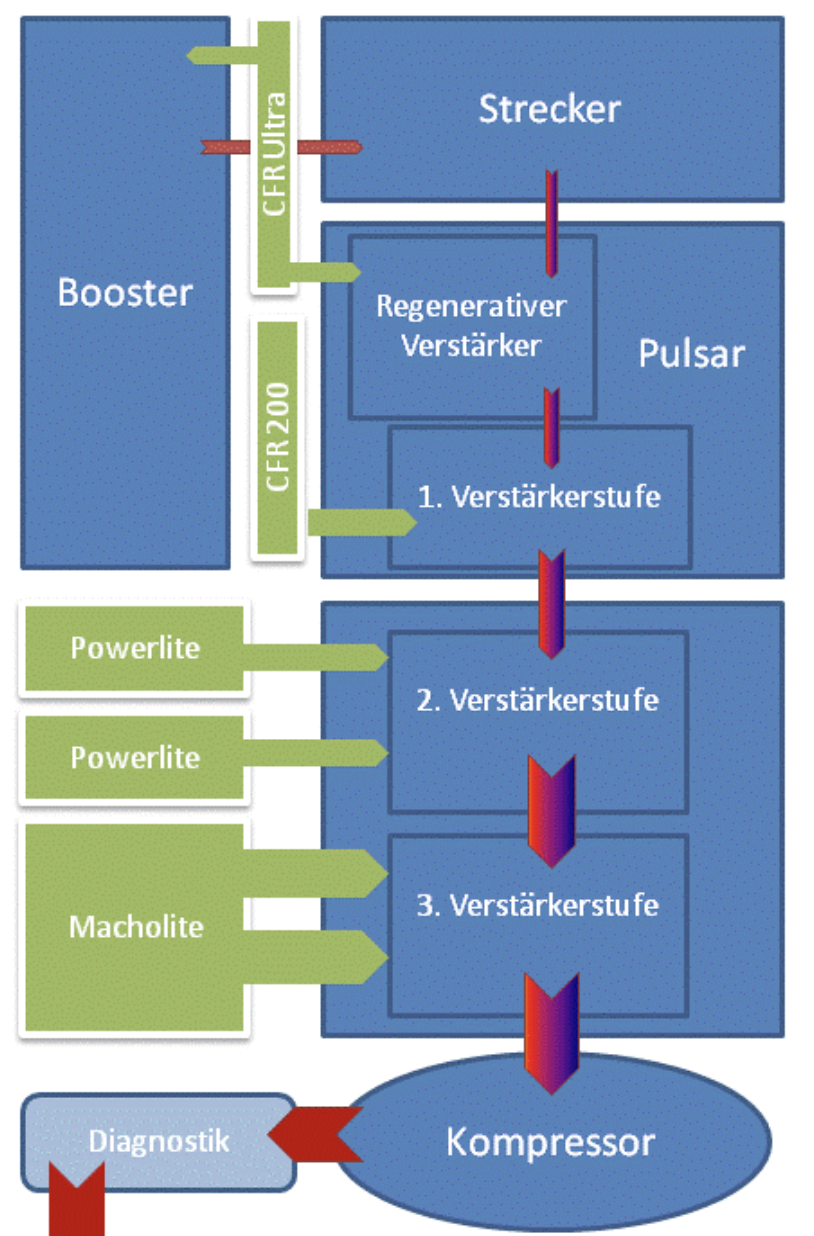}
    \includegraphics[width=0.3\textwidth]{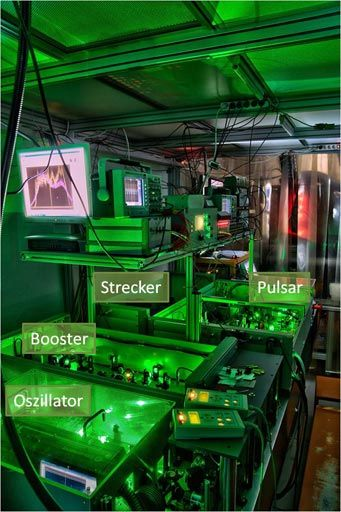}
    \includegraphics[width=0.315\textwidth]{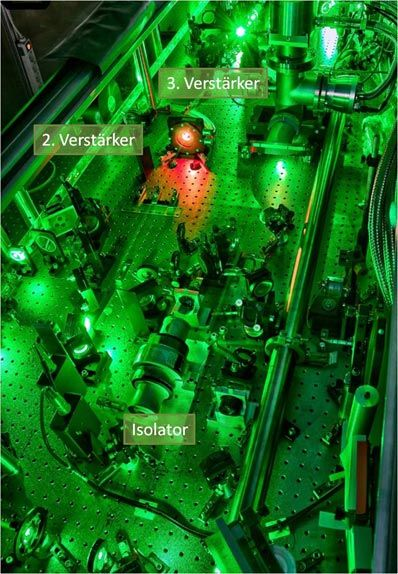}
    \caption{Schematic of the JETI system highlighting major assemblies. Current Installation of JETI40 at the University of Jena. Front end is shown in centre and power amplifiers right.}
    \label{fig:JETI}
\end{figure}

The detailed layout of the  JETI40 system and current installation is shown in 
Fig.~\ref{fig:JETI}. The schematic highlights the major components.

\begin{itemize} 
\item \textbf{Front end}\newline
The laser chain starts with a commercial femtosecond (fs) oscillator which delivers pulse train at $\approx 76.4$\,MHz (an integer fraction-1/17 of the \euxfel master clock rate of 1.3\,GHz). A key feature required of this oscillator (and also on the new laser system) is that the cavity length can be precisely matched to the  \euxfel master clock which is a SESAM-based mode-locked laser oscillator (Origami-15) \cite{lasoscsync}. The Origami-15 oscillator delivers soliton pulses with a duration of 200 fs and at a repetition rate of 216 MHz (1/6 of the master clock). This would be also used by various laser and detector diagnostics inside the experiment area. The current oscillator will therefore be replaced by a piezo-adjustable oscillator available at the Queen's University of Belfast. Each of these fs pulses contains an energy of a few nJ. A 10 Hz pulse-train is selected and and amplified to about 0.5 mJ in the booster. This part of the system is known as the front-end. 

\item \textbf{Optical pulse stretcher}\newline
Following the front end, the pulses are sent into a grating-based pulse stretcher.  There they are steered to hit an all-reflective grating four times.  The stretcher band-pass is set to about 100\,nm to avoid clipping effects that would adversely affect the pulse shape. 
\item \textbf{Multi-pass 10\,Hz Ti:Sapphire power amplifier}\newline  
Following the stretcher the pulses are amplified in a regenerative amplifier with a TEM$_{00}$ spatial mode and amplified in three amplification stages at 10\,Hz repetition rate allowing for stable operation. Each stage consists of a Ti:Sapphire crystal pumped with ns-duration green (532\,nm) laser pulses. Following each stage, the beam is expanded to remain below the damage threshold of the following optics in the optical chain. After a regenerative amplifier and three multi-pass amplifiers, a compressed output energy of 1.2\,J  can be reached. 
\item \textbf{Optical pulse compressor}\newline    
The fully amplified pulses will be expanded and sent into an optical pulse compressor which operates under vacuum.  The compressor  is based on the standard design of four reflections from two large gold-coated diffraction gratings on glass substrates. This compressor design   limits the practical repetition rate for high intensity beam crossings to 1\,Hz due to thermal effects. At higher repetition rates thermal aberrations affect the performance of the laser and higher repetition rates would require costly and complex additional features such as grating cooling or active compensation of grating aberrations. 

\end{itemize}

The laser clean room environment  has  sufficient space for both the options. This  includes also sufficient space for a subsequent installation of a further amplifier and upgrade to 350 TW and required transport beamline. This will enable LUXE to explore peak intensities of $1.2 \cdot 10^{21}$\,Wcm$^{-2}$, so that data well into the non-linear regime can be obtained at fields significantly exceeding the Schwinger limit  ($\chi_{\mathrm max}=3.8-4.7$).

\subsection{Installation Considerations}

It has to be disassembled and transported to the Osdorfer Born. The installation has to be start from the beginning. We outline the major steps involved in the assembly and to have an operational laser system. 
\begin{itemize}
    \item During the deinstallation process in Jena all details will be recorded with current data achieved.
    \item     First, three large optical tables (4 m x1.5 m each, $\sim 1$ Ton weight) will be installed. 
    \item The module has to be placed on the table according to their architecture at Jena. Here, all the control systems, devices etc will be placed mostly on a roof above the tables. The required electrical connections to all components have to be finalised. 
    \item The laser safety interlock will be implemented on the laser front end (for example, accidental tripping of the laser area doors will shutdown the power of oscillator ensuring no seed available)
    \item In parallel the power connection, water arrangement for the power supplies of the pump lasers will be performed in the service room. 
    \item The alignment of the laser front end will take place. 
    \item The pump laser will be placed at their positions. A full optical alignment will be performed before running them at full energy.
    \item The time synchronisation of pump lasers and laser pulse for the amplification will be performed.
    \item The delay stages and attenuator has to be implemented after the main amplification stage.
    \item The laser beam will be coupled in the compressor. The alignment of the compressor and pulse compression will be carried out.
    
\end{itemize}

\,%begin{table}[]
