# Supplementary material for: Technical Design Report for the LUXE Experiment
Source: arXiv:2308.00515 source file (2023-08-02)
Supplement: Supplementary file 4 [file appendix.tex]

\section{The ECAL plan for the installation}
%Can have appendices here, e.g. for very technical information that would disrupt the flow of the main note.
\Large

\vspace{1cm}
{\bf{Locations:}}

\vspace{.5cm}
\normalsize
\begin{itemize}
    \item Experimental Area (EA)
    \item Control Room (CR)
\end{itemize}
\vspace{.5cm}
\Large
{\bf{List of components to be installed:}}
\normalsize
\vspace{.5cm}
\begin{itemize}
    \item ECAL detector, including FE PCBs
    \item HV and LV power supply
    \item Rack with crates
    \item FPGA cards
    \item DAQ Computer with ethernet connection to the rack
\end{itemize}
\vspace{.5cm}
\Large
{\bf{Expected installations prior to the one above:}}
\normalsize
\vspace{.5cm}
\begin{itemize}
      \item The optical table for the tracker and ECAL is available and pre-aligned
      \item Cables for HV and LV between detector table and rack are installed
\end{itemize}
\vspace{.5cm}
The details of the resource loaded schedule are shown in   Fig.~\ref{fig:resource_schedule}.
\begin{figure}[hpbt]
 \begin{center}
 %\hspace*{-0.5cm}
 % \includegraphics[width=1.6\textwidth]{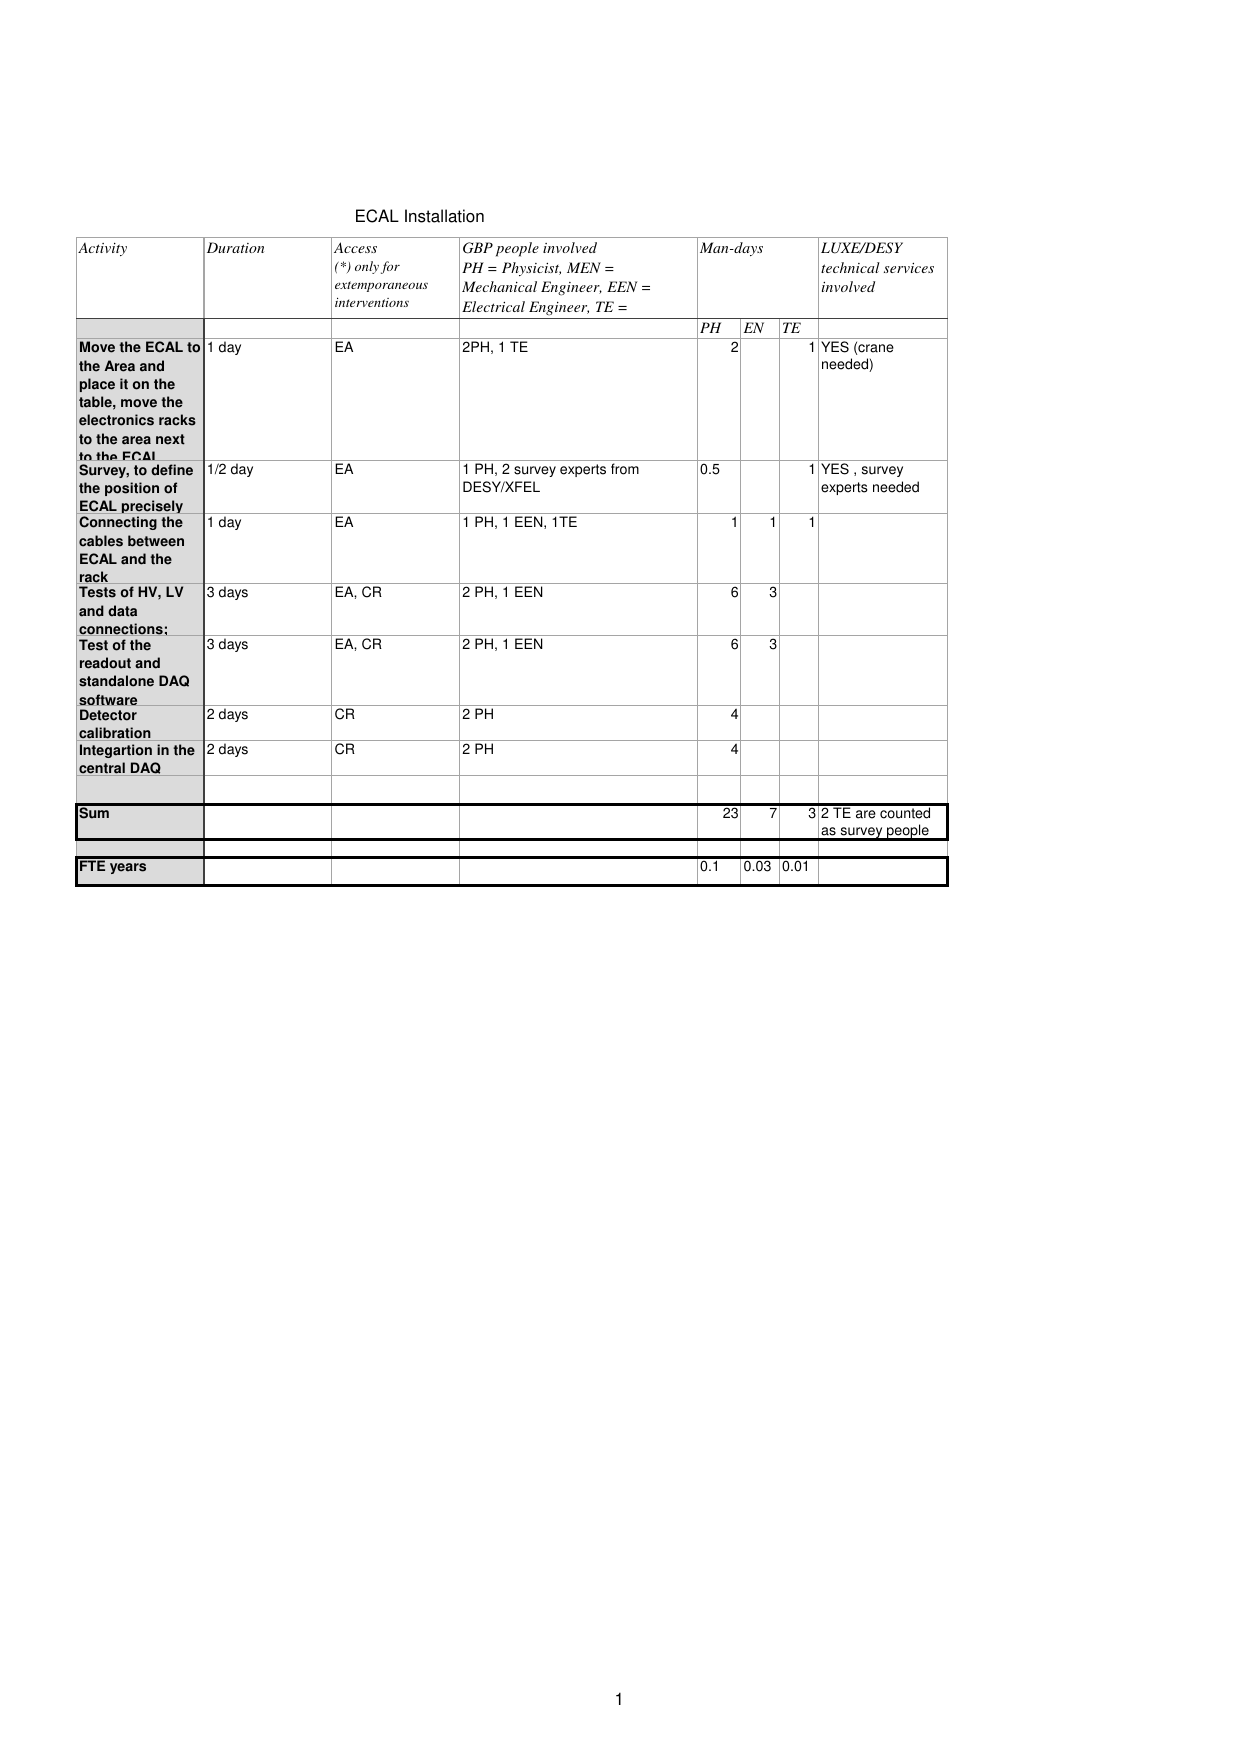}
 \includegraphics[width=1.1\textwidth]{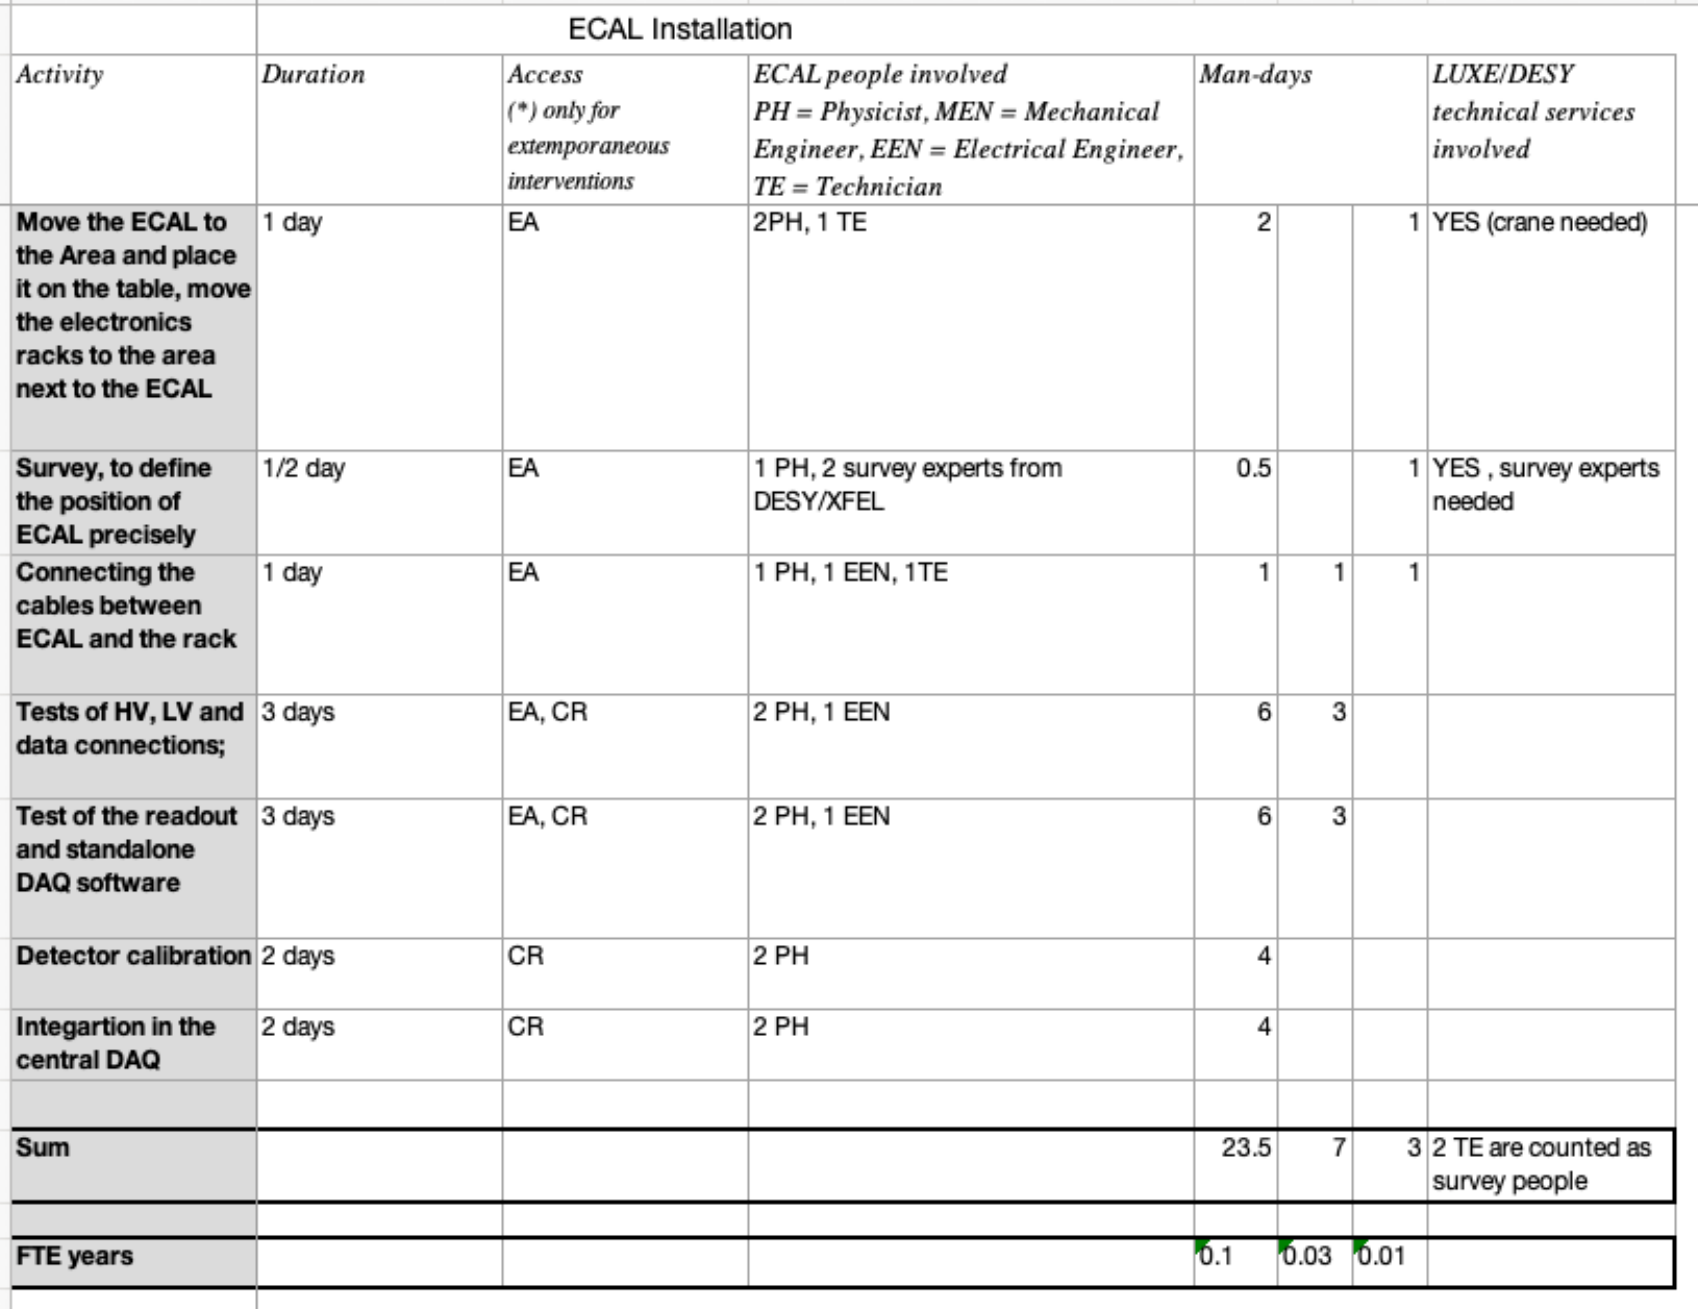}
    \caption{The resource loaded schedule for the installation of the ECAL. EA stands for experimental area and CR means control room.} 
    \label{fig:resource_schedule}
    \end{center}
\end{figure}

\section{Changes since the CDR}
Silicon sensors of $89.9 \times 89.9 \units {mm^2}$, corresponding to $16 \times 16$ pads, as produced by Hamamatsu Photonics for the CALICE Collaboration,
will be used. These sensors are higher than needed, $89.9 \units {mm}$ instead of about $50 \units {mm}$. However, since no new masks have to be produced, and the order will be done together with ECAL-E sensors, total costs will be less.
\clearpage
%\section{Title of Appendix C}
\section{Quality Factor}
\label{sec:QualityFactor}
\begin{table}[htp]
    \centering
        \caption{The list of  quality factors required for quantification of the level of confidence in a price estimate.}
   \begin{tabular}{p{1.5cm}|p{9.5cm}}
QF1 &
Off-the-shelf Items for which there is a recent ($< 1 $ year) catalog price or quote with more than one potential supplier
Items that are a copy or almost identical to an existing design for which there is a recent ($< 1 $ year) catalog price or quote with more than one potential supplier.\\\hline
QF2&
Items falling short of satisfying a single QF1 criterium, e.g.:
- only one potential vendor;
- estimate based on not completed design or design with minor modifications; - quotes $> 1$ year but still sufficiently reliable based on experience.\\\hline
QF3&
Items with quotes $> 2 $ years
Items whose cost estimates are based on a conceptual design or adapted from existing design with extensive modifications
Items whose costs are estimated using physicist or engineering experience regardless of the maturity of the design.\\\hline
QF4&
Items that have unproven fabrication yields or for which there are unique issues e.g. a special- order item and/or a single preferred supplier.\\\hline
QF5&
Items that are still in a conceptual stage with no detailed specifications or design.\\\hline

    \end{tabular}
    \label{tab:qf}
\end{table}
