# Supplementary material for: Technical Design Report for the LUXE Experiment
Source: arXiv:2308.00515 source file (2023-08-02)
Supplement: Supplementary file 6 [file appendix.tex]

\subsection*{Responsibilities required for each of the different work-package}

In the following tables the groups identified for each of the items required in the construction of the experiment are shown. The estimates presented here and also in Section~\ref{sec:ressources} still require further confirmations with each working groups.
\label{sec:Appendix:responsibilities}
\begin{landscape}% Landscape page
\begin{table}[]
\tiny
\begin{tabular}{|p{0.1\linewidth}|p{0.1\linewidth}|p{0.07\linewidth}|p{0.015\linewidth}|p{0.02\linewidth}|p{0.02\linewidth}|p{0.02\linewidth}|p{0.02\linewidth}|p{0.02\linewidth}|p{0.02\linewidth}|p{0.02\linewidth}|p{0.02\linewidth}|p{0.02\linewidth}|p{0.015\linewidth}|p{0.015\linewidth}|p{0.015\linewidth}|p{0.015\linewidth}|p{0.015\linewidth}|p{0.015\linewidth}|p{0.015\linewidth}|p{0.02\linewidth}|p{0.02\linewidth}|p{0.04\linewidth}|}
\hline

Workpackage & Item &  & FH & MEA & ZBAU & MDI & MVS & MCS & MSK & MPS & MPC & MKK & D3 & D5 & IT & IPP & MR & ZM3 & ZM5 & \euxfel Company & External company & Other institute\\ 
\multirow{19}{*}{\shortstack[l]{1) Electron beam \\line}} &  &  &  &  &  &  &  &  &  &  &  &  &  &  &  &  &  &  &  &  &  & \\ 
\hline
\cline{2-23}

 & \multirow{3}{*}{\shortstack[l]{Beampipe Apertures\\ and transition}} & Design & Or & Or &  &  & And &  &  &  &  &  &  &  &  &  &  &  &  &  &  & \\ 
 &  & Construction &  &  &  &  &  &  &  &  &  &  &  &  &  &  &  & Or &  &  & Or & \\ 
 &  & Installation & Or & Or &  &  & And &  &  &  &  &  &  &  &  &  &  &  &  &  &  & \\ 
\cline{2-23}

 & \multirow{3}{*}{\shortstack[l]{Beamline support \\and vibration}} & Design & Or & Or &  &  &  &  &  &  &  &  &  &  &  &  &  &  &  &  &  & \\ 
 &  & Construction &  & And &  &  &  &  &  &  &  &  &  &  &  &  &  & Or & Or &  & Or & \\ 
 &  & Installation & Or & Or &  &  &  &  &  &  &  &  &  &  &  &  &  &  &  &  &  & \\ 
\cline{2-23}

 & \multirow{3}{*}{\shortstack[l]{Alignment and Survey}} & Design & And & And &  &  &  &  &  &  &  &  &  &  &  &  &  &  &  &  &  & \\ 
 &  & Construction &  & And &  &  &  &  &  &  &  &  &  &  &  &  &  &  &  &  &  & \\ 
 &  & Installation & And & And &  &  &  &  &  &  &  &  &  &  &  &  &  &  &  &  &  & \\ 
\cline{2-23}

 & \multirow{3}{*}{\shortstack[l]{Transport}} & Design & Or & Or &  &  &  &  &  &  &  &  &  &  &  &  &  &  &  &  &  & \\ 
 &  & Construction &  & And &  &  &  &  &  &  &  &  &  &  &  &  &  &  &  & And &  & \\ 
 &  & Installation & Or & Or &  &  &  &  &  &  &  &  &  &  &  &  &  &  &  & And &  & \\ 
\cline{2-23}

 & \multirow{3}{*}{\shortstack[l]{Beam monitors}} & Design &  &  &  & And &  &  &  &  &  &  &  &  &  &  &  &  &  &  &  & \\ 
 &  & Construction &  &  &  & Or &  &  &  &  &  &  &  &  &  &  &  &  &  &  & Or & \\ 
 &  & Installation &  & And &  & And & And &  &  &  &  &  &  &  &  &  &  &  &  &  &  & \\ 
\cline{2-23}

 & \multirow{3}{*}{\shortstack[l]{Beam controls / ctrl\\ system and timing}} & Design &  &  &  &  &  & And & And & And &  &  &  &  &  &  &  &  &  &  &  & \\ 
 &  & Construction &  &  &  &  &  & And & And & And &  &  &  &  &  &  &  &  &  &  &  & \\ 
 &  & Installation &  &  &  &  &  & And & And & And &  &  &  &  &  &  &  &  &  &  &  & \\ 
%  &  &  &  &  &  &  &  &  &  &  &  &  &  &  &  &  &  &  &  &  &  & \\ 

\multirow{19}{*}{\shortstack[l]{2) Beam dumps}} &  &  &  &  &  &  &  &  &  &  &  &  &  &  &  &  &  &  &  &  &  & \\ 
\hline

 & \multirow{3}{*}{\shortstack[l]{Electron-laser \\ electron dump}} & Design & And &  &  &  &  &  &  &  &  &  & And &  &  &  &  &  &  &  &  & Dubna\\ 
 &  & Construction &  &  &  &  &  &  &  &  &  &  &  &  &  &  &  &  &  &  &  & Dubna\\ 
 &  & Installation & Or & Or &  &  &  &  &  &  &  &  & And &  &  &  &  &  &  &  &  & \\ 
 \cline{2-23}

 & \multirow{3}{*}{\shortstack[l]{Gamma-laser \\ electron dump}} & Design & And &  &  &  &  &  &  &  &  &  & And &  &  &  &  &  &  &  &  & Dubna\\ 
 &  & Construction &  &  &  &  &  &  &  &  &  &  &  &  &  &  &  &  &  &  &  & Dubna\\ 
 &  & Installation & Or & Or &  &  &  &  &  &  &  &  & And &  &  &  &  &  &  &  &  & \\ 
 \cline{2-23}

 & \multirow{3}{*}{\shortstack[l]{Final photon dump}} & Design & And &  &  &  &  &  &  &  &  &  & And &  &  &  &  &  &  &  &  & Dubna\\ 
 &  & Construction &  &  &  &  &  &  &  &  &  &  &  &  &  &  &  &  &  &  &  & Dubna\\ 
 &  & Installation & Or & Or &  &  &  &  &  &  &  &  & And &  &  &  &  &  &  &  &  & \\ 
 \cline{2-23}

 & \multirow{3}{*}{\shortstack[l]{Shielding}} & Design & Or & Or &  &  &  &  &  &  &  &  &  &  &  &  &  &  &  &  &  & Dubna\\ 
 &  & Construction & Or & Or &  &  &  &  &  &  &  &  & And &  &  &  &  &  &  &  & And & \\ 
 &  & Installation & Or & Or &  &  &  &  &  &  &  &  & And &  &  &  &  &  &  &  & And & \\ 
 \cline{2-23}

 & \multirow{3}{*}{\shortstack[l]{Monitoring}} & Design & And & And &  &  &  &  &  &  &  &  & And &  &  &  &  &  &  &  &  & \\ 
 &  & Construction & And &  &  &  &  &  &  &  &  &  & And & And  &  &  &  &  &  &  &  & \\ 
 &  & Installation & And &  &  &  &  &  &  &  &  &  & And & And &  &  &  &  &  &  &  & \\ 
 \cline{2-23}

 & \multirow{3}{*}{\shortstack[l]{Services}} & Design & And &  &  &  &  &  &  &  &  & And &  &  &  &  &  &  &  &  &  & \\ 
 &  & Construction & And &  &  &  &  &  &  &  &  & And &  &  &  &  &  &  &  &  &  & \\ 
 &  & Installation & And &  &  &  &  &  &  &  &  & And &  &  &  &  &  &  &  &  &  & \\ 
 \cline{2-23}

 & \multirow{3}{*}{\shortstack[l]{Transport}} & Design & Or & Or & And &  &  &  &  &  &  &  &  &  &  &  &  &  &  &  &  & \\ 
 &  & Construction &  &  &  &  &  &  &  &  &  &  &  &  &  &  &  &  &  &  &  & \\ 
 &  & Installation & Or & Or & And &  &  &  &  &  &  &  &  &  &  &  &  &  &  &  &  & \\ 
 &  &  &  &  &  &  &  &  &  &  &  &  &  &  &  &  &  &  &  &  &  & \\ 
 
 \hline

\hline
\end{tabular}
\caption{Identified responsibilities for the different items required by the LUXE experiment, for the design, construction and installation. When a group is needed it is assigned with "And". If two groups can achieve the same task they are assigned and "Or".}
% \label{TC:Annex:Resources_WP65}
\end{table}
\end{landscape}% Landscape page

\begin{landscape}% Landscape page
\begin{table}[]
\tiny
\begin{tabular}{|p{0.1\linewidth}|p{0.1\linewidth}|p{0.07\linewidth}|p{0.015\linewidth}|p{0.02\linewidth}|p{0.02\linewidth}|p{0.02\linewidth}|p{0.02\linewidth}|p{0.02\linewidth}|p{0.02\linewidth}|p{0.02\linewidth}|p{0.02\linewidth}|p{0.02\linewidth}|p{0.015\linewidth}|p{0.015\linewidth}|p{0.015\linewidth}|p{0.015\linewidth}|p{0.015\linewidth}|p{0.015\linewidth}|p{0.015\linewidth}|p{0.02\linewidth}|p{0.02\linewidth}|p{0.04\linewidth}|}
\hline

Workpackage & Item &  & FH & MEA & ZBAU & MDI & MVS & MCS & MSK & MPS & MPC & MKK & D3 & D5 & IT & IPP & MR & ZM3 & ZM5 & \euxfel Company & External company & Other institute\\
\multirow{7}{*}{\shortstack[l]{3) Experiment \\magnets}} &  &  &  &  &  &  &  &  &  &  &  &  &  &  &  &  &  &  &  &  &  & \\ 
\hline
\cline{2-23}
 &\multirow{3}{*}{\shortstack[l]{Procurement tests \\and measurements}} & Design &  & And &  &  &  &  &  &  &  &  &  &  &  &  &  &  &  &  &  & \\ 
 &  & Construction &  & And &  &  &  &  &  &  &  &  &  &  &  &  &  &  &  &  &  & \\ 
 &  & Installation &  & And &  &  &  &  &  &  &  &  &  &  &  &  &  &  &  &  &  & \\ 
 \cline{2-23}

 &\multirow{3}{*}{\shortstack[l]{Power network}} & Design &  &  &  &  &  &  &  &  &  & And &  &  &  &  &  &  &  &  &  & \\ 
 &  & Construction &  &  &  &  &  &  &  &  &  & And &  &  &  &  &  &  &  &  &  & \\ 
 &  & Installation &  &  &  &  &  &  &  &  &  & And &  &  &  &  &  &  &  &  &  & \\ 
  \cline{2-23}

 &\multirow{3}{*}{\shortstack[l]{Power supplies}} & Design &  &  &  &  &  &  &  &  & And &  &  &  &  &  &  &  &  &  &  & \\ 
 &  & Construction &  &  &  &  &  &  &  &  &  & And &  &  &  &  &  &  &  &  &  & \\ 
 &  & Installation &  &  &  &  &  &  &  &  &  & And &  &  &  &  &  &  &  &  &  & \\ 
  \cline{2-23}
 &\multirow{3}{*}{\shortstack[l]{Cooling}} & Design &  &  &  &  &  &  &  &  & And &  &  &  &  &  &  &  &  &  &  & \\ 
 &  & Construction &  &  &  &  &  &  &  &  &  & And &  &  &  &  &  &  &  &  &  & \\ 
 &  & Installation &  &  &  &  &  &  &  &  &  & And &  &  &  &  &  &  &  &  &  & \\ 
  \cline{2-23}

 &\multirow{3}{*}{\shortstack[l]{Cabling}} & Design &  &  &  &  &  &  &  &  & And &  &  &  &  &  &  &  &  &  &  & \\ 
 &  & Construction &  &  &  &  &  &  &  &  & And &  &  &  &  &  &  &  &  &  &  & \\ 
 &  & Installation &  &  &  &  &  &  &  &  & And &  &  &  &  &  &  &  &  &  &  & \\ 
  \cline{2-23}

 &\multirow{3}{*}{\shortstack[l]{Vacuum chambers\\ and Exit windows}} & Design &  &  &  &  & And &  &  &  &  &  &  &  &  &  &  &  &  &  &  & Weizmann\\ 
 &  & Construction &  &  &  &  & And &  &  &  &  &  &  &  &  &  &  &  &  &  &  & Weizmann\\ 
 &  & Installation & And & And &  &  & And &  &  &  &  &  &  &  &  &  &  &  &  &  &  & \\ 
  \cline{2-23}

 &\multirow{3}{*}{\shortstack[l]{Survey and positions}} & Design & And & And &  &  &  &  &  &  &  &  &  &  &  &  &  &  &  &  &  & \\ 
 &  & Construction &  &  &  &  &  &  &  &  &  &  &  &  &  &  &  &  &  &  &  & \\ 
 &  & Installation & And & And &  &  &  &  &  &  &  &  &  &  &  &  &  &  &  &  &  & \\ 
 &  &  &  &  &  &  &  &  &  &  &  &  &  &  &  &  &  &  &  &  &  & \\ 
  \cline{2-23}

 \hline

\hline
\end{tabular}
\caption{Identified responsibilities for the different items required by the LUXE experiment, for the design, construction and installation. When a group is needed it is assigned with "And". If two groups can achieve the same task they are assigned and "Or".}
% \label{TC:Annex:Resources_WP65}
\end{table}
\end{landscape}% Landscape page

\begin{landscape}% Landscape page
\begin{table}[]
\tiny
\begin{tabular}{|p{0.1\linewidth}|p{0.1\linewidth}|p{0.07\linewidth}|p{0.015\linewidth}|p{0.02\linewidth}|p{0.02\linewidth}|p{0.02\linewidth}|p{0.02\linewidth}|p{0.02\linewidth}|p{0.02\linewidth}|p{0.02\linewidth}|p{0.02\linewidth}|p{0.02\linewidth}|p{0.015\linewidth}|p{0.015\linewidth}|p{0.015\linewidth}|p{0.015\linewidth}|p{0.015\linewidth}|p{0.015\linewidth}|p{0.015\linewidth}|p{0.02\linewidth}|p{0.02\linewidth}|p{0.04\linewidth}|}
\hline

Workpackage & Item &  & FH & MEA & ZBAU & MDI & MVS & MCS & MSK & MPS & MPC & MKK & D3 & D5 & IT & IPP & MR & ZM3 & ZM5 & \euxfel Company & External company & Other institute\\
% \hline
% \multirow{19}{*}{\shortstack[l]{1) Electron beam \\line}} &  &  &  &  &  &  &  &  &  &  &  &  &  &  &  &  &  &  &  &  &  & \\ 
% \hline
% \cline{2-23}

%  & \multirow{3}{*}{\shortstack[l]{Beampipe Apertur\\ and transition}} & Design & Or & Or &  &  & And &  &  &  &  &  &  &  &  &  &  &  &  &  &  & \\ 
%  &  & Construction &  &  &  &  &  &  &  &  &  &  &  &  &  &  &  & Or &  &  & Or & \\ 
%  &  & Installation & Or & Or &  &  & And &  &  &  &  &  &  &  &  &  &  &  &  &  &  & \\ 
% \cline{2-23}
\multirow{12}{*}{\shortstack[l]{4) Technical \\infrastructure\\ UG03}} &  &  &  &  &  &  &  &  &  &  &  &  &  &  &  &  &  &  &  &  &  & \\ 
\hline
\cline{2-23}
 &\multirow{3}{*}{\shortstack[l]{Power network}} & Design &  &  &  &  &  & And &  &  & And & And &  &  &  &  &  &  &  &  &  & \\ 
 &  & Construction &  &  &  &  &  & And &  &  & And & And &  &  &  &  &  &  &  &  &  & \\ 
 &  & Installation &  &  &  &  &  & And &  &  & And & And &  &  &  &  &  &  &  &  &  & \\ 
 \cline{2-23}
 & Air conditioning & Design &  &  &  &  &  & And &  &  &  & And &  &  &  &  &  &  &  &  &  & \\ 
 &  & Construction &  &  &  &  &  & And &  &  &  & And &  &  &  &  &  &  &  &  &  & \\ 
 &  & Installation &  &  &  &  &  & And &  &  &  & And &  &  &  &  &  &  &  &  &  & \\ 
  \cline{2-23}

 & \multirow{3}{*}{\shortstack[l]{Liquids and\\ gas supply}} & Design &  & And &  &  &  & And &  &  &  &  &  &  &  &  &  &  &  &  &  & \\ 
 &  & Construction &  & And &  &  &  & And &  &  &  &  &  &  &  &  &  &  &  &  & And & \\ 
 &  & Installation &  & And &  &  &  & And &  &  &  &  &  &  &  &  &  &  &  &  & And & \\ 
  \cline{2-23}

 & \multirow{3}{*}{\shortstack[l]{Cabling (detector \\signal+beam \\monitoring)}} & Design & And &  &  & And &  &  &  &  &  &  &  &  &  &  &  &  &  &  & And & \\ 
 &  & Construction &  &  &  &  &  &  &  &  &  &  &  &  &  &  &  &  &  & And & And & \\ 
 &  & Installation &  &  &  &  &  &  &  &  &  &  &  &  &  &  &  &  &  & And & And & \\ 
  \cline{2-23}

 & \multirow{3}{*}{\shortstack[l]{Cable tray}} & Design &  &  &  & And &  &  &  &  &  &  &  &  &  &  &  &  &  & And & And & \\ 
 &  & Construction &  &  &  & And &  &  &  &  &  &  &  &  &  &  &  &  &  & And & And & \\ 
 &  & Installation &  &  &  & And &  &  &  &  &  &  &  &  &  &  &  &  &  & And & And & \\ 
  \cline{2-23}

 & \multirow{3}{*}{\shortstack[l]{Networking}} & Design &  &  &  & And &  &  &  &  &  &  &  &  & And &  &  &  &  &  &  & \\ 
 &  & Construction &  &  &  & And &  &  &  &  &  &  &  &  & And &  &  &  &  &  &  & \\ 
 &  & Installation &  &  &  & And &  &  &  &  &  &  &  &  &  &  &  &  &  &  & And & \\ 
  \cline{2-23}

 & \multirow{3}{*}{\shortstack[l]{Front-end racks}} & Design & And &  &  & And & And &  & And &  &  &  &  &  &  &  &  &  &  &  &  & \\ 
 &  & Construction & And &  &  & And & And &  & And &  &  &  &  &  &  &  &  &  &  &  &  & \\ 
 &  & Installation & And &  &  & And & And &  & And &  &  &  &  &  &  &  &  &  &  &  &  & \\ 
  \cline{2-23}

 & \multirow{3}{*}{\shortstack[l]{Detector movable \\structure}} & Design & And &  &  &  &  &  &  &  &  &  &  &  &  &  &  &  &  &  &  & \\ 
 &  & Construction &  &  &  &  &  &  &  &  &  &  &  &  &  &  &  &  &  &  & And & \\ 
 &  & Installation & And &  &  &  &  &  &  &  &  &  &  &  &  &  &  &  &  &  &  & \\ 
  \cline{2-23}

 & \multirow{3}{*}{\shortstack[l]{Detector support \\structure}} & Design & And &  &  &  &  &  &  &  &  &  &  &  &  &  &  &  &  &  &  & \\ 
 &  & Construction & And &  &  &  &  &  &  &  &  &  &  &  &  &  &  &  &  &  &  & \\ 
 &  & Installation & And &  &  &  &  &  &  &  &  &  &  &  &  &  &  &  &  &  &  & \\ 
  \cline{2-23}

 & \multirow{3}{*}{\shortstack[l]{Positioning and \\survey}} & Design & And & And &  &  &  &  &  &  &  &  &  &  &  &  &  &  &  &  &  & \\ 
 &  & Construction &  &  &  &  &  &  &  &  &  &  &  &  &  &  &  &  &  &  &  & \\ 
 &  & Installation & And & And &  &  &  &  &  &  &  &  &  &  &  &  &  &  &  &  &  & \\ 
  \cline{2-23}

 & \multirow{3}{*}{\shortstack[l]{Environment \\monitoring \\(temp and  hum..)}} & Design &  &  &  &  &  &  &  &  &  & And &  &  &  &  &  &  &  &  &  & \\ 
 &  & Construction &  &  &  &  &  &  &  &  &  & And &  &  &  &  &  &  &  &  &  & \\ 
 &  & Installation &  &  &  &  &  &  &  &  &  & And &  &  &  &  &  &  &  &  &  & \\ 
  \cline{2-23}

 & \multirow{3}{*}{\shortstack[l]{Development of \\integration concept}} & Design & And & And &  &  &  &  &  &  &  &  &  &  &  & And &  &  &  &  &  & \\ 
 &  & Construction &  &  &  &  &  &  &  &  &  &  &  &  &  &  &  &  &  &  &  & \\ 
 &  & Installation &  &  &  &  &  &  &  &  &  &  &  &  &  &  &  &  &  &  &  & \\ 
 &  &  &  &  &  &  &  &  &  &  &  &  &  &  &  &  &  &  &  &  &  & \\ 
 
 \hline

\hline
\end{tabular}
\caption{Identified responsibilities for the different items required by the LUXE experiment, for the design, construction and installation. When a group is needed it is assigned with "And". If two groups can achieve the same task they are assigned and "Or".}
% \label{TC:Annex:Resources_WP65}
\end{table}
\end{landscape}% Landscape page

\begin{landscape}% Landscape page
\begin{table}[]
\tiny
\begin{tabular}{|p{0.1\linewidth}|p{0.1\linewidth}|p{0.07\linewidth}|p{0.015\linewidth}|p{0.02\linewidth}|p{0.02\linewidth}|p{0.02\linewidth}|p{0.02\linewidth}|p{0.02\linewidth}|p{0.02\linewidth}|p{0.02\linewidth}|p{0.02\linewidth}|p{0.02\linewidth}|p{0.015\linewidth}|p{0.015\linewidth}|p{0.015\linewidth}|p{0.015\linewidth}|p{0.015\linewidth}|p{0.015\linewidth}|p{0.015\linewidth}|p{0.02\linewidth}|p{0.02\linewidth}|p{0.04\linewidth}|}
\hline

Workpackage & Item &  & FH & MEA & ZBAU & MDI & MVS & MCS & MSK & MPS & MPC & MKK & D3 & D5 & IT & IPP & MR & ZM3 & ZM5 & \euxfel Company & External company & Other institute\\

\multirow{10}{*}{\shortstack[l]{5) Surface building \\(include service \\and control room ) }} &  &  &  &  &  &  &  &  &  &  &  &  &  &  &  &  &  &  &  &  &  & \\ 
\hline
\cline{2-23}
 &\multirow{3}{*}{\shortstack[l]{Building }} & Design & And &  &  &  &  &  &  &  &  &  &  &  &  &  &  &  &  &  And &  And & \\ 
 &  & Construction &  &  &  &  &  &  &  &  &  &  &  &  &  &  &  &  &  &  And &  And & \\ 
 &  & Installation &  &  &  &  &  &  &  &  &  &  &  &  &  &  &  &  &  &  &  & \\ 
\cline{2-23}
 &\multirow{3}{*}{\shortstack[l]{Power network}} & Design &  &  &  &  &  & And &  &  & And & And &  &  &  &  &  &  &  &  &  & \\ 
 &  & Construction &  &  &  &  &  & And &  &  & And & And &  &  &  &  &  &  &  &  &  & \\ 
 &  & Installation &  &  &  &  &  & And &  &  & And & And &  &  &  &  &  &  &  &  &  & \\ 
 \cline{2-23}
 & Air conditioning & Design &  &  &  &  &  & And &  &  &  & And &  &  &  &  &  &  &  &  &  & \\ 
 &  & Construction &  &  &  &  &  & And &  &  &  & And &  &  &  &  &  &  &  &  &  & \\ 
 &  & Installation &  &  &  &  &  & And &  &  &  & And &  &  &  &  &  &  &  &  &  & \\ 
 \cline{2-23}

 & \multirow{3}{*}{\shortstack[l]{Liquids and\\ gas supply}} & Design &  & And &  &  &  & And &  &  &  &  &  &  &  &  &  &  &  &  &  & \\ 
 &  & Construction &  & And &  &  &  & And &  &  &  &  &  &  &  &  &  &  &  &  & And & \\ 
 &  & Installation &  & And &  &  &  & And &  &  &  &  &  &  &  &  &  &  &  &  & And & \\ 
  \cline{2-23}

 & \multirow{3}{*}{\shortstack[l]{Cabling}} & Design & And &  &  & And &  &  &  &  &  &  &  &  &  &  &  &  &  &  & And & \\ 
 &  & Construction &  &  &  &  &  &  &  &  &  &  &  &  &  &  &  &  &  & And & And & \\ 
 &  & Installation &  &  &  &  &  &  &  &  &  &  &  &  &  &  &  &  &  & And & And & \\ 
  \cline{2-23}

 & \multirow{3}{*}{\shortstack[l]{Cable tray}} & Design &  &  &  & And &  &  &  &  &  &  &  &  &  &  &  &  &  & And & And & \\ 
 &  & Construction &  &  &  & And &  &  &  &  &  &  &  &  &  &  &  &  &  & And & And & \\ 
 &  & Installation &  &  &  & And &  &  &  &  &  &  &  &  &  &  &  &  &  & And & And & \\ 
  \cline{2-23}

 & \multirow{3}{*}{\shortstack[l]{Networking}} & Design &  &  &  & And &  &  &  &  &  &  &  &  & And &  &  &  &  &  &  & \\ 
 &  & Construction &  &  &  & And &  &  &  &  &  &  &  &  & And &  &  &  &  &  &  & \\ 
 &  & Installation &  &  &  & And &  &  &  &  &  &  &  &  &  &  &  &  &  &  & And & \\ 
  \cline{2-23}

 & \multirow{3}{*}{\shortstack[l]{Front-end racks}} & Design & And &  &  &  &  &  &  &  &  &  &  &  &  &  &  &  &  &  &  & \\ 
 &  & Construction & And &  &  &  &  &  &  &  &  &  &  &  &  &  &  &  &  &  &  & \\ 
 &  & Installation & And &  &  &  &  &  &  &  &  &  &  &  &  &  &  &  &  &  &  & \\ 
  \cline{2-23}
 & \multirow{3}{*}{\shortstack[l]{Environment \\monitoring \\(temp and  hum..)}} & Design &  &  &  &  &  &  &  &  &  & And &  &  &  &  &  &  &  &  &  & \\ 
 &  & Construction &  &  &  &  &  &  &  &  &  & And &  &  &  &  &  &  &  &  &  & \\ 
 &  & Installation &  &  &  &  &  &  &  &  &  & And &  &  &  &  &  &  &  &  &  & \\ 
  \cline{2-23}

 & \multirow{3}{*}{\shortstack[l]{Development of \\integration concept}} & Design & And & And &  &  &  &  &  &  &  &  &  &  &  & And &  &  &  &  &  & \\ 
 &  & Construction &  &  &  &  &  &  &  &  &  &  &  &  &  &  &  &  &  &  &  & \\ 
 &  & Installation &  &  &  &  &  &  &  &  &  &  &  &  &  &  &  &  &  &  &  & \\ 
 &  &  &  &  &  &  &  &  &  &  &  &  &  &  &  &  &  &  &  &  &  & \\ 

 \hline

\hline
\end{tabular}
\caption{Identified responsibilities for the different items required by the LUXE experiment, for the design, construction and installation. When a group is needed it is assigned with "And". If two groups can achieve the same task they are assigned and "Or".}
% \label{TC:Annex:Resources_WP65}
\end{table}
\end{landscape}% Landscape page

\begin{landscape}% Landscape page
\begin{table}[]
\tiny
\begin{tabular}{|p{0.1\linewidth}|p{0.1\linewidth}|p{0.07\linewidth}|p{0.015\linewidth}|p{0.02\linewidth}|p{0.02\linewidth}|p{0.02\linewidth}|p{0.02\linewidth}|p{0.02\linewidth}|p{0.02\linewidth}|p{0.02\linewidth}|p{0.02\linewidth}|p{0.02\linewidth}|p{0.015\linewidth}|p{0.015\linewidth}|p{0.015\linewidth}|p{0.015\linewidth}|p{0.015\linewidth}|p{0.015\linewidth}|p{0.015\linewidth}|p{0.02\linewidth}|p{0.02\linewidth}|p{0.04\linewidth}|}
\hline

Workpackage & Item &  & FH & MEA & ZBAU & MDI & MVS & MCS & MSK & MPS & MPC & MKK & D3 & D5 & IT & IPP & MR & ZM3 & ZM5 & \euxfel Company & External company & Other institute\\

\multirow{16}{*}{\shortstack[l]{6) Laser \\infrastructure\\ and beamline}} &  &  &  &  &  &  &  &  &  &  &  &  &  &  &  &  &  &  &  &  &  & \\  

\hline
\cline{2-23}
 &\multirow{3}{*}{\shortstack[l]{Laser clean room}} & Design & And &  &  &  &  &  &  &  &  &  &  &  &  &  &  &  &  &  & And & \\ 
 &  & Construction &  &  &  &  &  &  &  &  &  &  &  &  &  &  &  &  &  &  & And & \\ 
 &  & Installation &  & And &  &  &  &  &  &  &  &  &  &  &  &  &  &  &  &  & And & \\ 
\cline{2-23}
 &\multirow{3}{*}{\shortstack[l]{Laser service room}} & Design & And &  &  &  &  &  &  &  &  &  &  &  &  &  &  &  &  &  & And & \\ 
 &  & Construction &  &  &  &  &  &  &  &  &  &  &  &  &  &  &  &  &  &  & And & \\ 
 &  & Installation &  &  &  &  &  &  &  &  &  &  &  &  &  &  &  &  &  &  & And & \\ 
\cline{2-23}
 &\multirow{3}{*}{\shortstack[l]{Power network}} & Design &  &  &  &  &  & And &  &  & And & And &  &  &  &  &  &  &  &  &  & \\ 
 &  & Construction &  &  &  &  &  & And &  &  & And & And &  &  &  &  &  &  &  &  &  & \\ 
 &  & Installation &  &  &  &  &  & And &  &  & And & And &  &  &  &  &  &  &  &  &  & \\ 
 \cline{2-23}
 & Air conditioning & Design &  &  &  &  &  & And &  &  &  & And &  &  &  &  &  &  &  &  &  & \\ 
 &  & Construction &  &  &  &  &  & And &  &  &  & And &  &  &  &  &  &  &  &  &  & \\ 
 &  & Installation &  &  &  &  &  & And &  &  &  & And &  &  &  &  &  &  &  &  &  & \\ 
  \cline{2-23}
  & \multirow{3}{*}{\shortstack[l]{Liquids and\\ gas supply}} & Design &  & And &  &  &  & And &  &  &  &  &  &  &  &  &  &  &  &  &  & \\ 
 &  & Construction &  & And &  &  &  & And &  &  &  &  &  &  &  &  &  &  &  &  & And & \\ 
 &  & Installation &  & And &  &  &  & And &  &  &  &  &  &  &  &  &  &  &  &  & And & \\ 
  \cline{2-23}

 & \multirow{3}{*}{\shortstack[l]{Cabling}} & Design & And &  &  & And &  &  &  &  &  &  &  &  &  &  &  &  &  &  & And & \\ 
 &  & Construction &  &  &  &  &  &  &  &  &  &  &  &  &  &  &  &  &  & And & And & \\ 
 &  & Installation &  &  &  &  &  &  &  &  &  &  &  &  &  &  &  &  &  & And & And & \\ 
  \cline{2-23}

 & \multirow{3}{*}{\shortstack[l]{Cable tray}} & Design &  &  &  & And &  &  &  &  &  &  &  &  &  &  &  &  &  & And & And & \\ 
 &  & Construction &  &  &  & And &  &  &  &  &  &  &  &  &  &  &  &  &  & And & And & \\ 
 &  & Installation &  &  &  & And &  &  &  &  &  &  &  &  &  &  &  &  &  & And & And & \\ 
  \cline{2-23}

 & \multirow{3}{*}{\shortstack[l]{Networking}} & Design &  &  &  & And &  &  &  &  &  &  &  &  & And &  &  &  &  &  &  & \\ 
 &  & Construction &  &  &  & And &  &  &  &  &  &  &  &  & And &  &  &  &  &  &  & \\ 
 &  & Installation &  &  &  & And &  &  &  &  &  &  &  &  &  &  &  &  &  &  & And & \\ 
  \cline{2-23}

 & \multirow{3}{*}{\shortstack[l]{Front-end racks}} & Design & And &  &  &  &  &  &  &  &  &  &  &  &  &  &  &  &  &  &  & \\ 
 &  & Construction & And &  &  &  &  &  &  &  &  &  &  &  &  &  &  &  &  &  &  & \\ 
 &  & Installation & And &  &  &  &  &  &  &  &  &  &  &  &  &  &  &  &  &  &  & \\ 
  \cline{2-23}
 & \multirow{3}{*}{\shortstack[l]{Environment \\monitoring \\(temp and  hum..)}} & Design &  &  &  &  &  &  &  &  &  & And &  &  &  &  &  &  &  &  &  & \\ 
 &  & Construction &  &  &  &  &  &  &  &  &  & And &  &  &  &  &  &  &  &  &  & \\ 
 &  & Installation &  &  &  &  &  &  &  &  &  & And &  &  &  &  &  &  &  &  &  & \\ 
  \cline{2-23}

 &\multirow{3}{*}{\shortstack[l]{Mirrors structure}} & Design &  &  & And &  &  &  &  &  &  &  &  &  &  &  &  &  &  &  &  & Jena\\ 
 &  & Construction &  &  &  &  &  &  &  &  &  &  &  &  &  &  &  & And &  &  &  & \\ 
 &  & Installation &  & And &  &  &  &  &  &  &  &  &  &  &  &  &  &  &  &  &  & \\ 
\cline{2-23}
 &\multirow{3}{*}{\shortstack[l]{Beampipe and\\  apertures and\\ transition}} & Design &  &  &  &  &  &  &  &  &  &  &  &  &  &  &  &  &  &  &  & Jena\\ 
 &  & Construction &  &  &  &  &  &  &  &  &  &  &  &  &  &  &  & And &  &  &  & \\ 
 &  & Installation &  & And &  &  &  &  &  &  &  &  &  &  &  &  &  &  &  &  &  & \\ 
\cline{2-23}
 &\multirow{3}{*}{\shortstack[l]{Beamline support}} & Design &  &  &  &  &  &  &  &  &  &  &  &  &  &  &  &  &  &  &  & Jena\\ 
 &  & Construction &  &  &  &  &  &  &  &  &  &  &  &  &  &  &  & And &  &  &  & \\ 
 &  & Installation &  & And &  &  &  &  &  &  &  &  &  &  &  &  &  &  &  &  &  & \\ 
\cline{2-23}
 &\multirow{3}{*}{\shortstack[l]{Positioning \\and survey}} & Design & And & And &  &  &  &  &  &  &  &  &  &  &  &  &  &  &  &  &  & Jena\\ 
 &  & Construction &  &  &  &  &  &  &  &  &  &  &  &  &  &  &  &  &  &  &  & \\ 
 &  & Installation & And & And &  &  &  &  &  &  &  &  &  &  &  &  &  &  &  &  &  & \\ 
\cline{2-23}
 &\multirow{3}{*}{\shortstack[l]{Beam monitors}} & Design &  &  &  &  &  &  &  &  &  &  &  &  &  &  &  &  &  &  &  & Jena\\ 
 &  & Construction &  &  &  &  &  &  &  &  &  &  &  &  &  &  &  & And &  &  &  & \\ 
 &  & Installation &  &  &  &  &  &  &  &  &  &  &  &  &  &  &  &  &  &  &  & \\ 
\cline{2-23}
 & \multirow{3}{*}{\shortstack[l]{Development of \\integration concept}} & Design & And & And &  &  &  &  &  &  &  &  &  &  &  & And &  &  &  &  &  & \\ 
 &  & Construction &  &  &  &  &  &  &  &  &  &  &  &  &  &  &  &  &  &  &  & \\ 
 &  & Installation &  &  &  &  &  &  &  &  &  &  &  &  &  &  &  &  &  &  &  & \\ 
 &  &  &  &  &  &  &  &  &  &  &  &  &  &  &  &  &  &  &  &  &  & \\

 \hline

\hline
\end{tabular}
\caption{Identified responsibilities for the different items required by the LUXE experiment, for the design, construction and installation. When a group is needed it is assigned with "And". If two groups can achieve the same task they are assigned and "Or".}
% \label{TC:Annex:Resources_WP65}
\end{table}
\end{landscape}% Landscape page

\begin{landscape}% Landscape page
\begin{table}[]
\tiny
\begin{tabular}{|p{0.1\linewidth}|p{0.1\linewidth}|p{0.07\linewidth}|p{0.015\linewidth}|p{0.02\linewidth}|p{0.02\linewidth}|p{0.02\linewidth}|p{0.02\linewidth}|p{0.02\linewidth}|p{0.02\linewidth}|p{0.02\linewidth}|p{0.02\linewidth}|p{0.02\linewidth}|p{0.015\linewidth}|p{0.015\linewidth}|p{0.015\linewidth}|p{0.015\linewidth}|p{0.015\linewidth}|p{0.015\linewidth}|p{0.015\linewidth}|p{0.02\linewidth}|p{0.02\linewidth}|p{0.04\linewidth}|}
\hline

Workpackage & Item &  & FH & MEA & ZBAU & MDI & MVS & MCS & MSK & MPS & MPC & MKK & D3 & D5 & IT & IPP & MR & ZM3 & ZM5 & \euxfel Company & External company & Other institute\\

\multirow{5}{*}{\shortstack[l]{7) Interaction\\ Chamber}} &  &  &  &  &  &  &  &  &  &  &  &  &  &  &  &  &  &  &  &  &  & \\ 
\hline
\cline{2-23}
 &\multirow{3}{*}{\shortstack[l]{Vacuum system}} & Design & And &  &  &  & And &  &  &  &  &  &  &  &  &  &  &  &  &  &  & \\ 
 &  & Construction &  &  &  &  & And &  &  &  &  &  &  &  &  &  &  &  &  &  & And & \\ 
 &  & Installation & And & And &  &  & And &  &  &  &  &  &  &  &  &  &  &  &  &  &  & \\ 
\cline{2-23}
 &\multirow{3}{*}{\shortstack[l]{Services}} & Design &  & And &  &  &  &  &  &  &  & And &  &  & And &  &  &  &  &  &  & \\ 
 &  & Construction &  & And &  &  &  &  &  &  &  & And &  &  & And &  &  &  &  &  &  & \\ 
 &  & Installation &  & And &  &  &  &  &  &  &  & And &  &  & And &  &  &  &  &  &  & \\ 
\cline{2-23}
 &\multirow{3}{*}{\shortstack[l]{Inner components}} & Design & And &  &  &  &  &  &  &  &  &  &  &  &  &  &  &  &  &  &  & Jena\\ 
 &  & Construction & And &  &  &  &  &  &  &  &  &  &  &  &  &  &  &  &  &  &  & Jena\\ 
 &  & Installation & And &  &  &  &  &  &  &  &  &  &  &  &  &  &  &  &  &  &  & Jena\\ 
\cline{2-23}
 &\multirow{3}{*}{\shortstack[l]{Monitoring}} & Design & And &  &  &  &  &  &  &  &  &  &  &  &  &  &  &  &  &  &  & Jena\\ 
 &  & Construction & And &  &  &  &  &  &  &  &  &  &  &  &  &  &  &  &  &  &  & Jena\\ 
 &  & Installation & And &  &  &  &  &  &  &  &  &  &  &  &  &  &  &  &  &  &  & Jena\\ 
\cline{2-23}
 &\multirow{3}{*}{\shortstack[l]{Positioning \\and survey}} & Design & And & And &  &  &  &  &  &  &  &  &  &  &  &  &  &  &  &  &  & \\ 
 &  & Construction &  &  &  &  &  &  &  &  &  &  &  &  &  &  &  &  &  &  &  & \\ 
 &  & Installation & And & And &  &  &  &  &  &  &  &  &  &  &  &  &  &  &  &  &  & \\ 
\hline
\end{tabular}
\caption{Identified responsibilities for the different items required by the LUXE experiment, for the design, construction and installation. When a group is needed it is assigned with "And". If two groups can achieve the same task they are assigned and "Or".}
% \label{TC:Annex:Resources_WP65}
\end{table}
\end{landscape}% Landscape page

\begin{landscape}% Landscape page
\begin{table}[]
\tiny
\begin{tabular}{|p{0.1\linewidth}|p{0.1\linewidth}|p{0.07\linewidth}|p{0.015\linewidth}|p{0.02\linewidth}|p{0.02\linewidth}|p{0.02\linewidth}|p{0.02\linewidth}|p{0.02\linewidth}|p{0.02\linewidth}|p{0.02\linewidth}|p{0.02\linewidth}|p{0.02\linewidth}|p{0.015\linewidth}|p{0.015\linewidth}|p{0.015\linewidth}|p{0.015\linewidth}|p{0.015\linewidth}|p{0.015\linewidth}|p{0.015\linewidth}|p{0.02\linewidth}|p{0.02\linewidth}|p{0.04\linewidth}|}
\hline

Workpackage & Item &  & FH & MEA & ZBAU & MDI & MVS & MCS & MSK & MPS & MPC & MKK & D3 & D5 & IT & IPP & MR & ZM3 & ZM5 & \euxfel Company & External company & Other institute\\
\multirow{4}{*}{\shortstack[l]{8) Safety }} &  &  &  &  &  &  &  &  &  &  &  &  &  &  &  &  &  &  &  &  &  & \\ 
\hline
\cline{2-23}
 &\multirow{3}{*}{\shortstack[l]{Interlocks}} & Design &  & And &  &  &  &  &  & And &  &  & And &  &  &  & And &  &  &  &  & \\ 
 &  & Construction &  & And &  &  &  &  &  & And &  &  & And &  &  &  & And &  &  &  &  & \\ 
 &  & Installation &  & And &  &  &  &  &  & And &  &  & And &  &  &  & And &  &  &  &  & \\ 
\cline{2-23}
 &\multirow{3}{*}{\shortstack[l]{Radiation \\protection\\ monitoring}} & Design &  &  &  &  &  &  &  &  &  &  & And &  &  &  & And &  &  &  &  & \\ 
 &  & Construction &  &  &  &  &  &  &  &  &  &  & And &  &  &  & And &  &  &  &  & \\ 
 &  & Installation &  &  &  &  &  &  &  &  &  &  & And &  &  &  & And &  &  &  &  & \\ 
\cline{2-23}
 &\multirow{3}{*}{\shortstack[l]{Other safety \\monitorings}} & Design &  &  &  &  &  &  &  &  &  &  &  & And &  &  &  &  &  &  &  & \\ 
 &  & Construction &  &  &  &  &  &  &  &  &  &  &  & And &  &  &  &  &  &  &  & \\ 
 &  & Installation &  &  &  &  &  &  &  &  &  &  &  & And &  &  &  &  &  &  &  & \\ 
\cline{2-23}
 &\multirow{3}{*}{\shortstack[l]{Safety concepts}} & Design &  &  &  &  &  &  &  &  &  &  &  &  &  &  & And &  &  & And &  & \\ 
 &  & Construction &  &  &  &  &  &  &  &  &  &  &  &  &  &  &  &  &  &  &  & \\ 
 &  & Installation &  &  &  &  &  &  &  &  &  &  &  &  &  &  &  &  &  &  &  & \\

\hline
\end{tabular}
\caption{Identified responsibilities for the different items required by the LUXE experiment, for the design, construction and installation. When a group is needed it is assigned with "And". If two groups can achieve the same task they are assigned and "Or".}
% \label{TC:Annex:Resources_WP65}
\end{table}
\end{landscape}% Landscape page

\subsection*{Extra figures}
\label{sec:Appendix:Extrafig}
\begin{figure}[ht]
   \centering
   \includegraphics*[height=8cm]{fig/TechnicalInfrastructure/\euxfelSupport} \hspace{2 cm} 
   \includegraphics*[height=8cm]{fig/TechnicalInfrastructure/\euxfelShieldingBlocksElements}
   
   \caption{CAD drawing of the building elements used in the construction of the experiment, (Top) support structure element, (Bottom) concrete blocks used for shielding.
   \label{fig:LUXE_CAD_SupportAndShieldingElements}}
\end{figure}

%%%%%%%%%%%%%%%%%%%%%%%%%%%%%%%%%%%%%%%%%%%%%%%%%%%%%%%%%%%%
% AL: removed appendix D from chapter 10 and added it here
%%%%%%%%%%%%%%%%%%%%%%%%%%%%%%%%%%%%%%%%%%%%%%%%%%%%%%%%%%%%
\section*{Appendix D: quality factor}

\begin{table}[!h]
    \centering
        \caption{The list of  quality factors required for quantification of the level of confidence in a price estimate.}
        \vspace{0.2cm}
   \begin{tabular}{p{0.8cm}|p{10.5cm}}
QF1 &
Off-the-shelf Items for which there is a recent ($< 1 $ year) catalog price or quote with more than one potential supplier
Items that are a copy or almost identical to an existing design for which there is a recent ($< 1 $ year) catalog price or quote with more than one potential supplier.\\\hline
QF2&
Items falling short of satisfying a single QF1 criterium, e.g.:
- only one potential vendor;
- estimate based on not completed design or design with minor modifications; - quotes $> 1$ year but still sufficiently reliable based on experience.\\\hline
QF3&
Items with quotes $> 2 $ years
Items whose cost estimates are based on a conceptual design or adapted from existing design with extensive modifications
Items whose costs are estimated using physicist or engineering experience regardless of the maturity of the design.\\\hline
QF4&
Items that have unproven fabrication yields or for which there are unique issues e.g. a special- order item and/or a single preferred supplier.\\\hline
QF5&
Items that are still in a conceptual stage with no detailed specifications or design.\\\hline

    \end{tabular}
    \label{tab:qf}
\end{table}
