# Supplementary material for: Technical Design Report for the LUXE Experiment
Source: arXiv:2308.00515 source file (2023-08-02)
Supplement: Supplementary file 7 [file appendix_ProjectManagement.tex]

This chapter contains an overview of the LUXE project management and project organisation. It is organised as follows: Section \ref{}

\section{Project Structure}

The LUXE project structure is defined by its two base project management documents, namely the work breakdown structure (WBS) and the product breakdown structure (PBS). The WBS lists and groups tasks that need to be completed to realize, operate and maintain the LUXE experimental complex. The PBS is a structured list of all components and deliverables of the LUXE experimental complex. Both WBS and PBS are closely linked. Table~\ref{tab:wbs} summarizes the highest level of the LUXE WBS elements. Each WBS element, or work package, is provided with a scoping statement that precisely describes the scope of each task and the desired outcome. Finally, each WBS element is linked to one or several deliverables, i.e. an element of the PBS. For the sake of brevity, the scoping statements and list of deliverables have been omitted \\

\begin{table}
\begin{center}
\begin{tabular}{|c|c|c|}
    \hline
    \textbf{WP \#} & \textbf{Name} & \textbf{Description}\\\hline
    d & d & d\\\hline
\end{tabular}
\label{tab:wbs}
\caption{LUXE WBS highest level elements. }
\end{center}
\end{table}

The WBS is used as basis for all further project management activities and documents. The tasks listed in the WBS enter the schedule and resource estimates, and are linked to the project documentation using a so-called project lifecycle management (PLM) tool.\\

\section{Organisational Structure}

The LUXE organisational structure is summarized in the organigram shown in fig.~\ref{fig:organigram}. 

\begin{figure}
    \centering
    \includegraphics[width=0.75\textwidth]{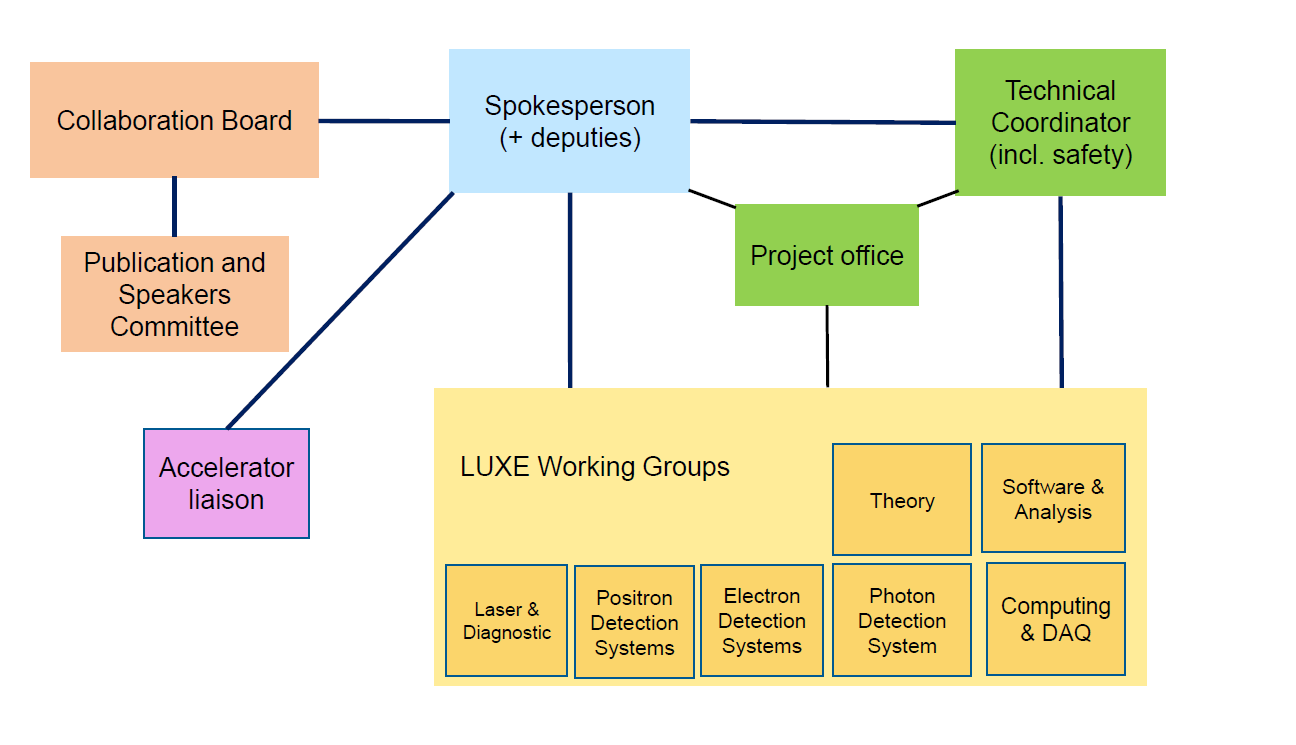}
    \caption{LUXE Organigram.}
    \label{fig:organigram}
\end{figure}

Table~\ref{} summarizes different areas of responsibility for components within the LUXE experimental complex.

\begin{center}
\begin{tabular}{c|c}
    d & d\\
    d & d
\end{tabular}
\end{center}

\section{Resource-Loaded Schedule}

The LUXE project schedule is driven mainly by the design, procurement and production lead times of the major elements in the experimental complex, namely the laser cleanroom surface building and laser system as well as the dipole magnets, beam dumps and interaction vacuum chamber (see fig. \ref{fig:majitemtimeline}). The installation schedule of the LUXE experiment is primarily driven by the \euxfel shutdown schedule, which foresees each year an end-of-year shutdown (duration of order one month) and a short summer shutdown (duration of order two weeks). In addition an extended long shutdown for six months is foreseen in the second half of the year 2025.Preliminary installation works will start in the shorter summer and end-of-year shutdowns in the years leading up to 2025 and the main installation of the long-lead-time major beamline elements and detectors will take place in the long shutdown in 2025.\\

\begin{figure}
    \centering
    \includegraphics[width=\textwidth]{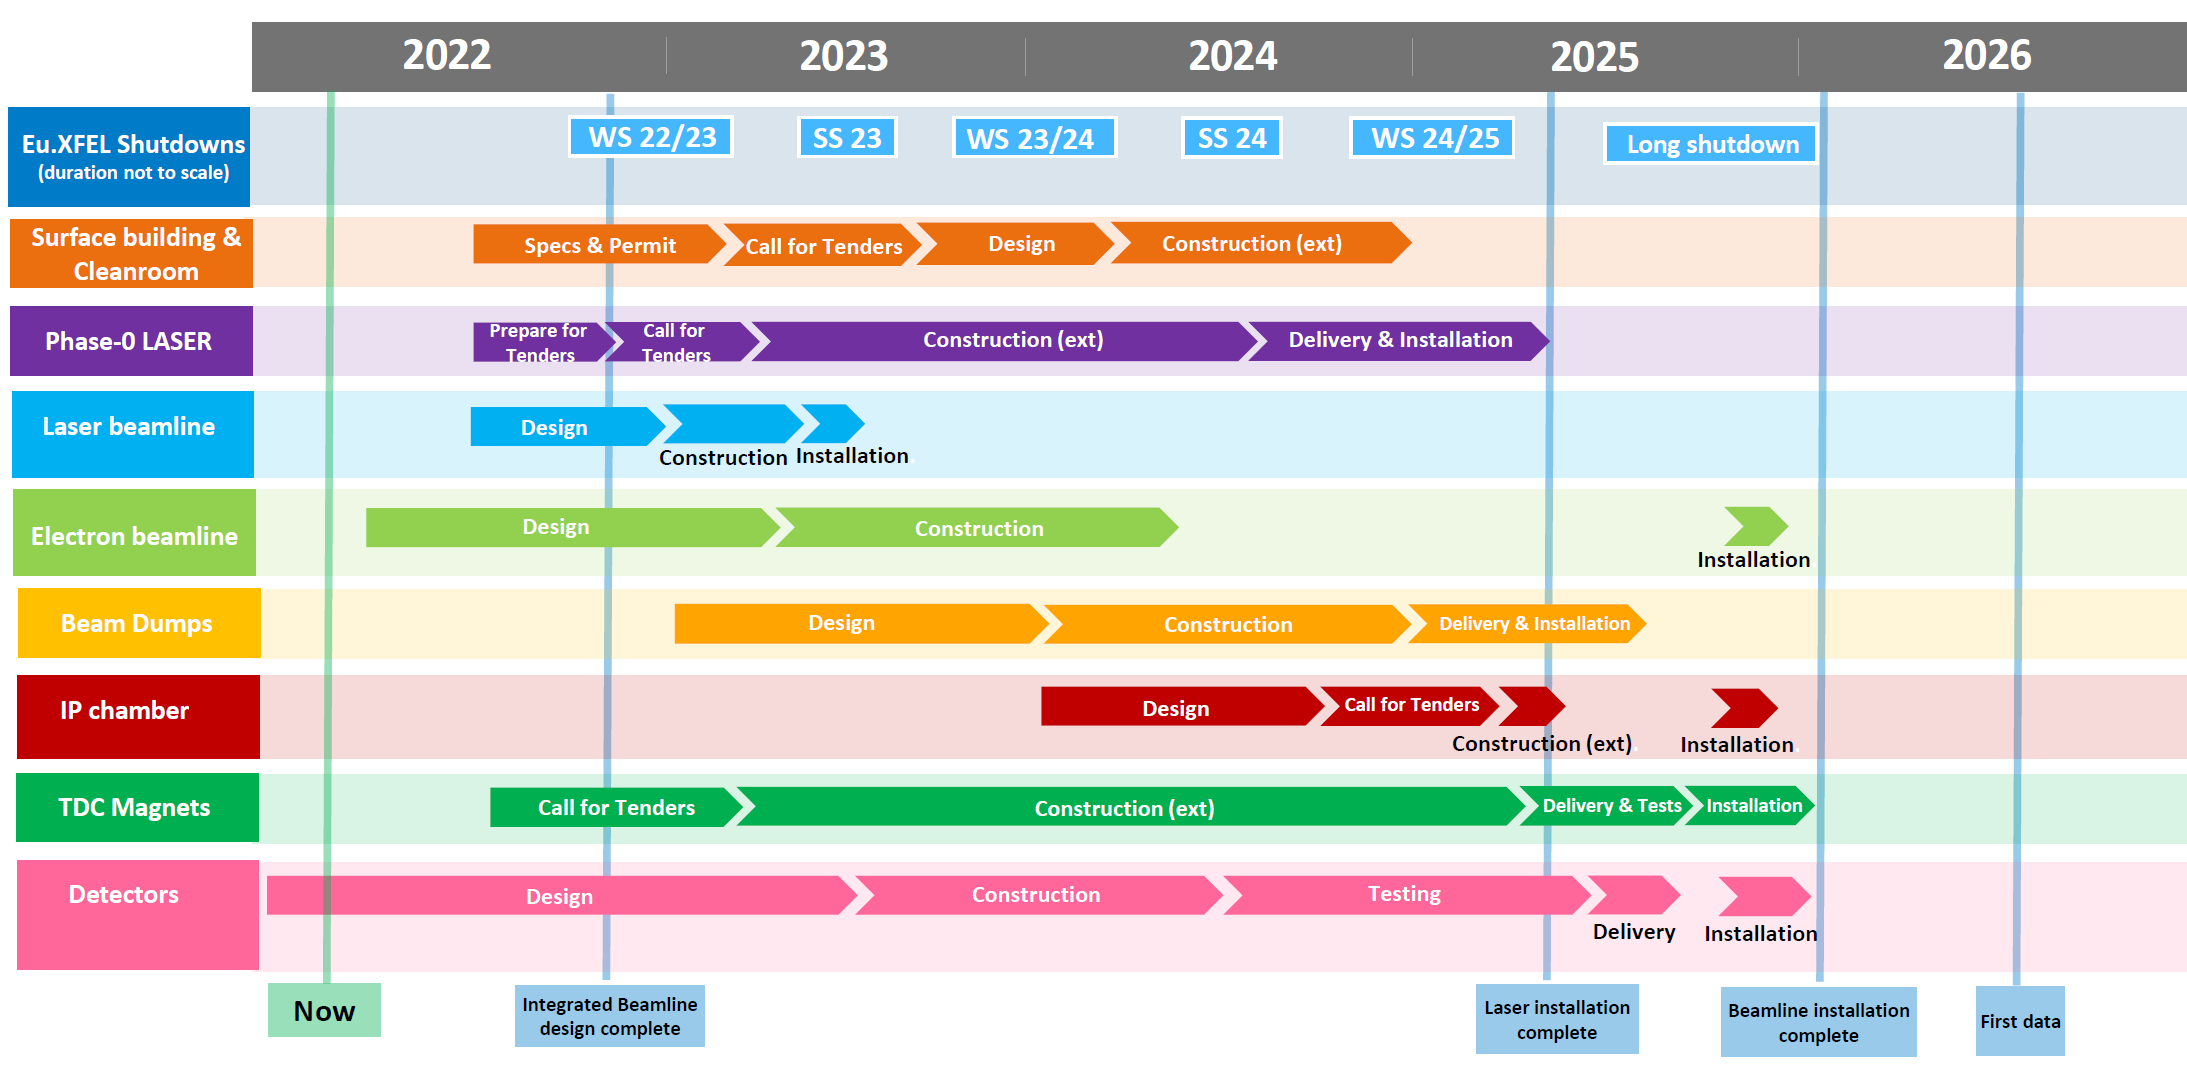}
    \caption{LUXE major items timeline.}
    \label{fig:majitemtimeline}
\end{figure}

\begin{figure}[htbp!]
\centering
\includegraphics[width=0.75\textwidth]{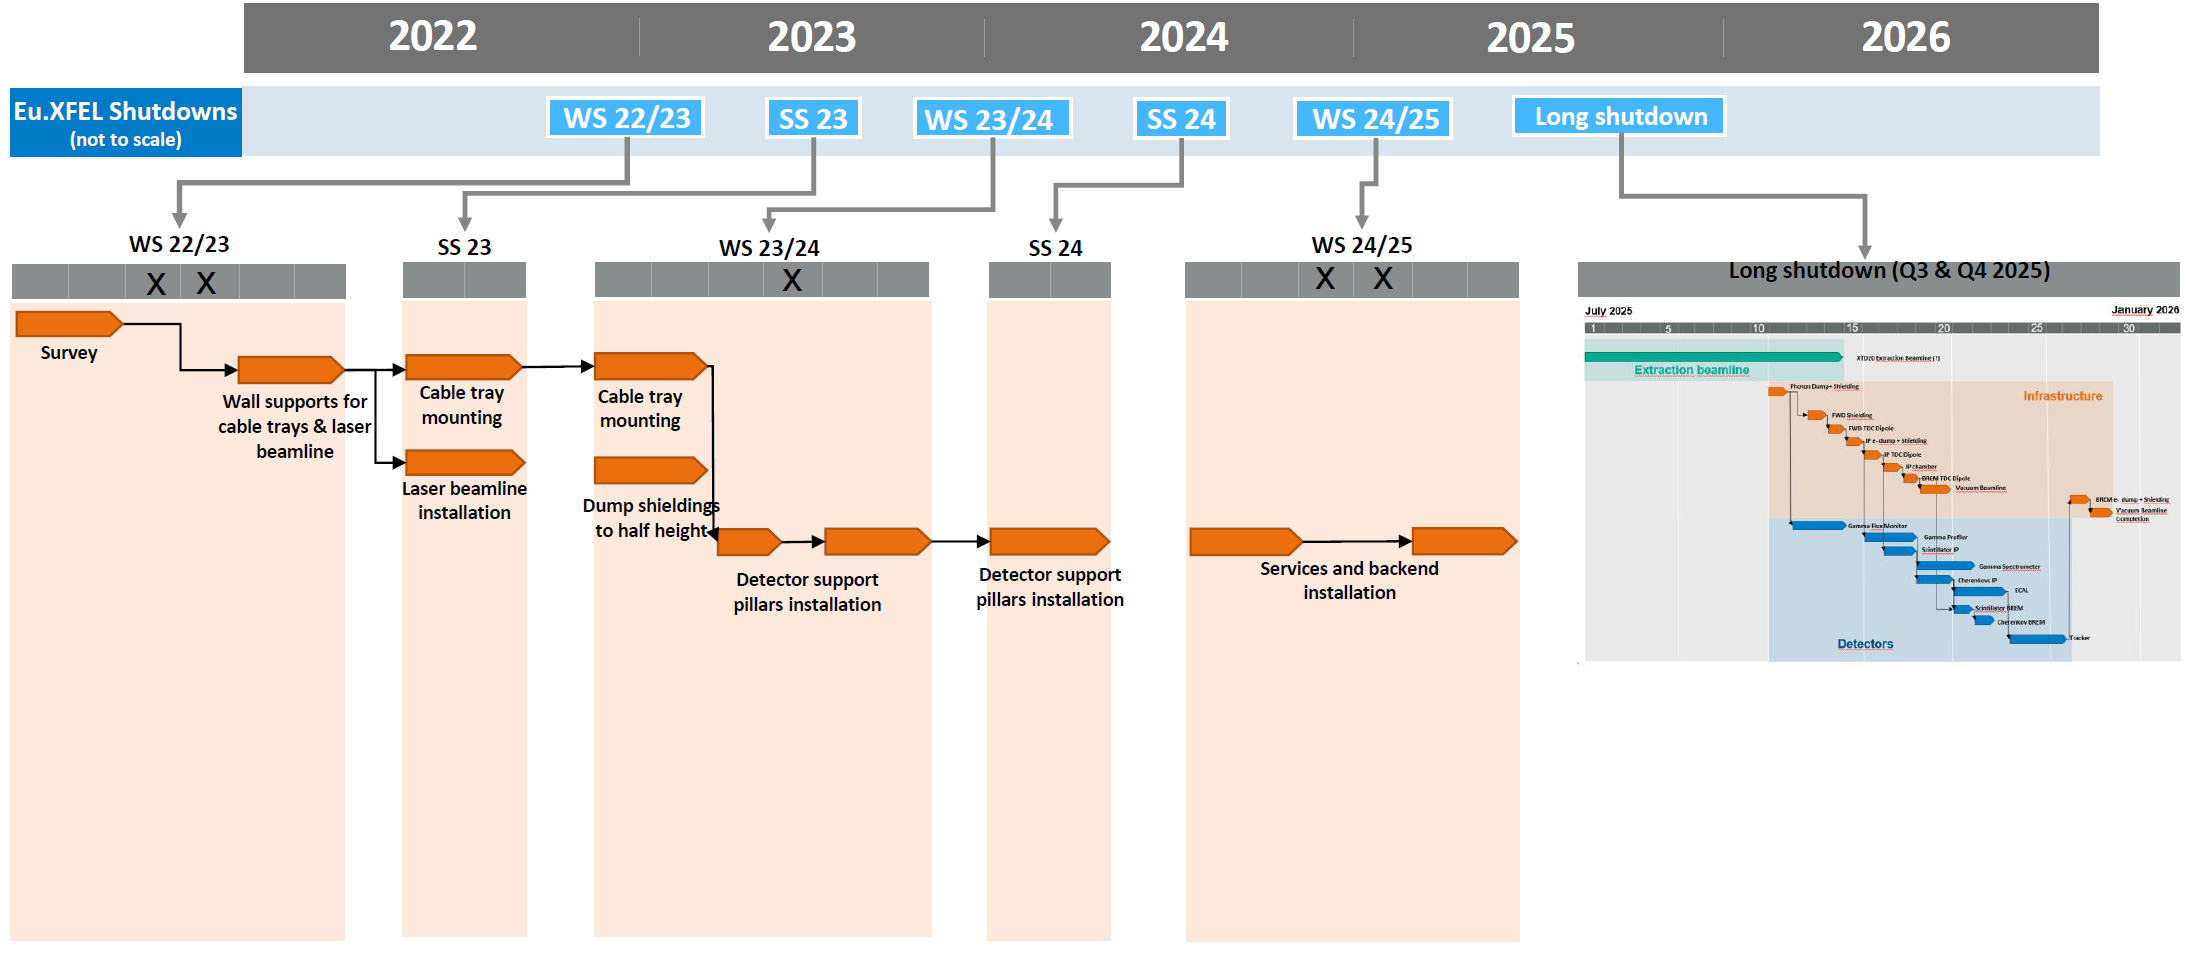}
\includegraphics[width=0.75\textwidth]{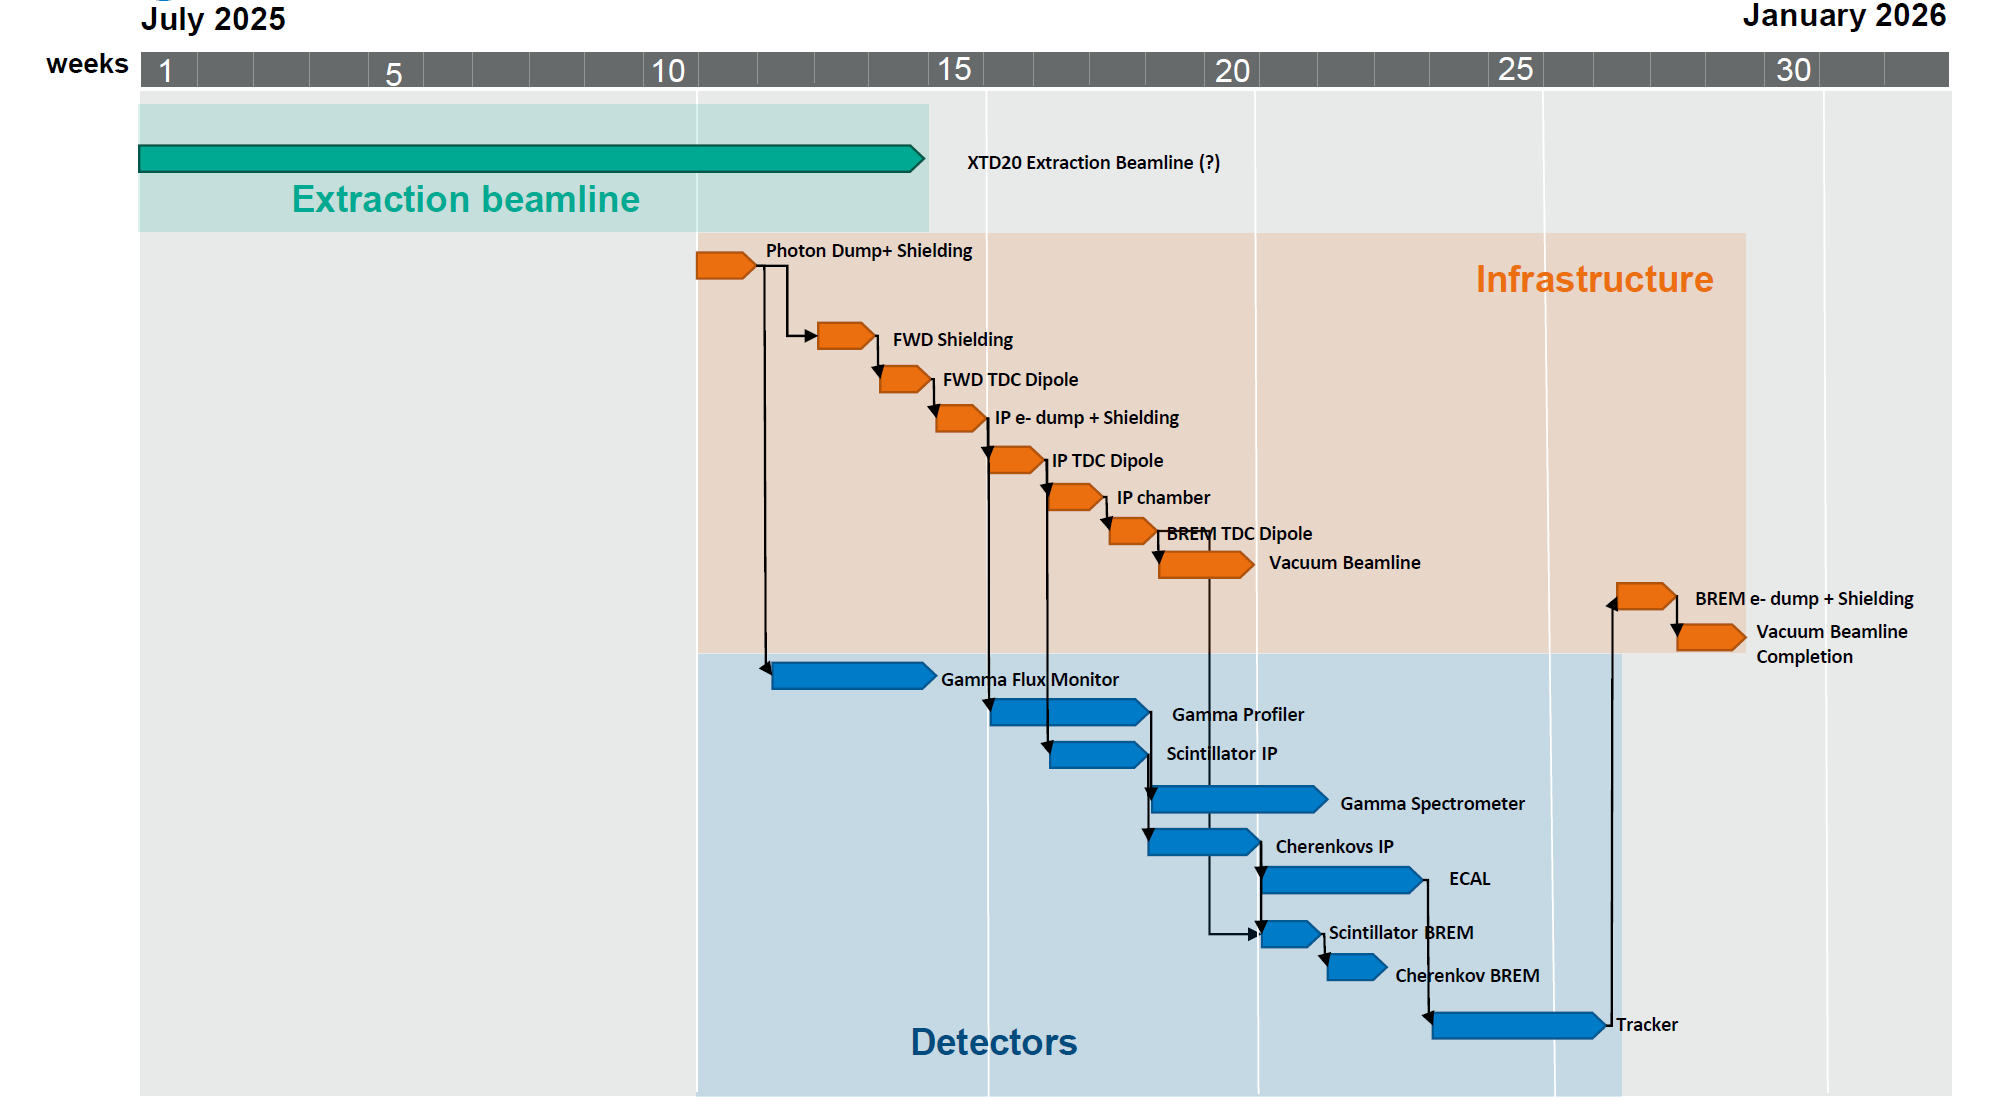} 
\caption{LUXE overall installation schedule (top). Detailed installation schedule in 2025 long shutdown (bottom).} 
\label{fig:luxeschedule} 
\end{figure}

The order of the installation works and duration of individual tasks as listed in section \ref{} and shown in fig.~\ref{fig:luxeschedule} has been discussed with the main contributing engineer of the LUXE project. The main boundary conditions to consider for the installation are the availability of space in the LUXE cavern, availability of transport such as forklift and crane, limited allowed number of workers, especially respecting parallel works on the XTD20 extraction beamline during the 2025 shutdown, as well as the ordering and manufacturing schedule of the long lead-time components in the beamline.

\begin{figure}
    \centering
    \includegraphics[width=\textwidth]{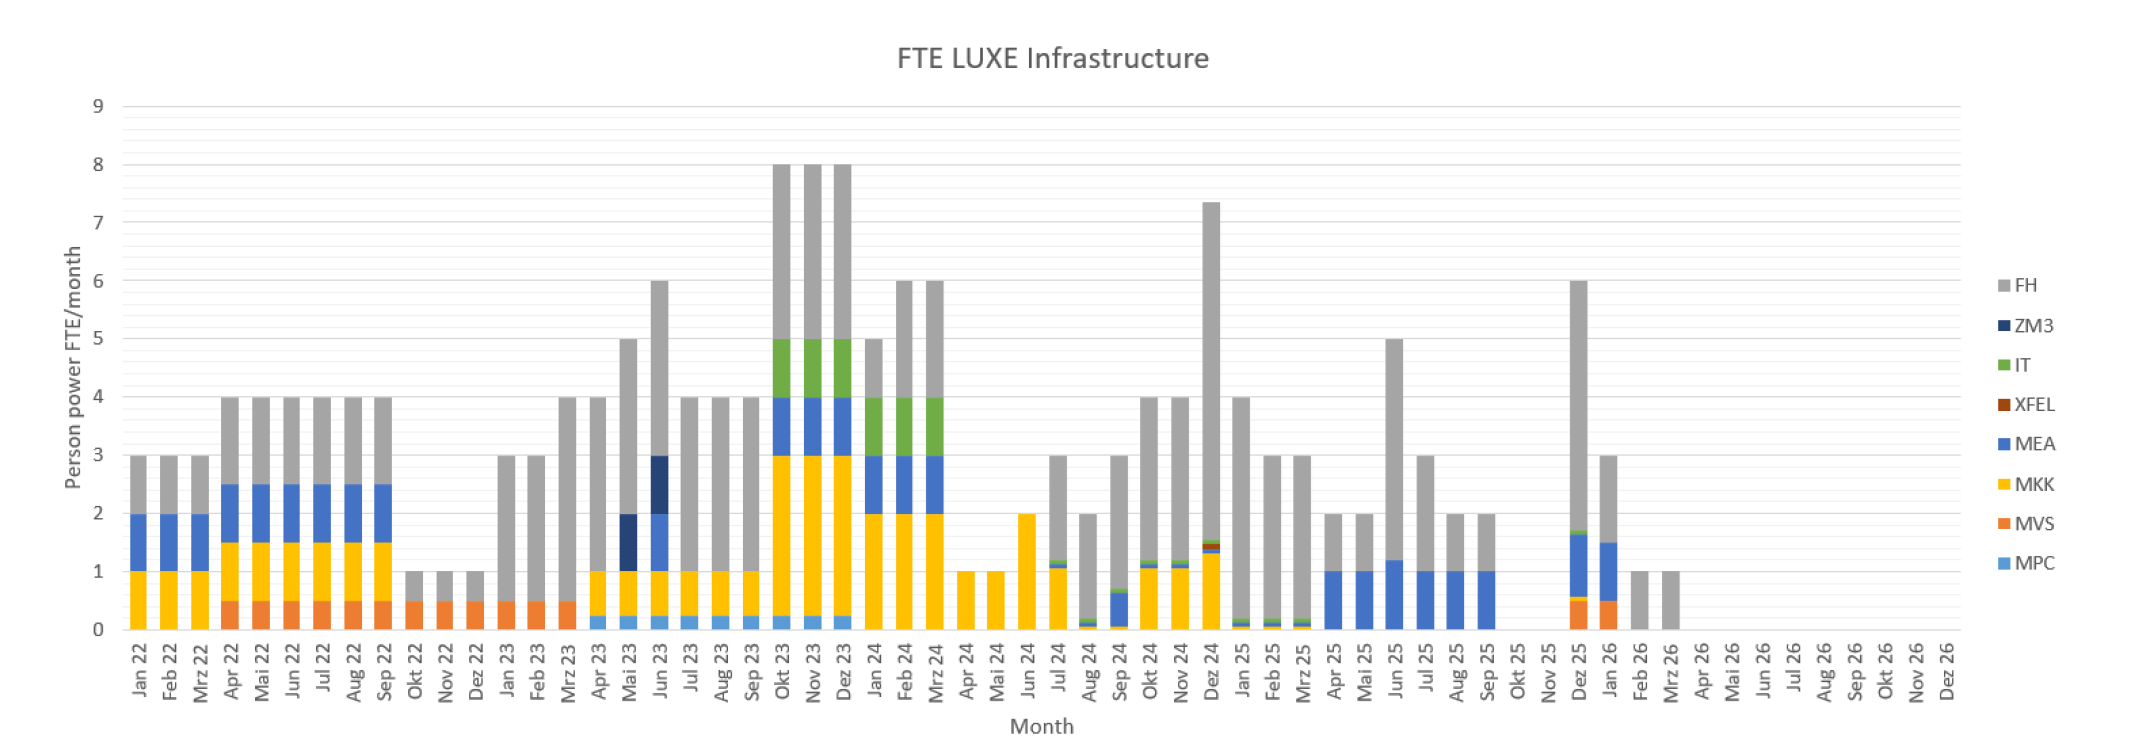}
    \caption{LUXE technical infrastructure FTE timeline by DESY technical groups.}
    \label{fig:luxeinfftemap}
\end{figure}

Fig.~\ref{fig:luxeinfftemap} shows the preliminary timeline of the DESY technical person-power needed for the design as well as the supervision of the manufacturing and installation of the LUXE technical infrastructure. The per-year FTE-need average is 2-3 FTE/year in FH and 1-2 FTE/year in the M-division, resulting in an integrated 8 FTE-years required in FH and 6 FTE-years in the M-division, in agreement with earlier estimates. The basis of estimate for this timeline is the list of tasks necessary to complete the infrastructure as shown in section~\ref{} \todo{refer to infrastructure section}. Each task is fractionally assigned to one or several DESY groups according to the expertise profile needed. The scenario assumed in the timeline shown is that any task which lies in the expertise of FH technical personnel is completed to a major fraction by the FH personnel and technical personnel of other DESY groups is only used where necessary. A preliminary estimate of the duration, FTE and group participation needed for the individual tasks were made in discussion with the main contributing LUXE engineer and received feedback by the technical note review panel, resulting in fig.~\ref{fig:luxeschedule}. It should be emphasized that further discussions with the relevant experts from the accelerator groups are required to arrive at a more granular and precise estimate.

\begin{figure}
    \centering
    \includegraphics[width=\textwidth]{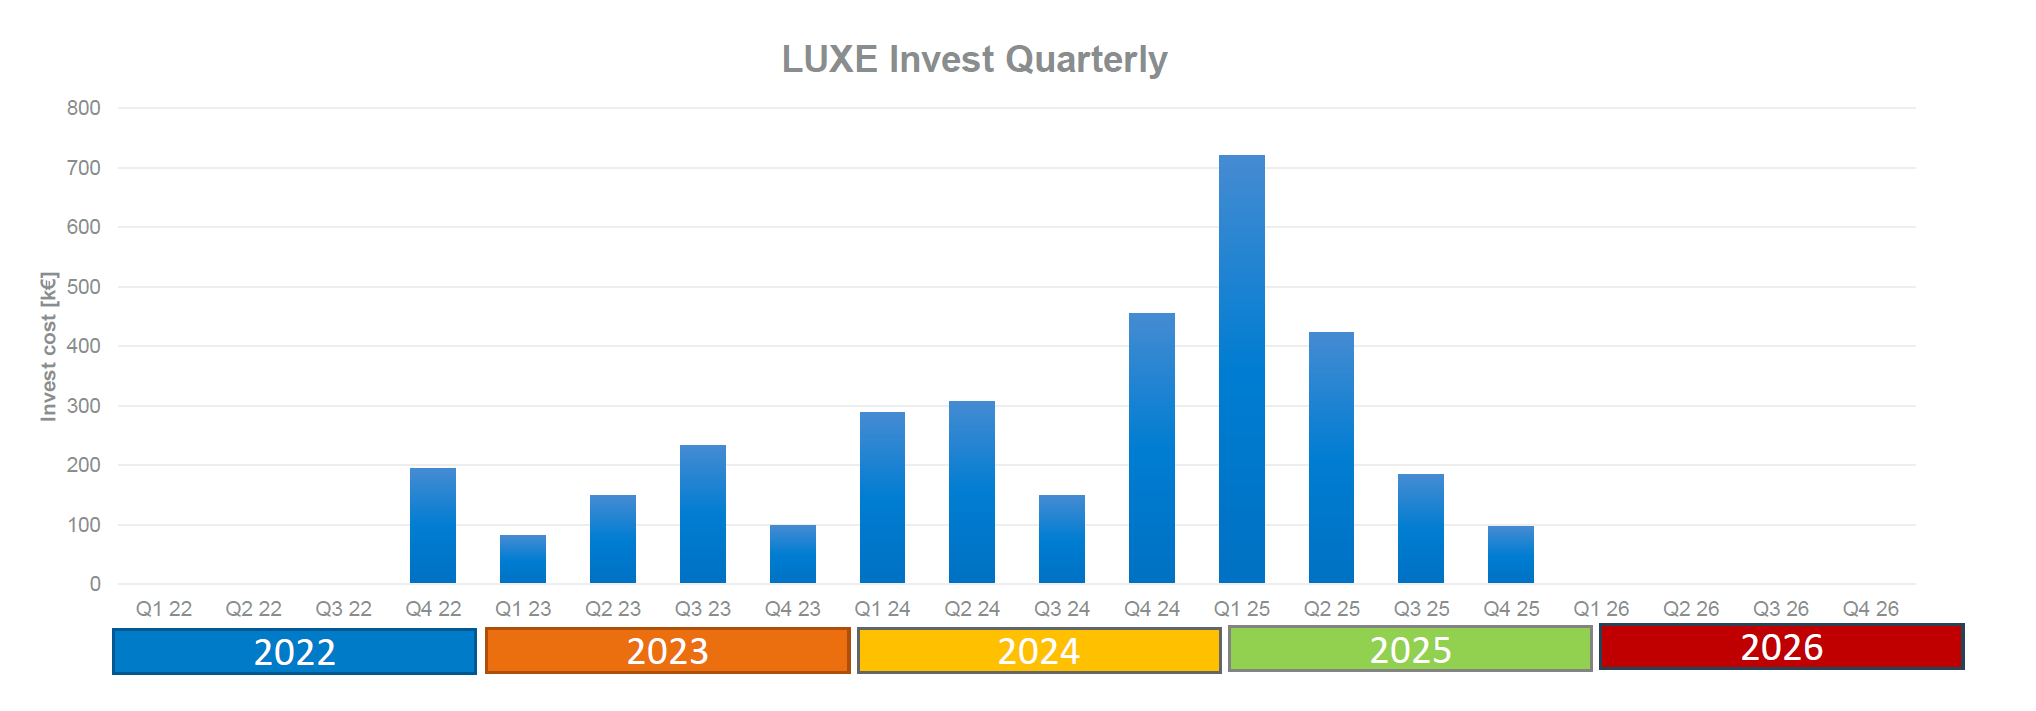}
    \caption{LUXE technical infrastructure spending profile.}
    \label{fig:luxeinfcostmap}
\end{figure}

Finally, fig.~\ref{fig:luxeinfcostmap} shows a preliminary estimate of the invest cost schedule for the LUXE technical infrastructure. The integrated cost corresponds to 3.5MEUR with a yearly average spending of 1MEUR.  The timeline shown is based on the list of items and cost from the technical infrastructure note tab.~\ref{} \todo{reference to infrastructure note}. The cost model is made such that one separate core invest and material cost (in MEUR) and person power (in FTE) that is assumed to come from local resources (i.e. DESY groups, M or FH). The core invest estimates are based on (preliminary) quotes from vendors or on experience from experts at DESY. The estimates of the personnel resources needed come from experts. Overheads, escalation or contingency are not included.

\section{Risk Estimate}

\section{Detector-specific estimates}
