# Supplementary material for: Technical Design Report for the LUXE Experiment
Source: arXiv:2308.00515 source file (2023-08-02)
Supplement: Supplementary file 10 [file appendix.tex]

\section{Changes with respect to the CDR Design}
